# Supplementary material for: Non-Coplanar Magnetic Orders in Classical Square-Kagome Antiferromagnets
Source: arXiv:2302.04171 ancillary file (2023-11-30)
Supplement: Supplementary file 1 [file Cuboc.pdf]

# Ground states of the phases I (cuboc) and II (cuboc-d), AFM square kagome, $J_1=J_2=J_3=1$

We want to show how to obtain deformed cuboctahedral ground states (phase II) by applying the generalized Luttinger-Tisza theory presented in: H.-J. Schmidt and J. Richter, Classical ground states of spin lattices, J. Phys. A: Math. Theor. **55**, 465005 (2022).

As a kind of preparation we first consider the simpler case of cuboctahedral ground states (phase I), although these ground states can also be obtained by elementary considerations.

---

## The case of cuboc ground states

The first task is to calculate the Fourier-transformed dressed J-matrix  $JJ \equiv J(q_1, q_2, \lambda)$ . We consider a primitive unit cell of the square kagome lattice and number its spin sites by 1, ..., 6 (see the light blue circles in the figure below). The couplings between these spins are directly inserted into  $JJ$ , for example, the coupling between “1” and “3” of strength  $J_2$  corresponds to the entry  $JJ(1,3)=JJ(3,1)=J_2$ .

The couplings between spins of the primitive unit cell and those of translated cells give rise to entries of  $JJ$  in the form of coupling constants multiplied by certain exponential factors. For example, the coupling between spin “1” and spin 5, shifted to the left and denoted by “5←”, corresponds to  $JJ(1,5)=J_2 \text{Exp}[-i q_1]=\overline{JJ(5,1)}$ . Similarly, the coupling between “4” and “6→↓” corresponds to the entry  $JJ(4,6)=J_x \text{Exp}[i(q_1 - q_2)]=\overline{JJ(6,4)}$ .

Out[•]=

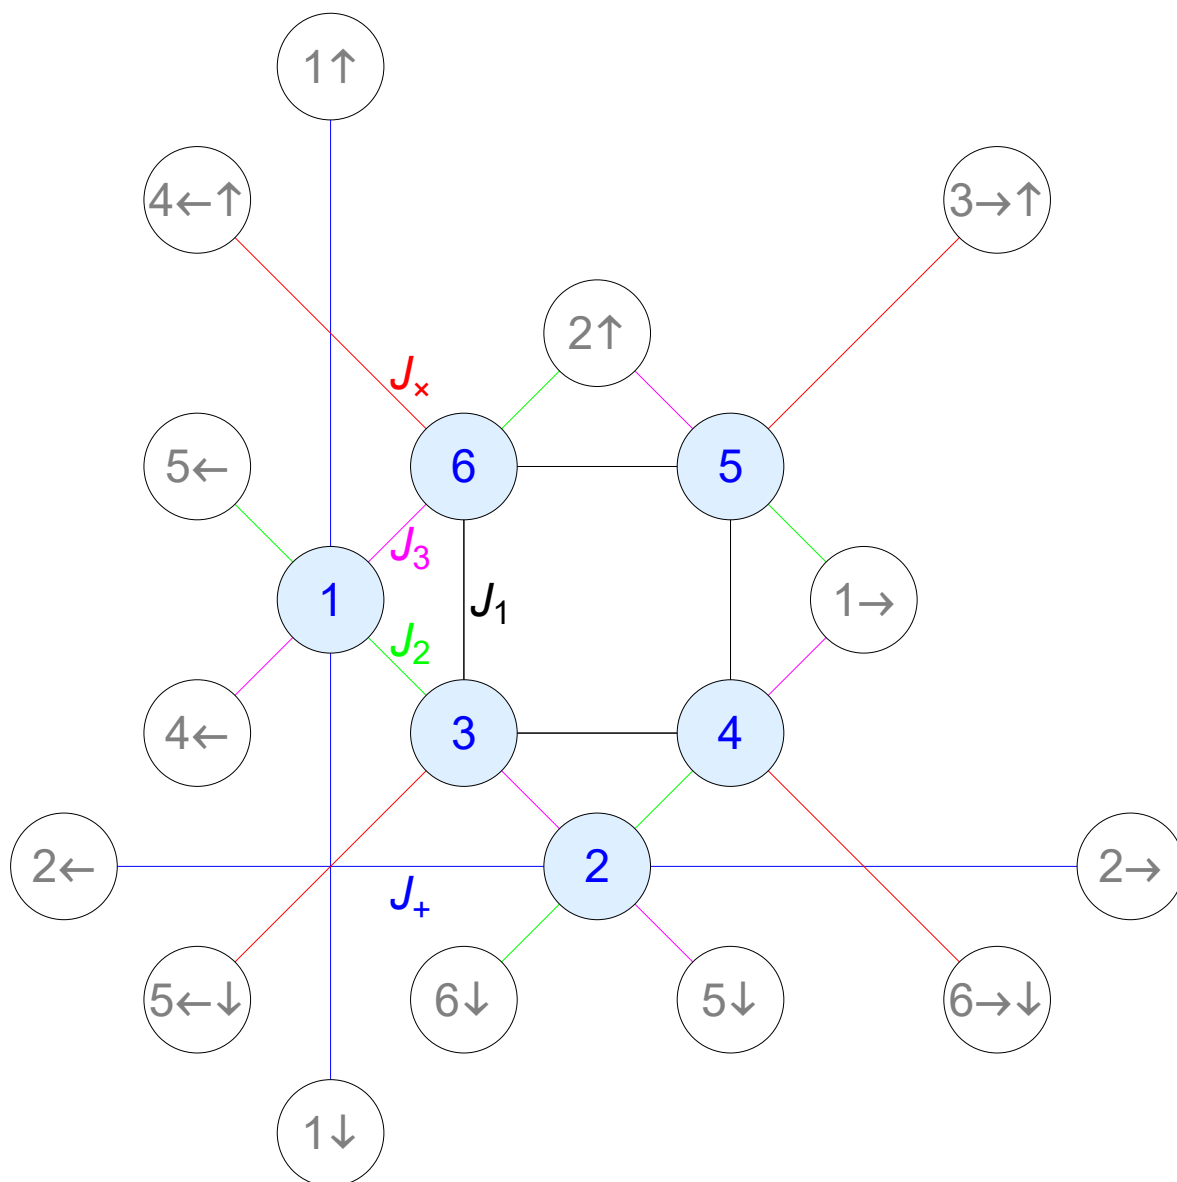

In this way we obtain the following J-matrix  $JJ \equiv J(q_1, q_2, \lambda)$ . Note, that we have not used subscripts and write “Jp” instead of  $J_+$ , and “Jc” instead of  $J_x$ . Moreover, we have introduced Lagrange parameters  $2\lambda$  and  $-\lambda$  in the diagonal of JJ that sum to zero and reflect the non-equivalence of the two groups of spin sites {1,2} and {3,4,5,6}.

```
In[1]:= JJ = Simplify[{ {2 Jp Cos[q2] + 2 λ, 0, J2, J3 Exp[-i q1], J2 Exp[-i q1], J3},
  {0, 2 Jp Cos[q1] + 2 λ, J3, J2, J3 Exp[-i q2], J2 Exp[-i q2]},
  {J2, J3, -λ, J1, Jc (Exp[-i (q1 + q2)]), J1},
  {J3 Exp[i q1], J2, J1, -λ, J1, Jc (Exp[i (q1 - q2)]), J1},
  {J2 Exp[i q1], J3 Exp[i q2], Jc (Exp[i (q1 + q2)]), J1, -λ, J1},
  {J3, J2 Exp[i q2], J1, Jc (Exp[i (q2 - q1)]), J1, -λ} }];
JJ // TableForm
```

Out[1]//TableForm=

|                              |                              |                         |                          |                          |                     |
|------------------------------|------------------------------|-------------------------|--------------------------|--------------------------|---------------------|
| $2(\lambda + J_p \cos[q_2])$ | 0                            | J2                      | $e^{-i q_1} J_3$         | $e^{-i q_1} J_2$         | J3                  |
| 0                            | $2(\lambda + J_p \cos[q_1])$ | J3                      | J2                       | $e^{-i q_2} J_3$         | $e^{-i q_2}$        |
| J2                           | J3                           | $-\lambda$              | J1                       | $e^{-i (q_1 + q_2)} J_c$ | J1                  |
| $e^{i q_1} J_3$              | J2                           | J1                      | $-\lambda$               | J1                       | $e^{i (q_1 - q_2)}$ |
| $e^{i q_1} J_2$              | $e^{i q_2} J_3$              | $e^{i (q_1 + q_2)} J_c$ | J1                       | $-\lambda$               | J1                  |
| J3                           | $e^{i q_2} J_2$              | J1                      | $e^{i (-q_1 + q_2)} J_c$ | J1                       | $-\lambda$          |

We specialize the J-matrix to the values  $\{J_1=1, J_2=1, J_3=1, J_p=1, J_c=1\}$ , and denote the special matrix by JB. It will serve as a mean to guess the correct choices for the general case.

```
In[2]:= special = {J1 → 1, J2 → 1, J3 → 1, Jp → 1, Jc → 1};
```

```
In[3]:= JB = Simplify[JJ /. special]; JB // TableForm
```

Out[3]//TableForm=

|                          |                          |                     |                      |                      |                     |
|--------------------------|--------------------------|---------------------|----------------------|----------------------|---------------------|
| $2(\lambda + \cos[q_2])$ | 0                        | 1                   | $e^{-i q_1}$         | $e^{-i q_1}$         | 1                   |
| 0                        | $2(\lambda + \cos[q_1])$ | 1                   | 1                    | $e^{-i q_2}$         | $e^{-i q_2}$        |
| 1                        | 1                        | $-\lambda$          | 1                    | $e^{-i (q_1 + q_2)}$ | 1                   |
| $e^{i q_1}$              | 1                        | 1                   | $-\lambda$           | 1                    | $e^{i (q_1 - q_2)}$ |
| $e^{i q_1}$              | $e^{i q_2}$              | $e^{i (q_1 + q_2)}$ | 1                    | $-\lambda$           | 1                   |
| 1                        | $e^{i q_2}$              | 1                   | $e^{i (-q_1 + q_2)}$ | 1                    | $-\lambda$          |

It has been remarked in the main text that the magnetic unit cell of the cuboc ground state has the size  $6 \times 2 \times 2 = 24$ . Hence it will suffice to consider the following q-vectors:

```
In[4]:= Q = {{0, 0}, {0, π}, {π, π}}
```

```
Out[4]= {{0, 0}, {0, π}, {π, π}}
```

The ground state Lagrange parameter  $\lambda$  can be obtained by the level

crossing of the minimal eigenvalues of JB. It has the value  $\hat{\lambda}=0.33333\dots$  and the corresponding energy per spin site  $2E_{\min}=-3.3333\dots$  (The factor 2 results from the usual convention of coupling counting.)

```
In[87]:= {ee, rule} = FindMaximum[
  Min[Table[Min[Eigenvalues[N[JB /. {q1 → Q[q, 1], q2 → Q[q, 2]]]], {q, Length[Q]}]],
  {λ, 0.35}]
```

```
Out[87]:= {-3.33333, {λ → 0.333333}}
```

```
In[88]:= Plot[Table[Eigenvalues[N[JB /. {q1 → Q[q, 1], q2 → Q[q, 2]]]], {q, Length[Q]}],
  {λ, 0, 1}, PlotRange → {-4, -3}, AxesOrigin → {0, -3.2}, AxesLabel → {"λ", "jmin"},
  LabelStyle → Directive[14, Gray], Epilog → {Red, Point[{rule[[1, 2]], ee}]}]
```

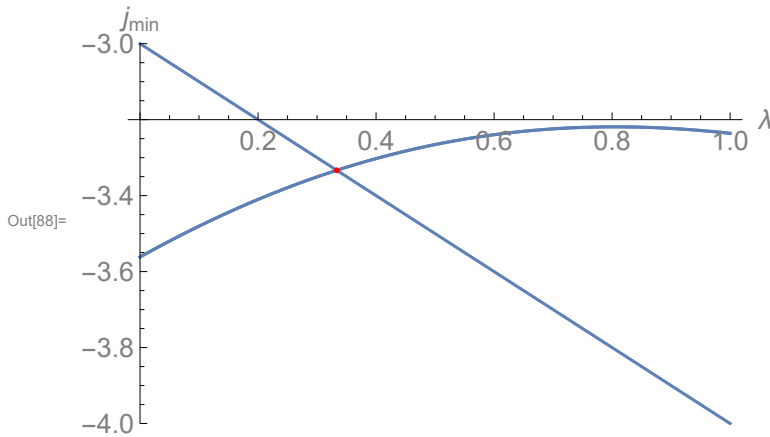

```
In[7]:= Table[{q, Min[Eigenvalues[N[JB /. {q1 → Q[q, 1], q2 → Q[q, 2]] /. rule]]}],
  {q, Length[Q]}]
```

```
Out[7]:= {{1, -1.33333}, {2, -3.33333}, {3, -3.33333}}
```

```
In[8]:= Q
```

```
Out[8]:= {{0, 0}, {0, π}, {π, π}}
```

It follows that the wave vectors  $\{0, \pi\}$  and  $\{\pi, \pi\}$  contribute to the ground state.

We identify the factor of the characteristic polynomial “pola” of  $JJ/. \{J1 \rightarrow 1, J2 \rightarrow 1, J3 \rightarrow 1\} /. \{q1 \rightarrow \pi, q2 \rightarrow \pi\}$  that leads to the eigenvalue of  $ee=-3.33333\dots$ . We note that this factor occurs squared.

```
In[9]:= pola = Factor[Simplify[
  CharacteristicPolynomial[JJ /. {J1 → 1, J2 → 1, J3 → 1} /. {q1 → π, q2 → π}, z]]]
```

```
Out[9]:= (-2 + Jc - z - λ) × (2 + Jc - z - λ) (-4 + 2 Jc Jp + Jc z + 2 Jp z + z^2 - 2 Jc λ + 2 Jp λ - z λ - 2 λ^2)^2
```

```
In[10]:= pola[[3, 1]]
```

```
Out[10]:= -4 + 2 Jc Jp + Jc z + 2 Jp z + z^2 - 2 Jc λ + 2 Jp λ - z λ - 2 λ^2
```

In[11]:= **solza = Solve[0 == pola[[3, 1]] /. special, z] [[1]]**

Out[11]=  $\left\{ z \rightarrow \frac{1}{2} \times \left( -3 + \lambda - \sqrt{17 - 6\lambda + 9\lambda^2} \right) \right\}$

In[12]:= **solza /. rule**

Out[12]=  $\{ z \rightarrow -3.33333 \}$

Analogously for  $\{q_1 \rightarrow 0, q_2 \rightarrow \pi\}$ :

In[13]:= **polb = Factor[Simplify[  
CharacteristicPolynomial[JJ /. {J1 → 1, J2 → 1, J3 → 1} /. {q1 → 0, q2 → π}, z]]]**

Out[13]=  $(Jc - z - \lambda) (2 + Jc + z + \lambda) \times$   
 $(-4 - 4Jp + 2JcJp - 2z + Jcz + 2Jpz + z^2 + 4\lambda - 2Jc\lambda + 2Jp\lambda - z\lambda - 2\lambda^2) \times$   
 $(4 - 2JcJp + Jcz + 2Jpz - z^2 - 2Jc\lambda + 2Jp\lambda + z\lambda + 2\lambda^2)$

In[14]:= **polb[[2]]**

Out[14]=  $2 + Jc + z + \lambda$

In[15]:= **solzb = Solve[0 == polb[[2]], z] [[1]]**

Out[15]=  $\{ z \rightarrow -2 - Jc - \lambda \}$

In[16]:= **solzb /. special /. rule**

Out[16]=  $\{ z \rightarrow -3.33333 \}$

The condition of level crossing leads to the general equations for the ground state Lagrange parameter  $\left\{ \lambda \rightarrow \frac{1}{3} (-Jc + 2Jp) \right\}$  and for the minimal energy per spin site  $E_{\min} = \frac{1}{3} \times (-3 - Jc - Jp)$ :

In[17]:= **crossing = Simplify[pola[[3, 1]] /. solzb]**

Out[17]=  $2 (Jc - 2Jp + 3\lambda)$

In[18]:= **soll = Solve[0 == crossing, λ] [[1]]**

Out[18]=  $\left\{ \lambda \rightarrow \frac{1}{3} (-Jc + 2Jp) \right\}$

In[19]:= **soll /. special**

Out[19]=  $\left\{ \lambda \rightarrow \frac{1}{3} \right\}$

In[20]:= **sollz = Simplify[solzb /. soll]**

Out[20]=  $\left\{ z \rightarrow -\frac{2}{3} \times (3 + Jc + Jp) \right\}$

In[21]:= **sollz /. special**

Out[21]=  $\left\{ z \rightarrow -\frac{10}{3} \right\}$

```
In[22]:= Emin = Simplify[1 / 2 sol1z[[1, 2]]]
```

```
Out[22]=  $\frac{1}{3} \times (-3 - Jc - Jp)$ 
```

To determine the ground state configuration we choose two suitable eigenvectors  $u, v$  of  $JJ$  corresponding to the wave vector  $\{\pi, \pi\}$  (recall that the corresponding eigenspace was twofold degenerate) and one eigenvector  $w$  corresponding to  $\{0, \pi\}$ :

```
In[23]:= esa = Eigensystem[JJ /. {J1 → 1, J2 → 1, J3 → 1} /. {q1 → π, q2 → π} /. sol1]
```

```
Out[23]=  $\left\{ \left\{ \frac{2}{3} \times (-3 + 2 Jc - Jp), \frac{2}{3} \times (3 + 2 Jc - Jp), -\frac{2}{3} \times (-3 + Jc + Jp), \right. \right.$   

 $\left. -\frac{2}{3} \times (-3 + Jc + Jp), -\frac{2}{3} \times (3 + Jc + Jp), -\frac{2}{3} \times (3 + Jc + Jp) \right\},$   

 $\{ \{0, 0, -1, 1, -1, 1\}, \{0, 0, 1, 1, 1, 1\}, \{1, -1, 0, -1, 0, 1\},$   

 $\{-1, -1, -1, 0, 1, 0\}, \{-1, 1, 0, -1, 0, 1\}, \{1, 1, -1, 0, 1, 0\} \}$ 
```

```
In[24]:= esa[[1]] /. special // N
```

```
Out[24]=  $\{-1.33333, 2.66667, 0.666667, 0.666667, -3.33333, -3.33333\}$ 
```

```
In[25]:= u = esa[[2, 5]]
```

```
Out[25]=  $\{-1, 1, 0, -1, 0, 1\}$ 
```

```
In[26]:= v = esa[[2, 6]]
```

```
Out[26]=  $\{1, 1, -1, 0, 1, 0\}$ 
```

```
In[27]:= esb = Eigensystem[JJ /. {J1 → 1, J2 → 1, J3 → 1} /. {q1 → 0, q2 → π} /. sol1];
```

```
In[28]:= esb[[1]] /. special // N
```

```
Out[28]=  $\{1.90273, 0.666667, -3.33333, -2.5694, -0.569401, 3.90273\}$ 
```

```
In[29]:= w = esb[[2, 3]]
```

```
Out[29]=  $\{0, 0, -1, 1, -1, 1\}$ 
```

Let  $W$  denote the matrix with columns  $u, v, w$ . It turns out that the six rows of  $W$  have already the same length. Upon multiplying with the global factor of  $1/\sqrt{2}$  they will become unit vectors and form a “rigid” 3-dimensional spin configuration (i.e., not depending on  $J_p$  and  $J_c$ ):

```
In[30]:= Wt = Simplify[ $\frac{1}{\sqrt{2}}$  {u, v, w}]; W = Transpose[Wt]; W // TableForm
```

Out[30]//TableForm=

$$\begin{array}{ccc} -\frac{1}{\sqrt{2}} & \frac{1}{\sqrt{2}} & 0 \\ \frac{1}{\sqrt{2}} & \frac{1}{\sqrt{2}} & 0 \\ 0 & -\frac{1}{\sqrt{2}} & -\frac{1}{\sqrt{2}} \\ -\frac{1}{\sqrt{2}} & 0 & \frac{1}{\sqrt{2}} \\ 0 & \frac{1}{\sqrt{2}} & -\frac{1}{\sqrt{2}} \\ \frac{1}{\sqrt{2}} & 0 & \frac{1}{\sqrt{2}} \end{array}$$

```
In[31]:= MatrixRank[W]
```

Out[31]= 3

We complete the set of these six spin vectors with their negative counterparts (which will be assumed in the other unit cells of the square Kagome lattice) and obtain a set S2 of 12 spins, pointing to the vertices of a cuboctahedron. This can be seen from their Gram matrix H2 (the matrix of all scalar products) and from a graphical representation:

```
In[32]:= S2 = Union[W, -W]; S2 // TableForm
```

```
Out[32]//TableForm=
```

|                       |                       |                       |
|-----------------------|-----------------------|-----------------------|
| 0                     | $-\frac{1}{\sqrt{2}}$ | $-\frac{1}{\sqrt{2}}$ |
| 0                     | $-\frac{1}{\sqrt{2}}$ | $\frac{1}{\sqrt{2}}$  |
| 0                     | $\frac{1}{\sqrt{2}}$  | $-\frac{1}{\sqrt{2}}$ |
| 0                     | $\frac{1}{\sqrt{2}}$  | $\frac{1}{\sqrt{2}}$  |
| $-\frac{1}{\sqrt{2}}$ | 0                     | $-\frac{1}{\sqrt{2}}$ |
| $-\frac{1}{\sqrt{2}}$ | 0                     | $\frac{1}{\sqrt{2}}$  |
| $-\frac{1}{\sqrt{2}}$ | $-\frac{1}{\sqrt{2}}$ | 0                     |
| $-\frac{1}{\sqrt{2}}$ | $\frac{1}{\sqrt{2}}$  | 0                     |
| $\frac{1}{\sqrt{2}}$  | 0                     | $-\frac{1}{\sqrt{2}}$ |
| $\frac{1}{\sqrt{2}}$  | 0                     | $\frac{1}{\sqrt{2}}$  |
| $\frac{1}{\sqrt{2}}$  | $-\frac{1}{\sqrt{2}}$ | 0                     |
| $\frac{1}{\sqrt{2}}$  | $\frac{1}{\sqrt{2}}$  | 0                     |

```
In[33]:= Length[S2]
```

```
Out[33]= 12
```

```
In[34]:= H2 = Table[S2[[i]].S2[[j]], {i, 12}, {j, 12}]; H2 // TableForm
```

```
Out[34]//TableForm=
```

|                |                |                |                |                |                |                |                |                |                |                |                |
|----------------|----------------|----------------|----------------|----------------|----------------|----------------|----------------|----------------|----------------|----------------|----------------|
| 1              | 0              | 0              | -1             | $\frac{1}{2}$  | $-\frac{1}{2}$ | $\frac{1}{2}$  | $-\frac{1}{2}$ | $\frac{1}{2}$  | $-\frac{1}{2}$ | $\frac{1}{2}$  | $-\frac{1}{2}$ |
| 0              | 1              | -1             | 0              | $-\frac{1}{2}$ | $\frac{1}{2}$  | $\frac{1}{2}$  | $-\frac{1}{2}$ | $-\frac{1}{2}$ | $\frac{1}{2}$  | $\frac{1}{2}$  | $-\frac{1}{2}$ |
| 0              | -1             | 1              | 0              | $\frac{1}{2}$  | $-\frac{1}{2}$ | $-\frac{1}{2}$ | $\frac{1}{2}$  | $\frac{1}{2}$  | $-\frac{1}{2}$ | $-\frac{1}{2}$ | $\frac{1}{2}$  |
| -1             | 0              | 0              | 1              | $-\frac{1}{2}$ | $\frac{1}{2}$  | $-\frac{1}{2}$ | $\frac{1}{2}$  | $-\frac{1}{2}$ | $\frac{1}{2}$  | $-\frac{1}{2}$ | $\frac{1}{2}$  |
| $\frac{1}{2}$  | $-\frac{1}{2}$ | $\frac{1}{2}$  | $-\frac{1}{2}$ | 1              | 0              | $\frac{1}{2}$  | $\frac{1}{2}$  | 0              | -1             | $-\frac{1}{2}$ | $-\frac{1}{2}$ |
| $-\frac{1}{2}$ | $\frac{1}{2}$  | $-\frac{1}{2}$ | $\frac{1}{2}$  | 0              | 1              | $\frac{1}{2}$  | $\frac{1}{2}$  | -1             | 0              | $-\frac{1}{2}$ | $-\frac{1}{2}$ |
| $\frac{1}{2}$  | $\frac{1}{2}$  | $-\frac{1}{2}$ | $-\frac{1}{2}$ | $\frac{1}{2}$  | $\frac{1}{2}$  | 1              | 0              | $-\frac{1}{2}$ | $-\frac{1}{2}$ | 0              | -1             |
| $-\frac{1}{2}$ | $-\frac{1}{2}$ | $\frac{1}{2}$  | $\frac{1}{2}$  | $\frac{1}{2}$  | $\frac{1}{2}$  | 0              | 1              | $-\frac{1}{2}$ | $-\frac{1}{2}$ | -1             | 0              |
| $\frac{1}{2}$  | $-\frac{1}{2}$ | $\frac{1}{2}$  | $-\frac{1}{2}$ | 0              | -1             | $-\frac{1}{2}$ | $-\frac{1}{2}$ | 1              | 0              | $\frac{1}{2}$  | $\frac{1}{2}$  |
| $-\frac{1}{2}$ | $\frac{1}{2}$  | $-\frac{1}{2}$ | $\frac{1}{2}$  | -1             | 0              | $-\frac{1}{2}$ | $-\frac{1}{2}$ | 0              | 1              | $\frac{1}{2}$  | $\frac{1}{2}$  |
| $\frac{1}{2}$  | $\frac{1}{2}$  | $-\frac{1}{2}$ | $-\frac{1}{2}$ | $-\frac{1}{2}$ | $-\frac{1}{2}$ | 0              | -1             | $\frac{1}{2}$  | $\frac{1}{2}$  | 1              | 0              |
| $-\frac{1}{2}$ | $-\frac{1}{2}$ | $\frac{1}{2}$  | $\frac{1}{2}$  | $-\frac{1}{2}$ | $-\frac{1}{2}$ | -1             | 0              | $\frac{1}{2}$  | $\frac{1}{2}$  | 0              | 1              |



```

In[35]:= pairs = Flatten[Table[{i, j}, {i, 12}, {j, i + 1, 12}], 1];
In[36]:= ED2 = Select[pairs, 0 < H2[[#1]], #2] < 0.7 &];
In[37]:= Graphics3D[Join[{Opacity[0.2], Sphere[]},
  Table[{PointSize[0.02], Opacity[1], Point[S2[[μ]]}, {μ, 12}],
  Table[{Text[Style[μ, 14, Opacity[1], Red], 1.1 S2[[μ]]}, {μ, 12}],
  Table[{Blue, Opacity[1], Line[{S2[[ED2[[k, 1]]], S2[[ED2[[k, 2]]]]},
    {k, Length[ED2] }]], Boxed → False]

```

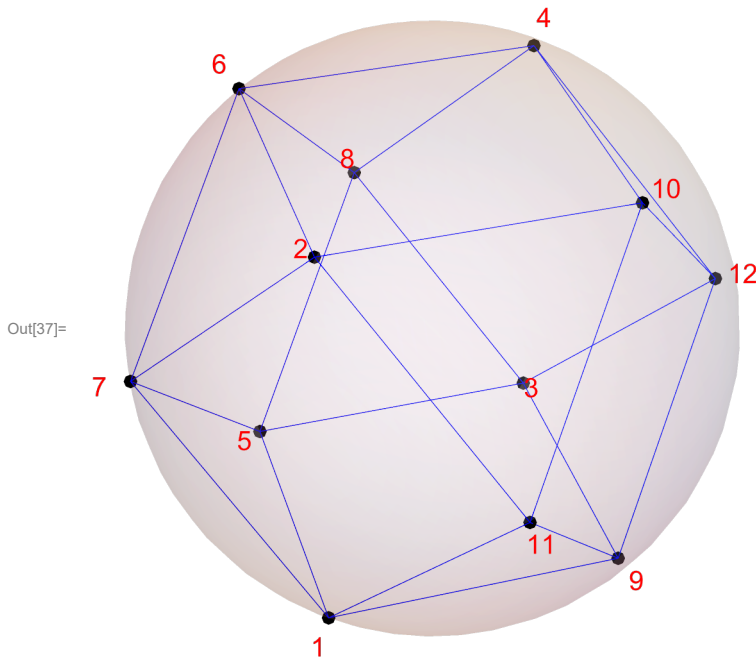

## The case of deformed cuboc ground states

We need not repeat that part of the reasoning, which is entirely analogous to the cuboc case, and focus on the differences.

We specialize the J-matrix to the values  $\{J_1=1, J_2=1, J_3=1, J_p=1, J_c=-1/100\}$ , and denote the special matrix by JA. It will serve as a mean to guess the correct choices for the general case.

```

In[38]:= deformed = {J1 → 1, J2 → 1, J3 → 1, Jp → 1, Jc → -1 / 100};

```

```
In[39]:= JA = Simplify[JJ /. deformed]; JA // TableForm
```

```
Out[39]//TableForm=
```

|                          |                          |                                 |                                  |                                  |                  |
|--------------------------|--------------------------|---------------------------------|----------------------------------|----------------------------------|------------------|
| $2(\lambda + \cos[q_2])$ | 0                        | 1                               | $e^{-iq_1}$                      | $e^{-iq_1}$                      | 1                |
| 0                        | $2(\lambda + \cos[q_1])$ | 1                               | 1                                | $e^{-iq_2}$                      | $e^{-iq_2}$      |
| 1                        | 1                        | $-\lambda$                      | 1                                | $-\frac{1}{100} e^{-i(q_1+q_2)}$ | 1                |
| $e^{iq_1}$               | 1                        | 1                               | $-\lambda$                       | 1                                | $-\frac{1}{100}$ |
| $e^{iq_1}$               | $e^{iq_2}$               | $-\frac{1}{100} e^{i(q_1+q_2)}$ | 1                                | $-\lambda$                       | 1                |
| 1                        | $e^{iq_2}$               | 1                               | $-\frac{1}{100} e^{i(-q_1+q_2)}$ | 1                                | $-\lambda$       |

The ground state Lagrange parameter  $\hat{\lambda}$  can be obtained by the level crossing of the minimal eigenvalues of JA. It has the value  $\hat{\lambda}=0.656733...$  and the corresponding energy per spin site  $2E_{\min}=-2.66673...$  (Note that there might occur small deviations from these values depending on the computer system):

```
In[41]:= {ee, rule} = FindMaximum[
  Min[Table[Min[Eigenvalues[N[JA /. {q1 -> Q[q, 1], q2 -> Q[q, 2]]]], {q, Length[Q]}]],
  {λ, 0.65}]
```

```
Out[41]= {-2.66673, {λ -> 0.656733}}
```

```
In[42]:= Plot[Table[Eigenvalues[N[JA /. {q1 -> Q[q, 1], q2 -> Q[q, 2]]]], {q, Length[Q]}],
  {λ, 0, 1}, PlotRange -> {-3.0, -2.6}, AxesOrigin -> {0, -2.7}, AxesLabel -> {"λ", "j_min"},
  LabelStyle -> Directive[14, Gray], Epilog -> {Red, Point[{rule[[1, 2]], ee}]}
```

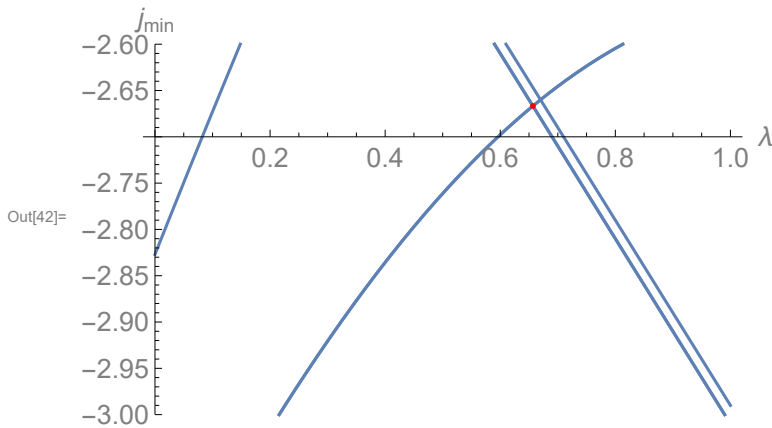

```
In[43]:= Table[{q, Min[Eigenvalues[N[JA /. {q1 -> Q[q, 1], q2 -> Q[q, 2]] /. rule]]},
  {q, Length[Q]}]
```

```
Out[43]= {{1, -2.66673}, {2, -2.64673}, {3, -2.66673}}
```

```
In[44]:= Q
```

```
Out[44]= {{0, 0}, {0, π}, {π, π}}
```

The difference to the cuboc case is that now the wave-vectors  $\{0,0\}$  and  $\{\pi,\pi\}$  contribute to the ground state. The condition of level crossing again leads to

the ground state Lagrange parameter  $\left\{ \lambda \rightarrow \frac{Jc^2 - 2 Jp + Jc (-3 + 2 Jp)}{3 \times (-1 + Jc)} \right\}$   
 and the minimal energy per site  $E_{\min} = \frac{3 + Jc^2 + Jp - Jc (3 + Jp)}{3 \times (-1 + Jc)} :$

```
In[45]:= polc = Factor[Simplify[
  CharacteristicPolynomial[JJ /. {J1 -> 1, J2 -> 1, J3 -> 1} /. {q1 -> 0, q2 -> 0}, z]]]
```

```
Out[45]= (-2 Jp + z - 2 λ) × (-2 + Jc - z - λ) (Jc + z + λ)2
  (8 - 4 Jp - 2 Jc Jp + 2 z + Jc z + 2 Jp z - z2 - 4 λ - 2 Jc λ + 2 Jp λ + z λ + 2 λ2)
```

```
In[46]:= polc[[2]]
```

```
Out[46]= -2 + Jc - z - λ
```

```
In[47]:= solzc = Solve[0 == polc[[2]], z][[1]]
```

```
Out[47]= {z -> -2 + Jc - λ}
```

```
In[48]:= solzc /. deformed /. rule
ee
```

```
Out[48]= {z -> -2.66673}
```

```
Out[49]= -2.66673
```

```
In[50]:= pola[[3, 1]]
```

```
Out[50]= -4 + 2 Jc Jp + Jc z + 2 Jp z + z2 - 2 Jc λ + 2 Jp λ - z λ - 2 λ2
```

```
In[51]:= solza = Solve[0 == pola[[3, 1]], z][[1]]
```

```
Out[51]= {z -> 1/2 (-Jc - 2 Jp + λ - sqrt(16 + Jc2 - 4 Jc Jp + 4 Jp2 + 6 Jc λ - 12 Jp λ + 9 λ2))}
```

```
In[52]:= solza /. deformed /. rule
ee
```

```
Out[52]= {z -> -2.66673}
```

```
Out[53]= -2.66673
```

```
In[54]:= crossing = Simplify[pola[[3, 1]] /. solzc]
```

```
Out[54]= 2 (Jc2 - 2 Jp + 2 Jc Jp + 3 λ - 3 Jc (1 + λ))
```

```
In[55]:= soll = Simplify[Solve[0 == crossing, λ][[1]]]
```

```
Out[55]= {λ -> (Jc2 - 2 Jp + Jc (-3 + 2 Jp)) / (3 × (-1 + Jc))}
```

```
In[56]:= soll /. deformed // N
rule
```

```
Out[56]= {λ -> 0.656733}
```

```
Out[57]= {λ -> 0.656733}
```

```
In[58]:= Emin =  $\frac{1}{2}$  (Simplify[solzc /. sol1]) [[1, 2]]
```

```
Out[58]= 
$$\frac{3 + \mathcal{J}c^2 + \mathcal{J}p - \mathcal{J}c (3 + \mathcal{J}p)}{3 \times (-1 + \mathcal{J}c)}$$

```

However, it turns out that, for the obtained ground state Lagrange parameter, the minimal eigenvalue of  $\mathcal{J}\mathcal{J}/\{q_1 \rightarrow \pi, q_2 \rightarrow \pi\}$  is 3-fold degenerate and its eigenvectors suffice to construct a ground state:

```
In[59]:= esa = Eigensystem[ $\mathcal{J}\mathcal{J}$  /. { $\mathcal{J}1 \rightarrow 1$ ,  $\mathcal{J}2 \rightarrow 1$ ,  $\mathcal{J}3 \rightarrow 1$ } /. { $q1 \rightarrow \pi$ ,  $q2 \rightarrow \pi$ } /. sol1]
```

```
Out[59]= 
$$\left\{ \left\{ \frac{2 \times (3 - 3 \mathcal{J}c + \mathcal{J}c^2 + \mathcal{J}p - \mathcal{J}c \mathcal{J}p)}{3 \times (-1 + \mathcal{J}c)}, \frac{2 \times (3 - 3 \mathcal{J}c + \mathcal{J}c^2 + \mathcal{J}p - \mathcal{J}c \mathcal{J}p)}{3 \times (-1 + \mathcal{J}c)}, \right. \right.$$


$$\frac{2 \times (3 - 3 \mathcal{J}c + \mathcal{J}c^2 + \mathcal{J}p - \mathcal{J}c \mathcal{J}p)}{3 \times (-1 + \mathcal{J}c)}, \frac{2 \times (-3 + 3 \mathcal{J}c + \mathcal{J}c^2 + \mathcal{J}p - \mathcal{J}c \mathcal{J}p)}{3 \times (-1 + \mathcal{J}c)},$$


$$\left. - \frac{2 \times (3 - 3 \mathcal{J}c + 2 \mathcal{J}c^2 - \mathcal{J}p + \mathcal{J}c \mathcal{J}p)}{3 \times (-1 + \mathcal{J}c)}, - \frac{2 \times (3 - 3 \mathcal{J}c + 2 \mathcal{J}c^2 - \mathcal{J}p + \mathcal{J}c \mathcal{J}p)}{3 \times (-1 + \mathcal{J}c)} \right\},$$


$$\left\{ \{0, 1 - \mathcal{J}c, -1, 0, 0, 1\}, \{1 - \mathcal{J}c, 1 - \mathcal{J}c, -1, 0, 1, 0\}, \{1 - \mathcal{J}c, 0, -1, 1, 0, 0\}, \right.$$


$$\left. \{0, 0, 1, 1, 1, 1\}, \left\{ -\frac{1}{-1 + \mathcal{J}c}, \frac{1}{-1 + \mathcal{J}c}, 0, -1, 0, 1 \right\}, \left\{ -\frac{1}{1 - \mathcal{J}c}, -\frac{1}{1 - \mathcal{J}c}, -1, 0, 1, 0 \right\} \right\}$$

```

```
In[60]:= esa[[1]] /. deformed // N
```

```
Out[60]= {-2.66673, -2.66673, -2.66673, 1.33327, 1.33347, 1.33347}
```

```
In[61]:= u = esa[[2, 1]]
```

```
Out[61]= {0, 1 -  $\mathcal{J}c$ , -1, 0, 0, 1}
```

```
In[62]:= v = esa[[2, 2]]
```

```
Out[62]= {1 -  $\mathcal{J}c$ , 1 -  $\mathcal{J}c$ , -1, 0, 1, 0}
```

```
In[63]:= w = esa[[2, 3]]
```

```
Out[63]= {1 -  $\mathcal{J}c$ , 0, -1, 1, 0, 0}
```

```
In[64]:= Wt = Chop[{u, v, w}]; W = Transpose[Wt]; W // TableForm
```

```
Out[64]//TableForm=
```

|                    |                    |                    |
|--------------------|--------------------|--------------------|
| 0                  | 1 - $\mathcal{J}c$ | 1 - $\mathcal{J}c$ |
| 1 - $\mathcal{J}c$ | 1 - $\mathcal{J}c$ | 0                  |
| -1                 | -1                 | -1                 |
| 0                  | 0                  | 1                  |
| 0                  | 1                  | 0                  |
| 1                  | 0                  | 0                  |

```
In[65]:= MatrixRank[W]
```

```
Out[65]= 3
```

In this case we have to consider a  $3 \times 3$ -matrix of coefficients  $\Gamma$  such that  $S=W\Gamma$  will be the ground state configuration. It follows that the diagonal

elements of the Gram matrix  $G = S S^T = W \Gamma \Gamma^T W^T \equiv W \Delta W^T$  should have the value 1. The latter condition yields  $\Delta$ :

```
In[66]:= Δ = Table[If[i < j, δ[i, j], δ[j, i]], {i, 3}, {j, 3}];
VAR = Union[Flatten[Δ]]
```

```
Out[66]= {δ[1, 1], δ[1, 2], δ[1, 3], δ[2, 2], δ[2, 3], δ[3, 3]}
```

```
In[67]:= G = W.Δ.Wt;
```

```
In[68]:= sold = Solve[Table[G[[i, i]] == 1, {i, 6}], VAR][[1]]
```

```
Out[68]= {δ[1, 1] → 1, δ[1, 2] → - $\frac{1-4Jc+2Jc^2}{2(-1+Jc)^2}$ , δ[1, 3] → - $\frac{2Jc-Jc^2}{(-1+Jc)^2}$ ,
δ[2, 2] → 1, δ[2, 3] → - $\frac{1-4Jc+2Jc^2}{2(-1+Jc)^2}$ , δ[3, 3] → 1}
```

```
In[69]:= Δ1 = Δ /. sold; Δ1 // TableForm
```

```
Out[69]//TableForm=
```

$$\begin{array}{ccc} 1 & -\frac{1-4Jc+2Jc^2}{2(-1+Jc)^2} & -\frac{2Jc-Jc^2}{(-1+Jc)^2} \\ -\frac{1-4Jc+2Jc^2}{2(-1+Jc)^2} & 1 & -\frac{1-4Jc+2Jc^2}{2(-1+Jc)^2} \\ -\frac{2Jc-Jc^2}{(-1+Jc)^2} & -\frac{1-4Jc+2Jc^2}{2(-1+Jc)^2} & 1 \end{array}$$

However, we must ensure that  $\Delta \equiv \Gamma \Gamma^T$  will be positively semi-definite:

```
In[70]:= evd = Eigenvalues[Δ1]
```

```
Out[70]= { $\frac{1}{(-1+Jc)^2}$ ,  $\frac{2-6Jc+3Jc^2-\sqrt{2-16Jc+44Jc^2-36Jc^3+9Jc^4}}{2(-1+Jc)^2}$ ,
 $\frac{2-6Jc+3Jc^2+\sqrt{2-16Jc+44Jc^2-36Jc^3+9Jc^4}}{2(-1+Jc)^2}$ }
```

```
In[71]:= soljc = Solve[0 == 2-6Jc+3Jc^2- $\sqrt{2-16Jc+44Jc^2-36Jc^3+9Jc^4}$ , Jc]
```

```
Out[71]= {{Jc →  $\frac{1}{2} \times (2-\sqrt{2})$ }, {Jc →  $\frac{1}{2} \times (2+\sqrt{2})$ }}
```

```
In[72]:= soljc // N
```

```
Out[72]= {{Jc → 0.292893}, {Jc → 1.70711}}
```

```
In[73]:= Plot[Evaluate[evd /. Jc -> x], {x, -1,  $\frac{1}{2} \times (2 - \sqrt{2})$ }]
```

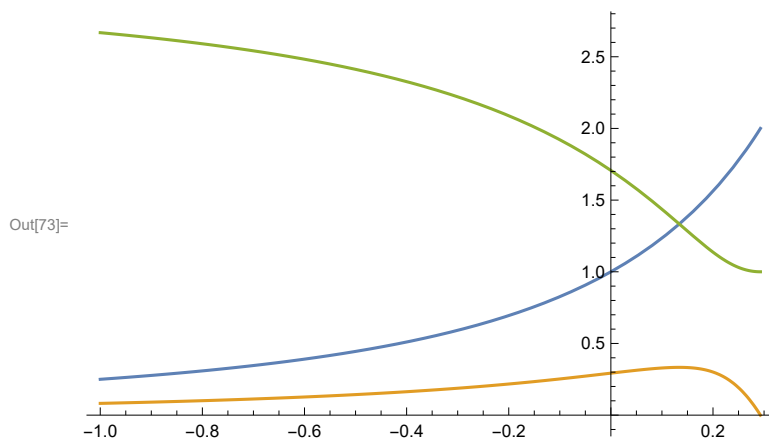

Recall that the deformed cuboc state is expected to live in the quadrant  $J_p > 0$ ,  $J_c < 0$ , and hence  $\Delta > 0$  will hold there. The Gram matrix  $G$  assumes the form  $G_1$ :

```
In[74]:= G1 = Simplify[G /. sold]; G1 // TableForm
```

Out[74]//TableForm=

|                                |                                |                                            |                                            |                                            |                                            |
|--------------------------------|--------------------------------|--------------------------------------------|--------------------------------------------|--------------------------------------------|--------------------------------------------|
| 1                              | 0                              | $\frac{1}{2 \times (-1 + Jc)}$             | $\frac{1}{2 - 2 Jc}$                       | $\frac{1}{2 - 2 Jc}$                       | $\frac{1}{2 \times (-1 + Jc)}$             |
| 0                              | 1                              | $\frac{1}{2 \times (-1 + Jc)}$             | $\frac{1}{2 \times (-1 + Jc)}$             | $\frac{1}{2 - 2 Jc}$                       | $\frac{1}{2 - 2 Jc}$                       |
| $\frac{1}{2 \times (-1 + Jc)}$ | $\frac{1}{2 \times (-1 + Jc)}$ | 1                                          | $\frac{-1 + 4 Jc - 2 Jc^2}{2 (-1 + Jc)^2}$ | $\frac{(-2 + Jc) Jc}{(-1 + Jc)^2}$         | $\frac{-1 + 4 Jc - 2 Jc^2}{2 (-1 + Jc)^2}$ |
| $\frac{1}{2 - 2 Jc}$           | $\frac{1}{2 \times (-1 + Jc)}$ | $\frac{-1 + 4 Jc - 2 Jc^2}{2 (-1 + Jc)^2}$ | 1                                          | $\frac{-1 + 4 Jc - 2 Jc^2}{2 (-1 + Jc)^2}$ | $\frac{(-2 + Jc) Jc}{(-1 + Jc)^2}$         |
| $\frac{1}{2 - 2 Jc}$           | $\frac{1}{2 - 2 Jc}$           | $\frac{(-2 + Jc) Jc}{(-1 + Jc)^2}$         | $\frac{-1 + 4 Jc - 2 Jc^2}{2 (-1 + Jc)^2}$ | 1                                          | $\frac{-1 + 4 Jc - 2 Jc^2}{2 (-1 + Jc)^2}$ |
| $\frac{1}{2 \times (-1 + Jc)}$ | $\frac{1}{2 - 2 Jc}$           | $\frac{-1 + 4 Jc - 2 Jc^2}{2 (-1 + Jc)^2}$ | $\frac{(-2 + Jc) Jc}{(-1 + Jc)^2}$         | $\frac{-1 + 4 Jc - 2 Jc^2}{2 (-1 + Jc)^2}$ | 1                                          |

After some calculations which will not be presented here we found that the following spin configuration  $T$  (complemented by the antipodes) has the same Gram matrix  $G1$ . Note that this configuration is no longer rigid since it depends on  $Jc$ .

$$\text{In[75]:= } T = \begin{pmatrix} -\frac{1}{\sqrt{2}} & -\frac{1}{\sqrt{2}} & 0 \\ -\frac{1}{\sqrt{2}} & \frac{1}{\sqrt{2}} & 0 \\ -\frac{1}{\sqrt{2}(-1+Jc)} & 0 & \frac{\sqrt{\frac{1}{2}+(-2+Jc)Jc}}{-1+Jc} \\ 0 & \frac{1}{\sqrt{2}(-1+Jc)} & -\frac{\sqrt{\frac{1}{2}+(-2+Jc)Jc}}{-1+Jc} \\ \frac{1}{\sqrt{2}(-1+Jc)} & 0 & \frac{\sqrt{\frac{1}{2}+(-2+Jc)Jc}}{-1+Jc} \\ 0 & -\frac{1}{\sqrt{2}(-1+Jc)} & -\frac{\sqrt{\frac{1}{2}+(-2+Jc)Jc}}{-1+Jc} \\ \frac{1}{\sqrt{2}} & \frac{1}{\sqrt{2}} & 0 \\ \frac{1}{\sqrt{2}} & -\frac{1}{\sqrt{2}} & 0 \\ \frac{1}{\sqrt{2}(-1+Jc)} & 0 & -\frac{\sqrt{\frac{1}{2}+(-2+Jc)Jc}}{-1+Jc} \\ 0 & -\frac{1}{\sqrt{2}(-1+Jc)} & \frac{\sqrt{\frac{1}{2}+(-2+Jc)Jc}}{-1+Jc} \\ -\frac{1}{\sqrt{2}(-1+Jc)} & 0 & -\frac{\sqrt{\frac{1}{2}+(-2+Jc)Jc}}{-1+Jc} \\ 0 & \frac{1}{\sqrt{2}(-1+Jc)} & \frac{\sqrt{\frac{1}{2}+(-2+Jc)Jc}}{-1+Jc} \end{pmatrix};$$

`In[76]:= G2 = Table[Simplify[T[[i]].T[[j]]], {i, 6}, {j, 6}];`

`In[77]:= FullSimplify[G1 == G2]`

`Out[77]= True`

We graphically present the ground state configuration T for the special case  $J_p=1, J_c=-1/100$ :

```
In[78]:= H2 = Table[N[T[[i]].T[[j]] /. deformed], {i, 12}, {j, 12}]; H2 // TableForm
```

```
Out[78]//TableForm=
```

|          |          |           |           |           |           |          |
|----------|----------|-----------|-----------|-----------|-----------|----------|
| 1.       | 0.       | -0.49505  | 0.49505   | 0.49505   | -0.49505  | -1.      |
| 0.       | 1.       | -0.49505  | -0.49505  | 0.49505   | 0.49505   | 0.       |
| -0.49505 | -0.49505 | 1.        | -0.509852 | 0.019704  | -0.509852 | 0.49505  |
| 0.49505  | -0.49505 | -0.509852 | 1.        | -0.509852 | 0.019704  | -0.49505 |
| 0.49505  | 0.49505  | 0.019704  | -0.509852 | 1.        | -0.509852 | -0.49505 |
| -0.49505 | 0.49505  | -0.509852 | 0.019704  | -0.509852 | 1.        | 0.49505  |
| -1.      | 0.       | 0.49505   | -0.49505  | -0.49505  | 0.49505   | 1.       |
| 0.       | -1.      | 0.49505   | 0.49505   | -0.49505  | -0.49505  | 0.       |
| 0.49505  | 0.49505  | -1.       | 0.509852  | -0.019704 | 0.509852  | -0.49505 |
| -0.49505 | 0.49505  | 0.509852  | -1.       | 0.509852  | -0.019704 | 0.49505  |
| -0.49505 | -0.49505 | -0.019704 | 0.509852  | -1.       | 0.509852  | 0.49505  |
| 0.49505  | -0.49505 | 0.509852  | -0.019704 | 0.509852  | -1.       | -0.49505 |

```
In[79]:= pairs = Flatten[Table[{i, j}, {i, 12}, {j, i + 1, 12}], 1];
```

```
In[80]:= ED2 = Select[pairs, 0.49 < H2[[#1]], #[2]] < 0.51 &];
```

```
In[81]:= Graphics3D[Join[{Opacity[0.2], Sphere[]},
  Table[{PointSize[0.02], Opacity[1], Point[T[[μ]] /. deformed]}, {μ, 12}],
  Table[{Text[Style[μ, 14, Opacity[1], Red], 1.1 T[[μ]] /. deformed]}, {μ, 12}],
  Table[{Blue, Opacity[1], Line[{T[[ED2[[k, 1]]] /. deformed, T[[ED2[[k, 2]]] /. deformed]}],
    {k, Length[ED2]}]], Boxed → False]
```

```
Out[81]=
```

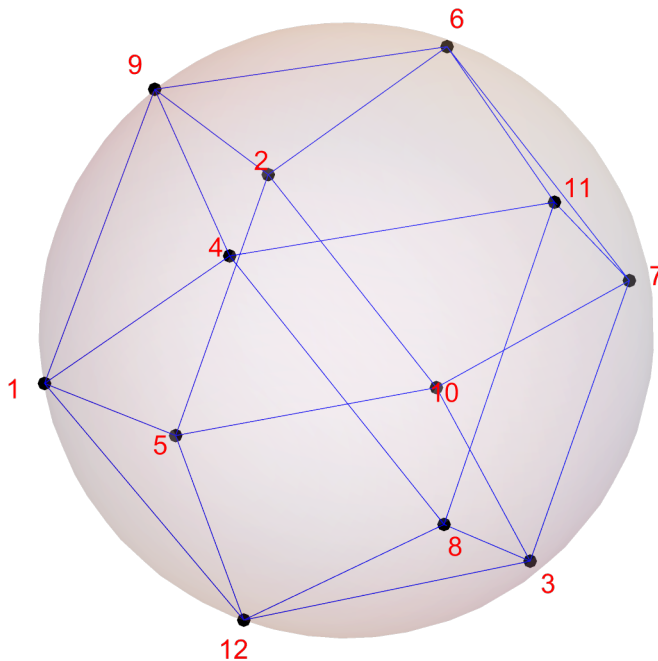



Another example is given by  $J_p=1$  and  $J_c=-1/10$ :

In[82]:= **val** = {  $J_p \rightarrow 1$ ,  $J_c \rightarrow -\frac{1}{10}$  }

Out[82]= {  $J_p \rightarrow 1$ ,  $J_c \rightarrow -\frac{1}{10}$  }

In[83]:= **T /. val // TableForm**

Out[83]//TableForm=

|                         |                         |                         |
|-------------------------|-------------------------|-------------------------|
| $-\frac{1}{\sqrt{2}}$   | $-\frac{1}{\sqrt{2}}$   | 0                       |
| $-\frac{1}{\sqrt{2}}$   | $\frac{1}{\sqrt{2}}$    | 0                       |
| $\frac{5\sqrt{2}}{11}$  | 0                       | $-\frac{\sqrt{71}}{11}$ |
| 0                       | $-\frac{5\sqrt{2}}{11}$ | $\frac{\sqrt{71}}{11}$  |
| $-\frac{5\sqrt{2}}{11}$ | 0                       | $-\frac{\sqrt{71}}{11}$ |
| 0                       | $\frac{5\sqrt{2}}{11}$  | $\frac{\sqrt{71}}{11}$  |
| $\frac{1}{\sqrt{2}}$    | $\frac{1}{\sqrt{2}}$    | 0                       |
| $\frac{1}{\sqrt{2}}$    | $-\frac{1}{\sqrt{2}}$   | 0                       |
| $-\frac{5\sqrt{2}}{11}$ | 0                       | $\frac{\sqrt{71}}{11}$  |
| 0                       | $\frac{5\sqrt{2}}{11}$  | $-\frac{\sqrt{71}}{11}$ |
| $\frac{5\sqrt{2}}{11}$  | 0                       | $\frac{\sqrt{71}}{11}$  |
| 0                       | $-\frac{5\sqrt{2}}{11}$ | $-\frac{\sqrt{71}}{11}$ |

In this case the deformed cuboctahedron assumes the form :

```
In[84]:= Graphics3D[Join[{Opacity[0.2], Sphere[]},
  Table[{PointSize[0.02], Opacity[1], Point[T[[μ]] /. val]}, {μ, 12}],
  Table[{Text[Style[μ, 14, Opacity[1], Red], 1.1 T[[μ]] /. val]}, {μ, 12}], {Blue,
  Opacity[1], Line[{T[[12]] /. val, T[[5]] /. val, T[[10]] /. val, T[[3]] /. val, T[[12]] /. val}],
  Line[{T[[4]] /. val, T[[9]] /. val, T[[6]] /. val, T[[11]] /. val, T[[4]] /. val}], Red, Line[
  {T[[1]] /. val, T[[2]] /. val, T[[7]] /. val, T[[8]] /. val, T[[1]] /. val}]}], Boxed → False]
```

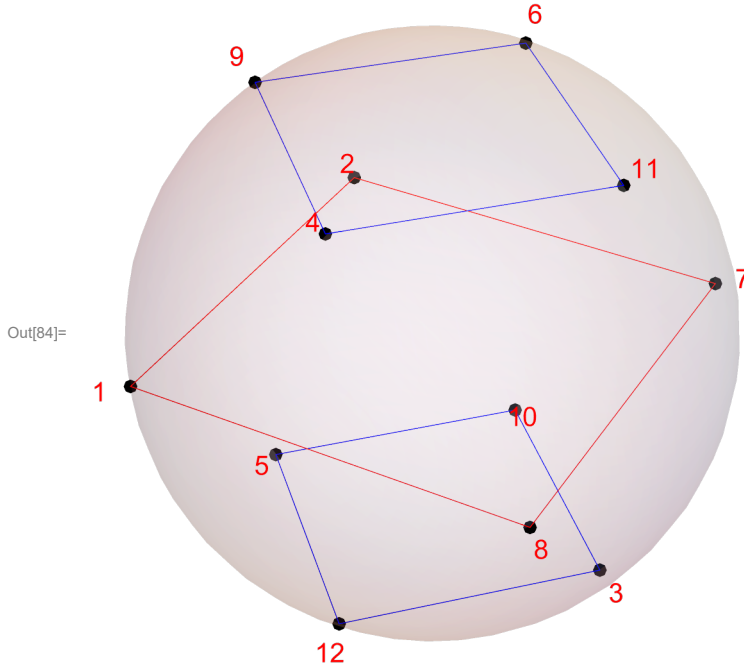

The outer (blue) squares have (opposite) z-values that deviate from the values of the cuboctahedron. The middle (red) square is still lying in the  $z=0$  plane and is not deformed.

The symmetry group of the deformed cuboc phase is  $\mathbf{D}_4^\sigma$ .

Recall that  $D_4$  is the symmetry group of a square, of order 8, and

$$\sigma = \begin{pmatrix} -1 & 0 & 0 \\ 0 & -1 & 0 \\ 0 & 0 & -1 \end{pmatrix} \text{ is the reflection at the origin.}$$

The magnetic unit cell is the same as for the cuboc phase, namely of size  $6 \times 2 \times 2$ .
