# Supplementary material for: Non-Coplanar Magnetic Orders in Classical Square-Kagome Antiferromagnets
Source: arXiv:2302.04171 ancillary file (2023-11-30)

# Non-coplanar ground states for phase VI (FM octagon-plaquette coupling) and phase VII (deformed $120^\circ$ ground states)

First we will describe three 1-parameter families of ground states that connect the three coplanar ground states a , b and c described in the manuscript in the following way:

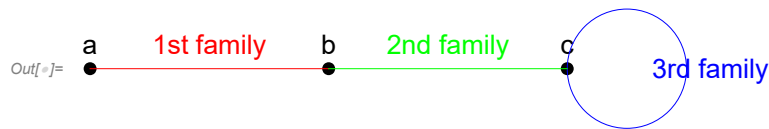

All ground states in the quadrant  $J_+, J_x < 0$  have to satisfy two rules:

- (1) The  $120^\circ$  rule, saying that the spins of adjacent spin sites have a mutual angle of  $120^\circ$ ,
- (2) The pairing rule, saying that spin pairs coupled by  $J_+$ , or  $J_x$  consist of identical spin vectors.

Conversely, every spin configuration satisfying (1) and (2) will be a ground state in the quadrant  $J_+, J_x < 0$

## Preparations

Definition of the squagome lattice, finite model with  $12 \times 12 = 144$  unit cells:

In[1]:= **L = 12;**

In[2]:= **Sites = Flatten[Table[{i, m, n}, {i, 6}, {m, 0, L - 1}, {n, 0, L - 1}], 2];**

In[3]:= **NN = len = Length[Sites]**

Out[3]= 864

Numbering of the sites in the primitive unit cell:

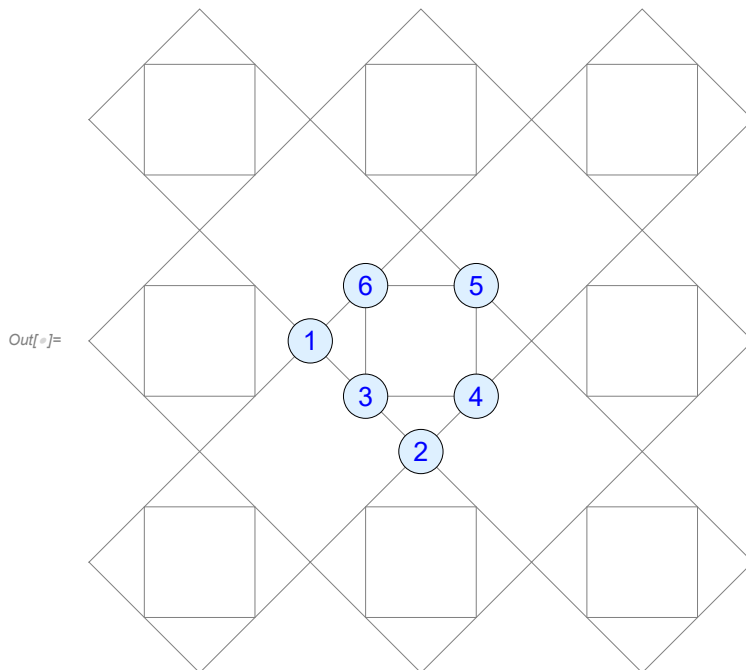

Spin sites will be encoded by multi - indices  $\{i, m, n\}$ , where  $m, n = 0, \dots, L - 1$  denote the position of the unit cell and  $i = 1, \dots, 6$  denotes the site number

within the unit cell. The sites in the primitive unit cell have the multi-indices  $\{i, 0, 0\}$ ,  $i = 1, \dots, 6$ . "Adjacency" of spin sites is always understood w.r.t. the  $(J_1, J_2, J_3)$ -lattice where  $J_+, J_x = 0$ .

### Definition of the J-matrix

```
In[4]:= J = Table[0, {len}, {len}];

In[5]:= For[μ = 1, μ ≤ len, μ++, {i1, n1, m1} = Sites[μ];
  For[ν = 1, ν ≤ len, ν++, {i2, n2, m2} = Sites[ν];
    If[n1 == n2 && m1 == m2, If[Sort[{i1, i2}] == {3, 4} || Sort[{i1, i2}] == {4, 5} ||
      Sort[{i1, i2}] == {5, 6} || Sort[{i1, i2}] == {3, 6}, J[[μ, ν]] = J[[ν, μ]] = J1]];
    If[n1 == n2 && m1 == m2, If[Sort[{i1, i2}] == {1, 3} || Sort[{i1, i2}] == {2, 4},
      J[[μ, ν]] = J[[ν, μ]] = J2]];
    If[n1 == n2 && m1 == m2, If[Sort[{i1, i2}] == {1, 6} || Sort[{i1, i2}] == {2, 3},
      J[[μ, ν]] = J[[ν, μ]] = J3]];
    If[Mod[n1 - 1 - n2, L] == 0 && m1 == m2, If[{i1, i2} == {1, 5}, J[[μ, ν]] = J[[ν, μ]] = J2]];
    If[Mod[n1 - 1 - n2, L] == 0 && m1 == m2, If[{i1, i2} == {1, 4}, J[[μ, ν]] = J[[ν, μ]] = J3]];
    If[Mod[n1 - 1 - n2, L] == 0 && m1 == m2, If[{i1, i2} == {2, 2}, J[[μ, ν]] = J[[ν, μ]] = Jp]];
    If[Mod[n1 + 1 - n2, L] == 0 && m1 == m2, If[{i1, i2} == {2, 2}, J[[μ, ν]] = J[[ν, μ]] = Jp]];
    If[Mod[m1 - 1 - m2, L] == 0 && n1 == n2, If[{i1, i2} == {2, 6}, J[[μ, ν]] = J[[ν, μ]] = J2]];
    If[Mod[m1 - 1 - m2, L] == 0 && n1 == n2, If[{i1, i2} == {2, 5}, J[[μ, ν]] = J[[ν, μ]] = J3]];
    If[Mod[m1 - 1 - m2, L] == 0 && n1 == n2, If[{i1, i2} == {1, 1}, J[[μ, ν]] = J[[ν, μ]] = Jp]];
    If[Mod[m1 + 1 - m2, L] == 0 && n1 == n2, If[{i1, i2} == {1, 1}, J[[μ, ν]] = J[[ν, μ]] = Jp]];
    If[Mod[m1 - 1 - m2, L] == 0 && Mod[n1 - 1 - n2, L] == 0,
      If[{i1, i2} == {3, 5}, J[[μ, ν]] = J[[ν, μ]] = Jc]];
    If[Mod[m1 + 1 - m2, L] == 0 && Mod[n1 - 1 - n2, L] == 0,
      If[{i1, i2} == {6, 4}, J[[μ, ν]] = J[[ν, μ]] = Jc]];
    If[Mod[m1 - 1 - m2, L] == 0 && Mod[n1 + 1 - n2, L] == 0,
      If[{i1, i2} == {4, 6}, J[[μ, ν]] = J[[ν, μ]] = Jc]];
    If[Mod[m1 + 1 - m2, L] == 0 && Mod[n1 + 1 - n2, L] == 0,
      If[{i1, i2} == {5, 3}, J[[μ, ν]] = J[[ν, μ]] = Jc]]];
```

### Specialization to J1=J2=J3=1

```
In[6]:= JA = Simplify[J /. {J1 → 1, J2 → 1, J3 → 1}];
```

```
In[7]:=
```

# First family

We reconsider the two coplanar ground states a and b considered in the main text, see Figure 8, and sketch them in the following way:

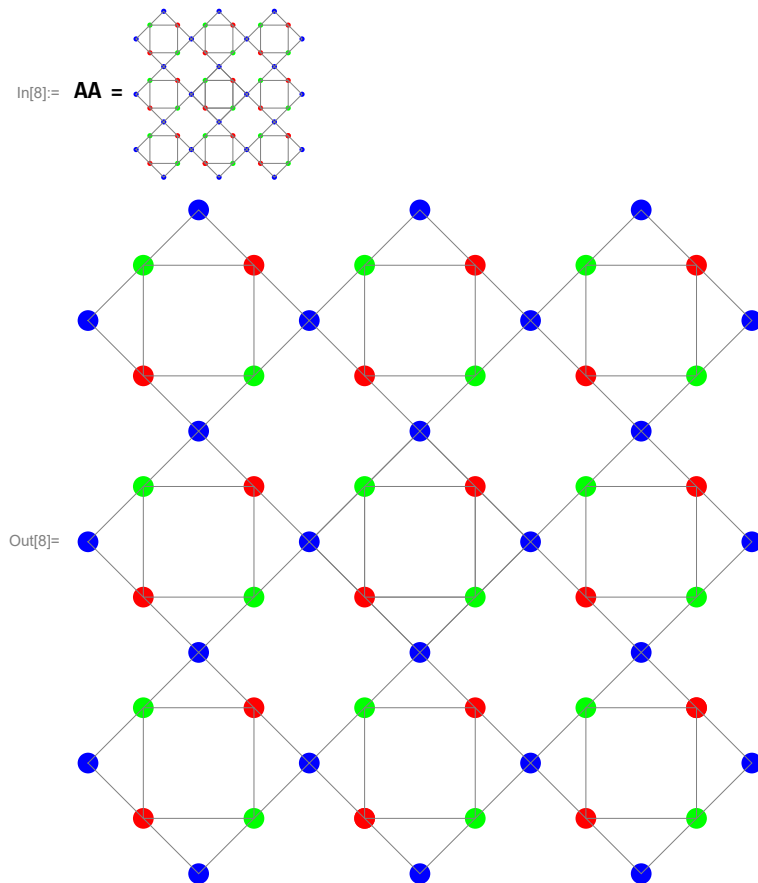

In[9]:=

**BB =**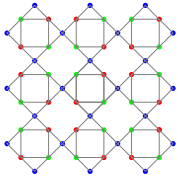

Out[9]=

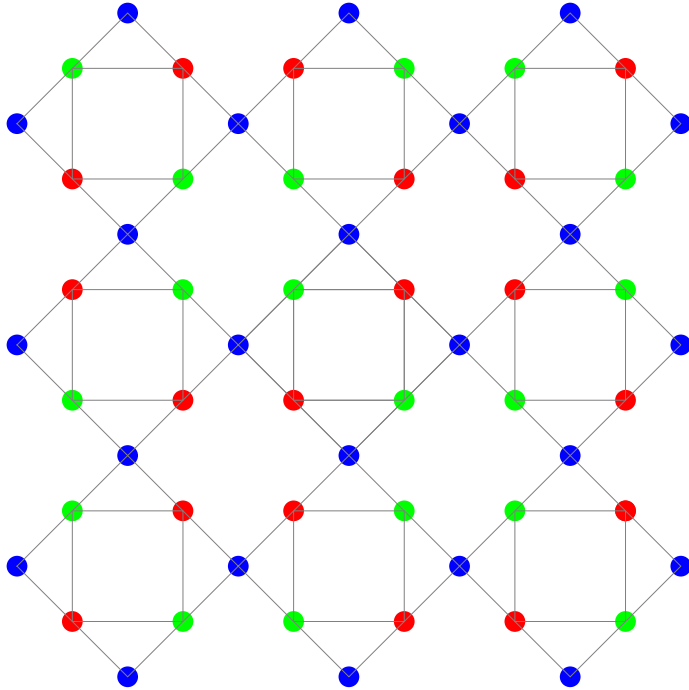

Both coplanar ground states a and b have a constant blue bow tie spin vector  $\mathbf{s}$  corresponding to the sites  $(1,m,n)$  and  $(2,m,n)$ , say,  $\mathbf{s}=(0,0,1)$ . Therefore, the remaining spins in the squares can be independently rotated about  $\mathbf{s}$  as long as the pairing rule is obeyed. This leads to family of non-coplanar ground states depending on a parameter  $\alpha$ .

The total spin configuration only uses the following 5 different spin vectors symbolized by 5 different colors:

```
In[10]:= Y1 = { {0, 0, 1}, {- $\frac{\sqrt{3}}{2}$ , 0, - $\frac{1}{2}$ }, { $\frac{\sqrt{3}}{2}$ , 0, - $\frac{1}{2}$ },
  {- $\frac{1}{2}\sqrt{3}\cos[\alpha]$ , - $\frac{1}{2}\sqrt{3}\sin[\alpha]$ , - $\frac{1}{2}$ }, { $\frac{1}{2}\sqrt{3}\cos[\alpha]$ ,  $\frac{1}{2}\sqrt{3}\sin[\alpha]$ , - $\frac{1}{2}$ }};
Z1 = Table[Flatten[{CB[[i]], Y1[[i]]}], {i, 5}] // TableForm
```

Part: Part specification CB[[1]] is longer than depth of object.

Part: Part specification CB[[2]] is longer than depth of object.

Part: Part specification CB[[3]] is longer than depth of object.

General: Further output of Part::partd will be suppressed during this calculation.

```
Out[10]//TableForm=
  CB[[1]]      0      0      1
  CB[[2]]      - $\frac{\sqrt{3}}{2}$       0      - $\frac{1}{2}$ 
  CB[[3]]       $\frac{\sqrt{3}}{2}$       0      - $\frac{1}{2}$ 
  CB[[4]]      - $\frac{1}{2}\sqrt{3}\cos[\alpha]$       - $\frac{1}{2}\sqrt{3}\sin[\alpha]$       - $\frac{1}{2}$ 
  CB[[5]]       $\frac{1}{2}\sqrt{3}\cos[\alpha]$        $\frac{1}{2}\sqrt{3}\sin[\alpha]$       - $\frac{1}{2}$ 
```

The spin vectors  $S1[\mu]$  for the lattice sites  $\mu=(i,m,n)$  will be defined as follows:

```
In[11]:= Clear[S1]
In[12]:= For[ $\mu = 1, \mu \leq NN, \mu++$ , {i, m, n} = Sites[[ $\mu$ ]];
  S1[ $\mu$ ] = Which[i == 1 | i == 2, Y1[[1]], EvenQ[m + n] && OddQ[i], Y1[[2]], EvenQ[m + n] &&
    EvenQ[i], Y1[[3]], OddQ[m + n] && OddQ[i], Y1[[4]], OddQ[m + n] && EvenQ[i], Y1[[5]]];
```

The first family of non-coplanar ground states will be sketched in the following figure:

```
In[13]:= CB = {Black, Orange, Yellow, Green, Blue, Cyan, Purple, Magenta, Red};
```

```
In[14]:= col1[ $\mu_+$ ] := CB[[Position[Y1, S1[ $\mu$ ]][[1, 1]]]
```

```

In[15]:= e[3] = {0, 0};
          e[4] = {1, 0};
          e[5] = {1, 1};
          e[6] = {0, 1};
          e[1] = {-0.5, 0.5};
          e[2] = {0.5, -0.5};
          e1 = {2, 0};
          e2 = {0, 2};

In[17]:= L2 = 3;
Graphics[{Table[{Gray, Line[{e[3] + m e1 + n e2, e[4] + m e1 + n e2, e[5] + m e1 + n e2,
          e[6] + m e1 + n e2, e[3] + m e1 + n e2}], Line[{e[1] + m e1 + n e2, e[2] + m e1 + n e2,
          e[1] + (m + 1) e1 + n e2, e[2] + m e1 + (n + 1) e2, e[1] + m e1 + n e2}]}],
          {m, 1, L2}, {n, 1, L2}], Table[μ = Position[Sites, {i, m, n}][[1, 1]];
          {col1[μ], PointSize[0.03], Point[e[i] + m e1 + n e2]}, {i, 6}, {m, 1, L2}, {n, 1, L2}]]]

```

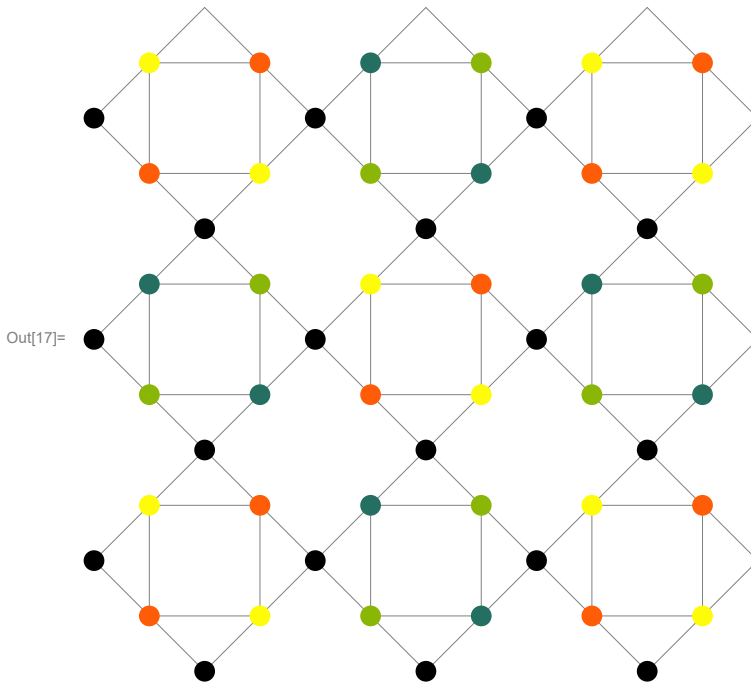

A test follows whether the known minimal energy function

$E = \frac{1}{3} \times (-3 + Jc + Jp)$  of the coplanar  $120^\circ$  ground states is also obtained by the above defined spin configuration:

```

In[18]:= E1 = Simplify[1 / (2 NN) Sum[JA[μ, ν] × Simplify[S1[μ].S1[ν]], {μ, NN}, {ν, NN}]]

Out[18]= 1/3 × (-3 + Jc + Jp)

```

Now we consider the limit cases, first  $\alpha \rightarrow 0$ :

```

In[19]:= Y10 = Union[Simplify[Y1 /. α → 0]]

Out[19]= {{0, 0, 1}, {-√3/2, 0, -1/2}, {√3/2, 0, -1/2}}

```

```
In[20]:= col10[μ_] := CB[Position[Y10, Simplify[S1[μ] /. α → 0]]][1, 1]]
```

```
In[21]:= L2 = 3;
```

```
Graphics[{Table[{Gray, Line[{e[3] + m e1 + n e2, e[4] + m e1 + n e2, e[5] + m e1 + n e2,
e[6] + m e1 + n e2, e[3] + m e1 + n e2}], Line[{e[1] + m e1 + n e2, e[2] + m e1 + n e2,
e[1] + (m + 1) e1 + n e2, e[2] + m e1 + (n + 1) e2, e[1] + m e1 + n e2}]}],
{m, 1, L2}, {n, 1, L2}], Table[μ = Position[Sites, {i, m, n}][1, 1];
{col10[μ], PointSize[0.03], Point[e[i] + m e1 + n e2]}, {i, 6}, {m, 1, L2}, {n, 1, L2}]]]
```

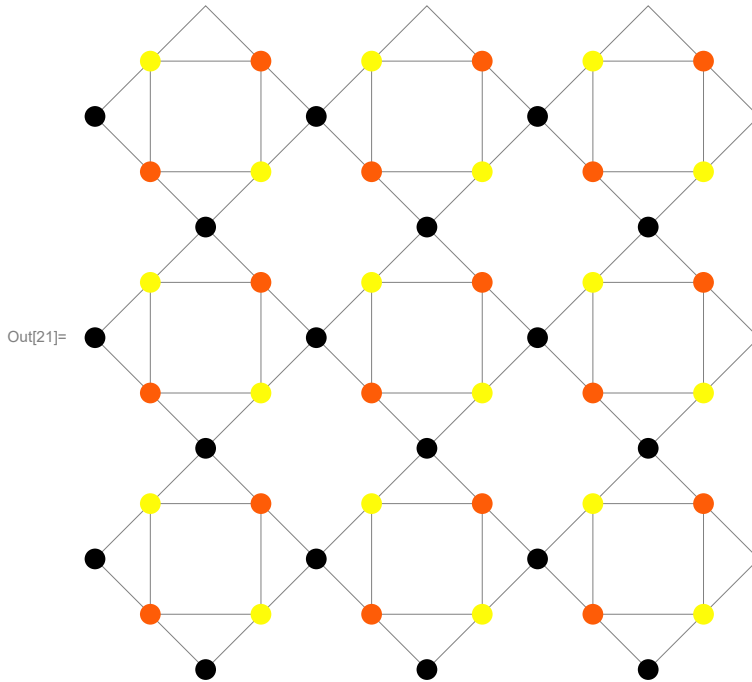

This is obviously the coplanar configuration considered above.  
Next consider  $\alpha \rightarrow \pi$ :

```
In[22]:= Y11 = Union[Simplify[Y1 /. α → π]]
```

```
Out[22]= {{0, 0, 1}, {- $\frac{\sqrt{3}}{2}$ , 0, - $\frac{1}{2}$ }, { $\frac{\sqrt{3}}{2}$ , 0, - $\frac{1}{2}$ }}
```

```
In[23]:= col11[μ_] := CB[Position[Y11, Simplify[S1[μ] /. α → π]]][1, 1]]
```



```

In[24]:= L2 = 3;
Graphics[{Table[{Gray, Line[{e[3] + m e1 + n e2, e[4] + m e1 + n e2, e[5] + m e1 + n e2,
e[6] + m e1 + n e2, e[3] + m e1 + n e2}], Line[{e[1] + m e1 + n e2, e[2] + m e1 + n e2,
e[1] + (m + 1) e1 + n e2, e[2] + m e1 + (n + 1) e2, e[1] + m e1 + n e2}]}],
{m, 1, L2}, {n, 1, L2}], Table[μ = Position[Sites, {i, m, n}][[1, 1]];
{col11[μ], PointSize[0.03], Point[e[i] + m e1 + n e2]}, {i, 6}, {m, 1, L2}, {n, 1, L2}]]]

```

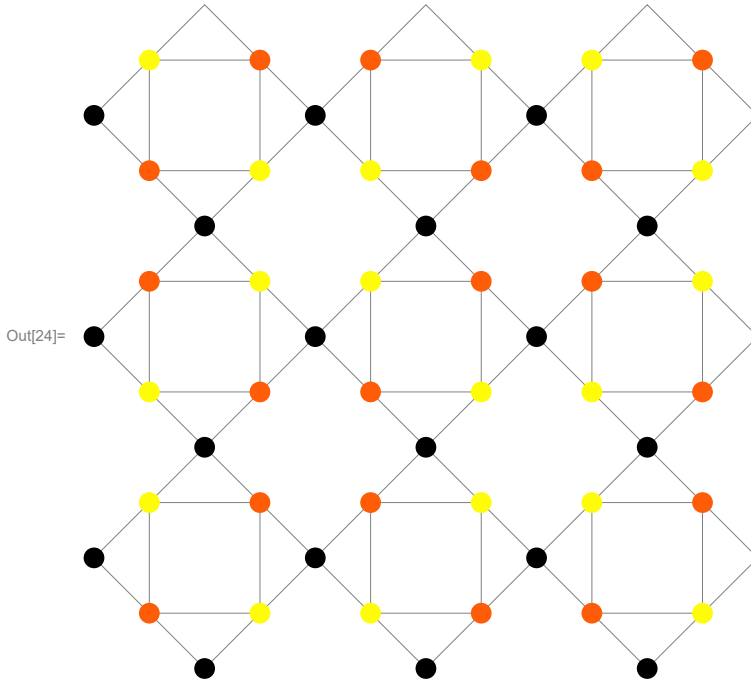

This is obviously the coplanar configuration b considered above, thereby confirming the following part of the above sketch:

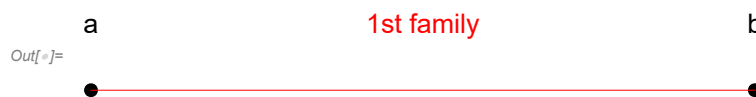

In[25]:=

## First family, alternative derivation

We will present another derivation of the 1st family based on generalized Luttinger-Tizsa theory and start with the Fourier-transformed dressed J-Matrix  $JJ(q_1, q_2, \lambda)$ :

In[26]:= **Clear** [ $\lambda$ ]

```
In[27]:= JJ = Simplify[{{2 Jp Cos[q2] + 2 λ, 0, J2, J3 Exp[-i q1], J2 Exp[-i q1], J3},
  {0, 2 Jp Cos[q1] + 2 λ, J3, J2, J3 Exp[-i q2], J2 Exp[-i q2]}, {J2, J3, -λ, J1,
  Jc (Exp[-i (q1 + q2)]), J1}, {J3 Exp[i q1], J2, J1, -λ, J1, Jc (Exp[i (q1 - q2)])},
  {J2 Exp[i q1], J3 Exp[i q2], Jc (Exp[i (q1 + q2)]), J1, -λ, J1},
  {J3, J2 Exp[i q2], J1, Jc (Exp[i (q2 - q1)]), J1, -λ}}];
```

```
In[28]:= JJB = Simplify[JJ /. {J1 → 1, J2 → 1, J3 → 1}]; JJB // TableForm
```

```
Out[28]//TableForm=
```

|                               |                               |                         |                          |                          |                         |
|-------------------------------|-------------------------------|-------------------------|--------------------------|--------------------------|-------------------------|
| $2 (\lambda + J_p \cos[q_2])$ | 0                             | 1                       | $e^{-i q_1}$             | $e^{-i q_1}$             | 1                       |
| 0                             | $2 (\lambda + J_p \cos[q_1])$ | 1                       | 1                        | $e^{-i q_2}$             | $e^{-i q_2}$            |
| 1                             | 1                             | $-\lambda$              | 1                        | $e^{-i (q_1 + q_2)} J_c$ | 1                       |
| $e^{i q_1}$                   | 1                             | 1                       | $-\lambda$               | 1                        | $e^{i (q_1 - q_2)} J_c$ |
| $e^{i q_1}$                   | $e^{i q_2}$                   | $e^{i (q_1 + q_2)} J_c$ | 1                        | $-\lambda$               | 1                       |
| 1                             | $e^{i q_2}$                   | 1                       | $e^{i (-q_1 + q_2)} J_c$ | 1                        | $-\lambda$              |

```
In[29]:= NL = L / 2
```

```
Out[29]= 6
```

```
In[30]:= Q = Sort[Flatten[Join[Table[{n1 π / NL, n2 π / NL}, {n1, 1, NL}, {n2, -NL, NL}],
  Table[{n1 π / NL, n2 π / NL}, {n1, 0, 0}, {n2, 0, NL}]], 1]];
```

```
In[31]:= Q = Delete[Q, Position[Q, {π, -π}]];
```

```
In[32]:= Length[Q]
```

```
Out[32]= 84
```

We look at the reference point  $J_p = J_c = -1$  and verify that the minimal eigenvalue

is  $-10/3$  of JJ is assumed for  $\mathbf{q} \in \{0,0\}, \{0,\pi\}, \{\pi,0\}, \{\pi,\pi\}$  and  $\lambda = 1/3$ :

```
In[33]:= val = {Jp → -1, Jc → -1}
```

```
Out[33]= {Jp → -1, Jc → -1}
```

```
In[34]:= Plot[Min[Table[Min[Re[Eigenvalues[N[JJB /. val /. {q1 → Q[[q, 1], q2 → Q[[q, 2]]]]],
  {q, Length[Q]}]], {λ, 0, 1}]]
```

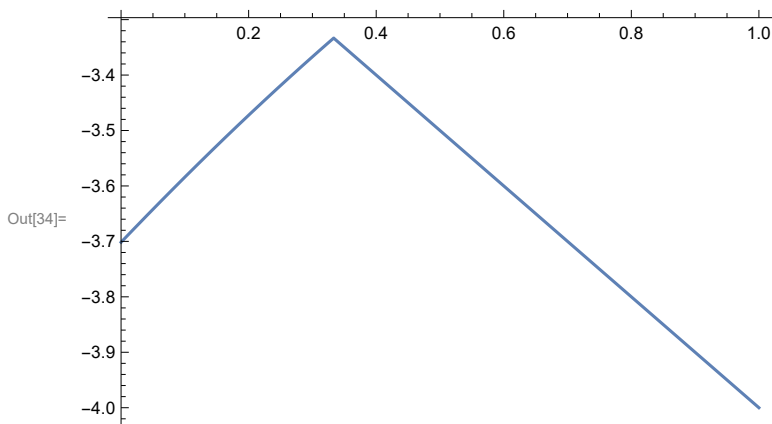

```
In[35]:= {ee, rule} = FindMaximum[
  Min[Table[Min[Re[Eigenvalues[N[JJB /. val /. {q1 → Q[i, 1], q2 → Q[i, 2]]}]]],
    {q, Length[Q]}]], {λ, 0.5}]
```

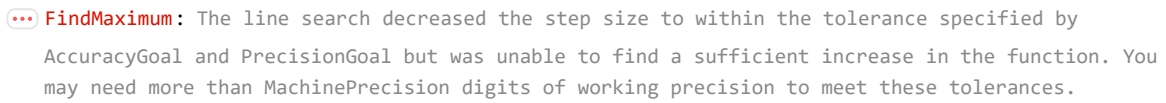 **FindMaximum:** The line search decreased the step size to within the tolerance specified by AccuracyGoal and PrecisionGoal but was unable to find a sufficient increase in the function. You may need more than MachinePrecision digits of working precision to meet these tolerances.

```
Out[35]= {-3.33333, {λ → 0.333333}}
```

```
In[36]:= tab = Table[Rationalize[
  Min[Re[N[Eigenvalues[N[JJB /. val /. {q1 → Q[i, 1], q2 → Q[i, 2]] /. rule]]]],
  10^(-8)], {i, Length[Q]}];
```

```
In[37]:= pos = Position[tab, Min[tab]]
```

```
Out[37]= {{1}, {7}, {73}, {84}}
```

```
In[38]:= {Q[[1]], Q[[7]], Q[[73]], Q[[84]]}
```

```
Out[38]= {{0, 0}, {0, π}, {π, 0}, {π, π}}
```

The condition that, for example,  $JJ(0,0,\lambda)$  and  $JJ(0,\pi,\lambda)$  have a common eigenvalue leads to the equation  $\lambda = \frac{1}{3} (Jc - 2 Jp)$  for the (reduced) Lagrange parameter  $\lambda$  and to the minimal energy function

$$E1 = \frac{1}{3} \times (-3 + Jc + Jp):$$

```
In[39]:= pa = Factor[Simplify[CharacteristicPolynomial[JJB /. {q1 → 0, q2 → 0}, z]]]
```

```
Out[39]= (-2 Jp + z - 2 λ) × (-2 + Jc - z - λ) (Jc + z + λ)2
(8 - 4 Jp - 2 Jc Jp + 2 z + Jc z + 2 Jp z - z2 - 4 λ - 2 Jc λ + 2 Jp λ + z λ + 2 λ2)
```

```
In[40]:= solz = Solve[0 == (8 - 4 Jp - 2 Jc Jp + 2 z + Jc z + 2 Jp z - z2 - 4 λ - 2 Jc λ + 2 Jp λ + z λ + 2 λ2), z];
solz /. val /. rule
```

```
Out[41]= {{z → -3.33333}, {z → 2.66667}}
```

```
In[42]:= ee
```

```
Out[42]= -3.33333
```

```
In[43]:= pb = Factor[Simplify[CharacteristicPolynomial[JJB /. {q1 → 0, q2 → π}, z]]]
```

```
Out[43]= (Jc - z - λ) (2 + Jc + z + λ) ×
(-4 - 4 Jp + 2 Jc Jp - 2 z + Jc z + 2 Jp z + z2 + 4 λ - 2 Jc λ + 2 Jp λ - z λ - 2 λ2) ×
(4 - 2 Jc Jp + Jc z + 2 Jp z - z2 - 2 Jc λ + 2 Jp λ + z λ + 2 λ2)
```

```
In[44]:= solz = Solve[0 == (4 - 2 Jc Jp + Jc z + 2 Jp z - z2 - 2 Jc λ + 2 Jp λ + z λ + 2 λ2), z];
solz /. val /. rule
```

```
Out[45]= {{z → -3.33333}, {z → 0.666667}}
```

```
In[46]:= ee
```

```
Out[46]= -3.33333
```

```
In[47]:= res = Factor[
  Simplify[Resultant[(8 - 4 Jp - 2 Jc Jp + 2 z + Jc z + 2 Jp z - z^2 - 4 λ - 2 Jc λ + 2 Jp λ + z λ + 2 λ^2),
    (4 - 2 Jc Jp + Jc z + 2 Jp z - z^2 - 2 Jc λ + 2 Jp λ + z λ + 2 λ^2), z]]]
```

```
Out[47]= 8 (Jc - 2 Jp - 3 λ)
```

```
In[48]:= soll = Simplify[Solve[res == 0, λ][[1]]]
```

```
Out[48]= {λ →  $\frac{1}{3} (Jc - 2 Jp)$ }
```

```
In[49]:= N[soll /. val]
```

```
Out[49]= {λ → 0.333333}
```

```
In[50]:= rule
```

```
Out[50]= {λ → 0.333333}
```

```
In[51]:= Simplify[solz /. soll]
```

```
Out[51]= {{z →  $\frac{2}{3} \times (-3 + Jc + Jp)$ }, {z →  $\frac{2}{3} \times (3 + Jc + Jp)$ }}
```

```
In[52]:= Simplify[solz /. soll] /. val // N
```

```
Out[52]= {{z → -3.33333}, {z → 0.666667}}
```

```
In[53]:= E1 = Simplify[1 / 2 solz[[1, 1, 2]] /. soll]
```

```
Out[53]=  $\frac{1}{3} \times (-3 + Jc + Jp)$ 
```

Next we construct a spin configuration from the eigenspaces of  $JJ(0,0,\lambda)$  and  $JJ(\pi,\pi,\lambda)$  corresponding to the minimal eigenvalues. These eigenvectors do not depend on  $Jp$  or  $Jc$ , and hence the resulting spin configuration will be “rigid”.

```
In[54]:= esa = Eigensystem[JJB /. {q1 → 0, q2 → 0} /. soll]
```

```
Out[54]= {{ $-\frac{2}{3} \times (2 Jc - Jp)$ ,  $-\frac{2}{3} \times (2 Jc - Jp)$ ,  $\frac{2}{3} \times (-3 + Jc + Jp)$ ,  $\frac{2}{3} \times (-3 + Jc + Jp)$ ,  $\frac{2 (Jc + Jp)}{3}$ ,  $\frac{2}{3} \times (6 + Jc + Jp)$ }, {{0, 0, 0, -1, 0, 1}, {0, 0, -1, 0, 1, 0}, {-1, -1, 0, 1, 0, 1}, {-1, -1, 1, 0, 1, 0}, {-1, 1, 0, 0, 0, 0}, {1, 1, 1, 1, 1, 1}}}
```

```
In[55]:= esa[[1]] /. val // N
```

```
Out[55]= {0.666667, 0.666667, -3.33333, -3.33333, -1.33333, 2.66667}
```

```
In[56]:= ee
```

```
Out[56]= -3.33333
```

```
In[57]:= u = Simplify[esa[[2, 3]]]
```

```
Out[57]= {-1, -1, 0, 1, 0, 1}
```

```
In[58]:= w = Simplify[esa[[2, 4]]]
```

```
Out[58]= {-1, -1, 1, 0, 1, 0}
```

```
In[59]:= esc = Eigensystem[JJB /. {q1 → π, q2 → π} /. sol1];
```

```
In[60]:= esc[[1]] /. val // N
```

```
Out[60]= {-3.33333, 0.666667, 3.90273, 3.90273, -0.569401, -0.569401}
```

```
In[61]:= ee
```

```
Out[61]= -3.33333
```

```
In[62]:= v = Simplify[esc[[2, 1]]]
```

```
Out[62]= {0, 0, -1, 1, -1, 1}
```

The 6×3-matrix of eigenvectors  $W$  assumes the following form:

```
In[63]:= Wt = {u, v, w}; W = Transpose[Wt]; W // TableForm
```

```
Out[63]//TableForm=
```

```

-1      0      -1
-1      0      -1
 0      -1      1
 1       1      0
 0      -1      1
 1       1      0

```

```
In[64]:= MatrixRank[W]
```

```
Out[64]= 2
```

Further linear transformations within the eigenspaces are required for the 6 rows of  $W$  to become unit vectors. These transformations are represented by the matrix  $\Delta$ :

```
In[65]:= Δ =  $\begin{pmatrix} \delta_1 & 0 & \delta_3 \\ 0 & \delta_2 & 0 \\ \delta_3 & 0 & \delta_4 \end{pmatrix}$ ;
```

```
In[66]:= VAR = {δ1, δ2, δ3, δ4};
```

```
In[67]:= G = W.Δ.Wt;
```

```
In[68]:= sold = Simplify[Solve[Table[G[[i, i]] == 1, {i, 6}], VAR][[1]]]
```

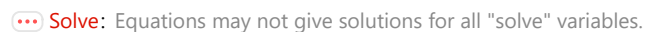 **Solve:** Equations may not give solutions for all "solve" variables.

```
Out[68]= {δ2 → 1 - δ1, δ3 →  $\frac{1}{2} - \delta_1$ , δ4 → δ1}
```

```
In[69]:= Δ1 = Δ /. sold; Δ1 // TableForm
```

```
Out[69]//TableForm=
```

```

δ1      0       $\frac{1}{2} - \delta_1$ 
 0      1 - δ1    0
 $\frac{1}{2} - \delta_1$   0      δ1

```

In[70]:= **G1 = Simplify[G /. sold]; G1 // TableForm**

Out[70]//TableForm=

$$\begin{array}{cccccc} 1 & 1 & -\frac{1}{2} & -\frac{1}{2} & -\frac{1}{2} & -\frac{1}{2} \\ 1 & 1 & -\frac{1}{2} & -\frac{1}{2} & -\frac{1}{2} & -\frac{1}{2} \\ -\frac{1}{2} & -\frac{1}{2} & 1 & -\frac{1}{2} & 1 & -\frac{1}{2} \\ -\frac{1}{2} & -\frac{1}{2} & -\frac{1}{2} & 1 & -\frac{1}{2} & 1 \\ -\frac{1}{2} & -\frac{1}{2} & 1 & -\frac{1}{2} & 1 & -\frac{1}{2} \\ -\frac{1}{2} & -\frac{1}{2} & -\frac{1}{2} & 1 & -\frac{1}{2} & 1 \end{array}$$

In[71]:= **Eigenvalues[Δ1]**

Out[71]=  $\left\{ \frac{1}{2}, 1 - \delta 1, \frac{1}{2} \times (-1 + 4 \delta 1) \right\}$

Thus we obtain 6 spin vectors in the primitive unit cell depending on a parameter  $\delta 1$  that has to satisfy  $0 \leq \delta 1 \leq 1/4$  in order to have  $\Delta 1 \geq 0$ . Using  $\Gamma 1 = \sqrt{\Delta 1}$  and a suitable rotation R2 in spin space we obtain the following (partial) spin configuration T2:

In[72]:= **r1 = Simplify[MatrixPower[Δ1, 1 / 2]]**

Out[72]=  $\left\{ \left\{ \frac{1 + \sqrt{-1 + 4 \delta 1}}{2 \sqrt{2}}, 0, -\frac{-1 + \sqrt{-1 + 4 \delta 1}}{2 \sqrt{2}} \right\}, \left\{ 0, \sqrt{1 - \delta 1}, 0 \right\}, \left\{ -\frac{-1 + \sqrt{-1 + 4 \delta 1}}{2 \sqrt{2}}, 0, \frac{1 + \sqrt{-1 + 4 \delta 1}}{2 \sqrt{2}} \right\} \right\}$

In[73]:= **R2 =  $\begin{pmatrix} -\frac{1}{\sqrt{2}} & 0 & -\frac{1}{\sqrt{2}} \\ 0 & 1 & 0 \\ \frac{1}{\sqrt{2}} & 0 & -\frac{1}{\sqrt{2}} \end{pmatrix}$ ;**

In[74]:= **T2 = Simplify[W.r1.R2]; T2 // TableForm**

Out[74]//TableForm=

$$\begin{array}{ccc} 0 & 0 & 1 \\ 0 & 0 & 1 \\ \frac{1}{2} \sqrt{-1 + 4 \delta 1} & -\sqrt{1 - \delta 1} & -\frac{1}{2} \\ -\frac{1}{2} \sqrt{-1 + 4 \delta 1} & \sqrt{1 - \delta 1} & -\frac{1}{2} \\ \frac{1}{2} \sqrt{-1 + 4 \delta 1} & -\sqrt{1 - \delta 1} & -\frac{1}{2} \\ -\frac{1}{2} \sqrt{-1 + 4 \delta 1} & \sqrt{1 - \delta 1} & -\frac{1}{2} \end{array}$$

T2, being restricted to the primitive unit cell, is still coplanar:

In[75]:= **MatrixRank[T2]**

Out[75]= 2

We extend T2 to a spin configuration T, defined on all 864 lattice sites, by

using that the 2nd component of the spin vectors, coming from the eigenvector  $v$  of  $JJ(\pi, \pi, \lambda)$ , is multiplied by -1 if we pass to neighbouring unit cells (right or left or up or down) and the other components are left unchanged:

```
In[76]:= F1 = DiagonalMatrix[{1, -1, 1}];
In[77]:= Clear[T]
In[78]:= For[μ = 1, μ ≤ NN, μ++, {i, m, n} = Sites[[μ]];
           U = Simplify[T2.MatrixPower[F1, m + n]];
           T[μ] = U[[i]]]
```

We will check that the spin configuration  $T$  still has the minimal energy  $\frac{1}{3} \times (-3 + J_c + J_p)$  known for  $120^\circ$  ground states in the sector  $J_p, J_c < 0$ :

```
In[79]:= EN = Simplify[1 / (2 NN) Sum[Simplify[JA[[μ, ν]] × T[μ].T[ν]], {μ, NN}, {ν, NN}]]
Out[79]=  $\frac{1}{3} \times (-3 + J_c + J_p)$ 
```

$T$  generally consists of only 5 different spin vectors

```
In[80]:= ST = Union[Table[T[μ], {μ, NN}]]; ST // TableForm
Out[80]//TableForm=
```

| 0                                     | 0                      | 1              |
|---------------------------------------|------------------------|----------------|
| $-\frac{1}{2} \sqrt{-1 + 4 \delta 1}$ | $-\sqrt{1 - \delta 1}$ | $-\frac{1}{2}$ |
| $-\frac{1}{2} \sqrt{-1 + 4 \delta 1}$ | $\sqrt{1 - \delta 1}$  | $-\frac{1}{2}$ |
| $\frac{1}{2} \sqrt{-1 + 4 \delta 1}$  | $-\sqrt{1 - \delta 1}$ | $-\frac{1}{2}$ |
| $\frac{1}{2} \sqrt{-1 + 4 \delta 1}$  | $\sqrt{1 - \delta 1}$  | $-\frac{1}{2}$ |

```
In[81]:= Length[ST]
Out[81]= 5
```

and represents a non-coplanar ground state:

```
In[82]:= MatrixRank[ST]
Out[82]= 3
```

The limit  $\delta 1 \rightarrow 1$  represents the coplanar ground state denoted by (a) in the main text, Figure 8. This follows from the form of T for the primitive unit cell and the fact that 2nd component of all spin vectors vanishes. Therefore, the q-vector  $(\pi, \pi)$ , which is responsible for a sign reversal of the 2nd component, is not active and the ground state (a) has only the q-vector (0,0).

```
In[83]:= Simplify[T2 /. {δ1 → 1}] // TableForm
```

```
Out[83]//TableForm=
```

|                       |   |                |
|-----------------------|---|----------------|
| 0                     | 0 | 1              |
| 0                     | 0 | 1              |
| $\frac{\sqrt{3}}{2}$  | 0 | $-\frac{1}{2}$ |
| $-\frac{\sqrt{3}}{2}$ | 0 | $-\frac{1}{2}$ |
| $\frac{\sqrt{3}}{2}$  | 0 | $-\frac{1}{2}$ |
| $-\frac{\sqrt{3}}{2}$ | 0 | $-\frac{1}{2}$ |

The other limit  $\delta 1 \rightarrow 1/4$  represents the coplanar ground state denoted by (b) in the main text, Figure 8. This follows from the form of T for the primitive unit cell and the fact that now the 1st component of all spin vectors vanishes. Therefore, the q-vector  $(\pi, \pi)$ , which is responsible for a sign reversal of the 2nd component, is still active and the ground state (b) has the q-vectors (0,0) and  $(\pi, \pi)$ .

```
In[84]:= Simplify[T2 /. {δ1 → 1 / 4}] // TableForm
```

```
Out[84]//TableForm=
```

|   |                       |                |
|---|-----------------------|----------------|
| 0 | 0                     | 1              |
| 0 | 0                     | 1              |
| 0 | $-\frac{\sqrt{3}}{2}$ | $-\frac{1}{2}$ |
| 0 | $\frac{\sqrt{3}}{2}$  | $-\frac{1}{2}$ |
| 0 | $-\frac{\sqrt{3}}{2}$ | $-\frac{1}{2}$ |
| 0 | $\frac{\sqrt{3}}{2}$  | $-\frac{1}{2}$ |

Summarizing, we can identify the family  $T(\delta 1)$  of ground states with the first family described above.

## Second family

According the the 120° rule the 4 spin vectors in the squares of each unit cell



form angles of  $120^\circ$  between vectors of adjacent spin sites. In the first family of ground states described above, in each unit cell there are only two such vectors, say **a** and **b**, such that the sequence of the 4 spin vector in the square reads (**a,b,a,b**).

But there exist more general configurations of 4 spin vectors that obey the  $120^\circ$  rule. They may be of the type (**a,b,a,c**) or (**a,b,c,d**).

We start with the case  $(r[3],r[4],r[5],r[6]) = (\mathbf{a},\mathbf{b},\mathbf{a},\mathbf{c})$ . The spin vectors  $r[i]$  in the primitive unit cell will be defined as follows, depending on a parameter  $\beta$ :

```
In[86]:= r[3] = r[5] = {0, 0, 1};
r[4] = {sqrt[3]/2 Cos[beta], sqrt[3]/2 Sin[beta], -1/2};
r[6] = {sqrt[3]/2 Cos[beta], -sqrt[3]/2 Sin[beta], -1/2};
```

Due to the pairing rule the spins in the squares of the other unit cells are defined according to the following permutations.

```
In[89]:= R1 = {1, 2, 4, 3, 6, 5}; R2 = {1, 2, 6, 5, 4, 3}; R12 = {1, 2, 5, 6, 3, 4};
In[90]:= Clear[S2]
In[91]:= For[i = 3, i <= 6, i++,
  For[m = 0, m <= L - 1, m++, For[n = 0, n <= L - 1, n++, mu = Position[Sites, {i, m, n}][[1, 1]];
    S2[mu] = Which[EvenQ[m] && EvenQ[n],
      r[i], OddQ[m] && EvenQ[n], r[R1[[i]],
      EvenQ[m] && OddQ[n], r[R2[[i]], OddQ[m] && OddQ[n], r[R12[[i]]]]]]]
```

The remaining bow tie spins are defined such that they complete  $120^\circ$  triangles:

```
In[92]:= For[m = 0, m <= L - 1, m++, For[n = 0, n <= L - 1, n++, mu = Position[Sites, {1, m, n}][[1, 1]];
  lambda = Position[Sites, {3, m, n}][[1, 1]];
  nu = Position[Sites, {6, m, n}][[1, 1]];
  S2[mu] = Simplify[-S2[lambda] - S2[nu]]]
In[93]:= For[m = 0, m <= L - 1, m++, For[n = 0, n <= L - 1, n++, mu = Position[Sites, {2, m, n}][[1, 1]];
  lambda = Position[Sites, {3, m, n}][[1, 1]];
  nu = Position[Sites, {4, m, n}][[1, 1]];
  S2[mu] = Simplify[-S2[lambda] - S2[nu]]]
```

The total spin configuration only uses the following 5 different spin vectors symbolized by different colors:

```
In[94]:= Y2 = Union[Table[S2[μ], {μ, NN}]];
```

```
Z2 = Table[Flatten[{CB[i], Y2[i]}], {i, 5}] // TableForm
```

```
Out[94]//TableForm=
```

|                                                                                   |                                     |                                     |                |
|-----------------------------------------------------------------------------------|-------------------------------------|-------------------------------------|----------------|
| 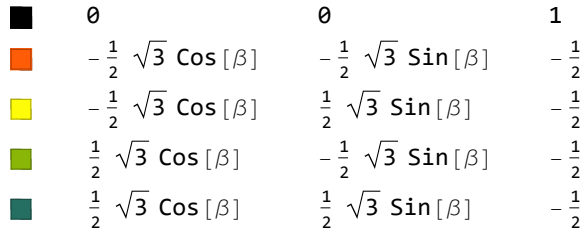 | 0                                   | 0                                   | 1              |
| 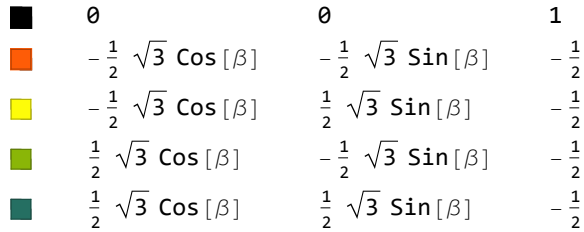 | $-\frac{1}{2} \sqrt{3} \cos[\beta]$ | $-\frac{1}{2} \sqrt{3} \sin[\beta]$ | $-\frac{1}{2}$ |
| 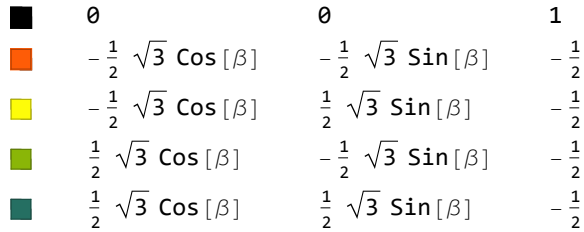 | $-\frac{1}{2} \sqrt{3} \cos[\beta]$ | $\frac{1}{2} \sqrt{3} \sin[\beta]$  | $-\frac{1}{2}$ |
| 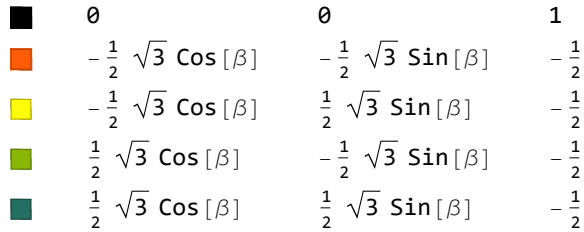 | $\frac{1}{2} \sqrt{3} \cos[\beta]$  | $-\frac{1}{2} \sqrt{3} \sin[\beta]$ | $-\frac{1}{2}$ |
| 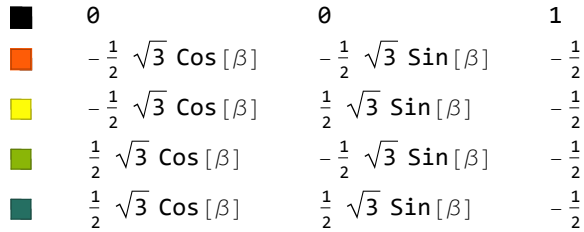 | $\frac{1}{2} \sqrt{3} \cos[\beta]$  | $\frac{1}{2} \sqrt{3} \sin[\beta]$  | $-\frac{1}{2}$ |

A test follows whether the known minimal energy function

$E = \frac{1}{3} \times (-3 + Jc + Jp)$  of the coplanar  $120^\circ$  ground states is also obtained by the above defined spin configuration:

```
In[95]:= E2 = Simplify[1 / (2 NN) Sum[JA[μ, ν] × Simplify[S2[μ].S2[ν]], {μ, NN}, {ν, NN}]]
```

```
Out[95]=  $\frac{1}{3} \times (-3 + Jc + Jp)$ 
```

Next we produce a graphical sketch of the spin configuration by using the 5 different colors:

```
In[96]:= col2[μ_] := CB[Position[Y2, S2[μ]][[1, 1]]]
```

```

In[97]:= Graphics[
  {Table[{Gray, Line[{e[3] + m e1 + n e2, e[4] + m e1 + n e2, e[5] + m e1 + n e2, e[6] + m e1 + n e2,
    e[3] + m e1 + n e2}], Line[{e[1] + m e1 + n e2, e[2] + m e1 + n e2,
    e[1] + (m + 1) e1 + n e2, e[2] + m e1 + (n + 1) e2, e[1] + m e1 + n e2}]}],
  {m, 1, L2}, {n, 1, L2}], Table[μ = Position[Sites, {i, m, n}][[1, 1]];
  {col2[μ], PointSize[0.03], Point[e[i] + m e1 + n e2]}, {i, 6}, {m, 1, L2}, {n, 1, L2}]]]

```

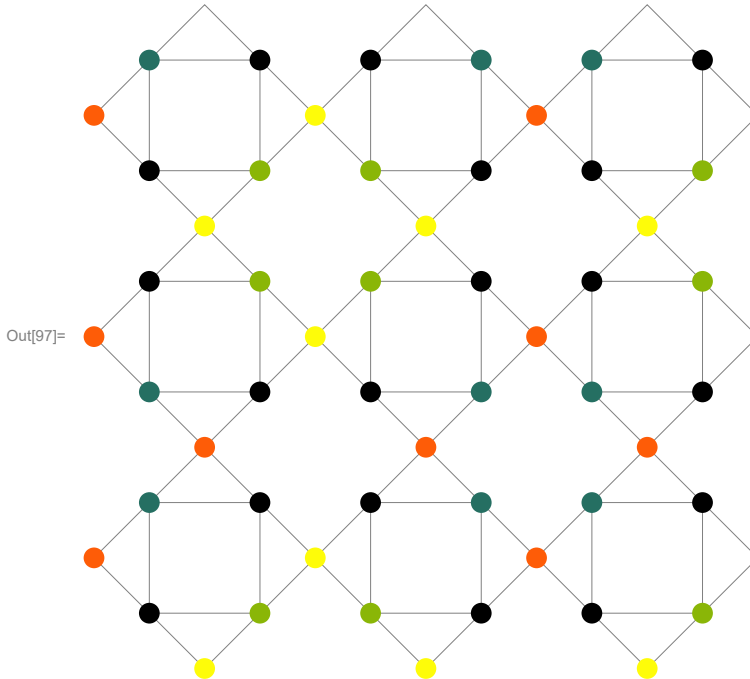

Now we consider the limit cases, first  $\beta \rightarrow 0$ :

```

In[98]:= Y20 = Union[Simplify[Y2 /. β → 0]]

```

```

Out[98]= {{0, 0, 1}, {-√3/2, 0, -1/2}, {√3/2, 0, -1/2}}

```

```

In[99]:= col20[μ_] := CB[Position[Y20, Simplify[S2[μ] /. β → 0]][[1, 1]]]

```

```

In[100]:= Graphics[
  {Table[{Gray, Line[{e[3] + m e1 + n e2, e[4] + m e1 + n e2, e[5] + m e1 + n e2, e[6] + m e1 + n e2,
    e[3] + m e1 + n e2}], Line[{e[1] + m e1 + n e2, e[2] + m e1 + n e2,
    e[1] + (m + 1) e1 + n e2, e[2] + m e1 + (n + 1) e2, e[1] + m e1 + n e2}]}],
  {m, 1, L2}, {n, 1, L2}], Table[μ = Position[Sites, {i, m, n}][[1, 1]];
  {col20[μ], PointSize[0.03], Point[e[i] + m e1 + n e2]}, {i, 6}, {m, 1, L2}, {n, 1, L2}]]]

```

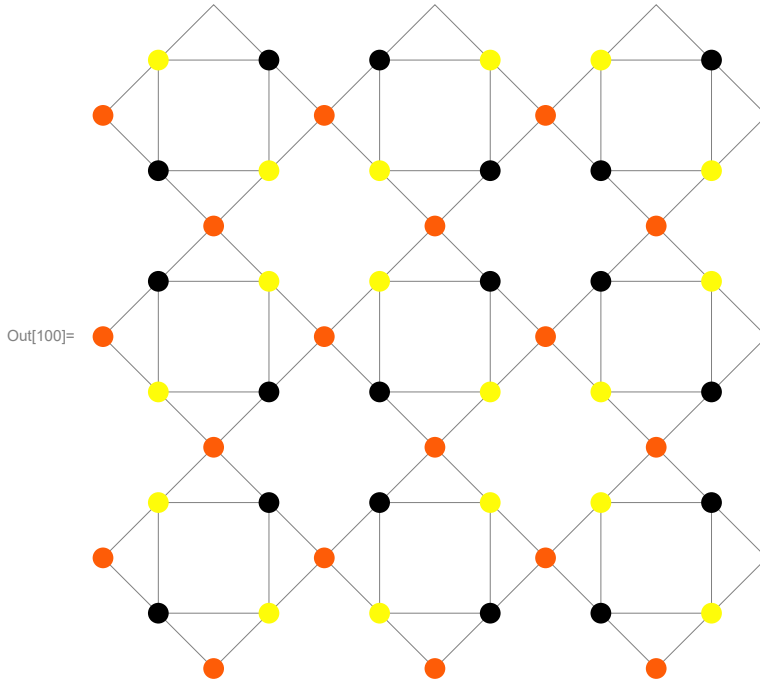

This is obviously the coplanar configuration (b) considered in the main text, Figure 8.

Next consider  $\beta \rightarrow \pi/2$ :

```

In[101]:= Y21 = Union[Simplify[Y2 /. β → π / 2]]

```

```

Out[101]= {{0, 0, 1}, {0, -√3/2, -1/2}, {0, √3/2, -1/2}}

```

```

In[102]:= col21[μ_] := CB[Position[Y21, Simplify[S2[μ] /. β → π / 2]][[1, 1]]]

```

```

In[103]:= Graphics[
  {Table[{Gray, Line[{e[3] + m e1 + n e2, e[4] + m e1 + n e2, e[5] + m e1 + n e2, e[6] + m e1 + n e2,
    e[3] + m e1 + n e2}], Line[{e[1] + m e1 + n e2, e[2] + m e1 + n e2,
    e[1] + (m + 1) e1 + n e2, e[2] + m e1 + (n + 1) e2, e[1] + m e1 + n e2}]}],
  {m, 1, L2}, {n, 1, L2}], Table[μ = Position[Sites, {i, m, n}][[1, 1]];
  {col21[μ], PointSize[0.03], Point[e[i] + m e1 + n e2]}, {i, 6}, {m, 1, L2}, {n, 1, L2}]]]

```

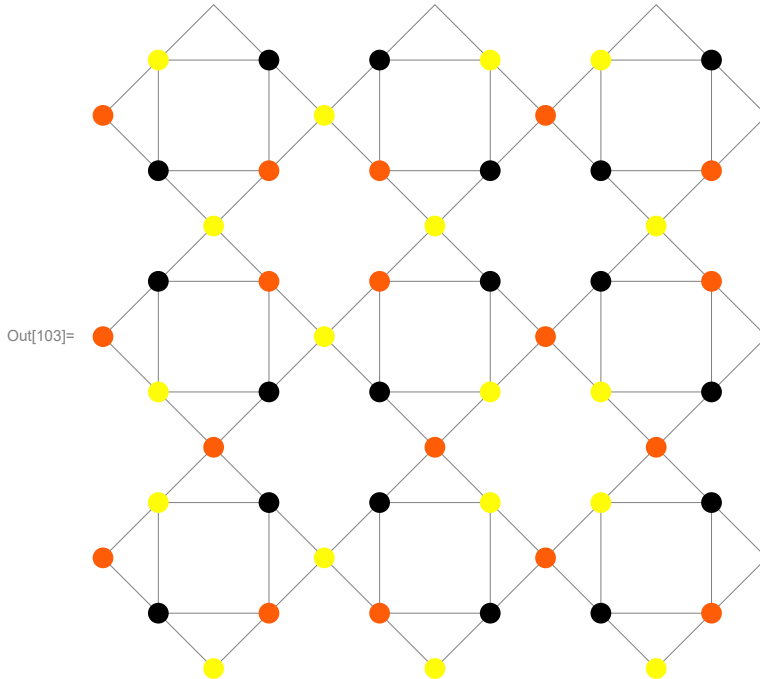

This is obviously the coplanar configuration (c) considered in the main text, Figure 8, thereby confirming the following part of the above sketch:

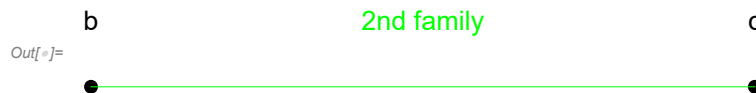

In[104]=

## Third family

Finally we consider the case of 4 different spin vectors  $(s[3], s[4], s[5], s[6]) = (\mathbf{a}, \mathbf{b}, \mathbf{c}, \mathbf{d})$  in the square of the primitive unit cell. These vectors will be defined as follows. They form a 1-parameter family depending on a parameter  $\gamma$ .

```
In[105]:= s[3] = {0, 0, 1};
s[4] = {Sqrt[3]/2 Cos[γ], Sqrt[3]/2 Sin[γ], -1/2};
s[5] = {-4 Sqrt[3] Cos[γ]/(5 + 3 Cos[2 γ]), 0, (-1 - 3 Cos[2 γ])/(5 + 3 Cos[2 γ])};
s[6] = {Sqrt[3]/2 Cos[γ], -Sqrt[3]/2 Sin[γ], -1/2};
```

This is a check that this family obeys the 120° rule:

```
In[109]:= FullSimplify[{s[3].s[4], s[4].s[5], s[5].s[6], s[6].s[3]}]
Out[109]= {-1/2, -1/2, -1/2, -1/2}
```

We show an example of the 4 spin vectors for  $\gamma = \pi/3$ :

```
In[110]:= Graphics3D[Join[Table[{CB[i + 1], Arrow[{0, 0, 0}, s[i] /. γ → π/3]}], {i, 3, 6}],
Table[Text[Style[i, 14, CB[i + 1]], 1.1 s[i] /. γ → π/3], {i, 3, 6}]]]
```

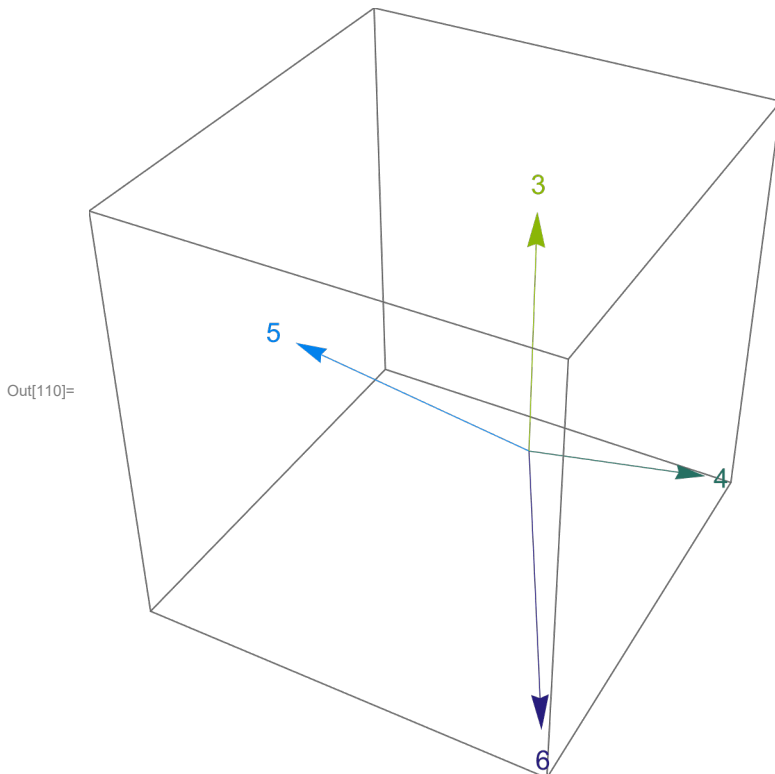

For the other unit cells the spins in the squares are defined according to the following permutations. This definition satisfies the pairing rule.

$$\rho_1 = \{1, 2, 4, 3, 6, 5\}; \rho_2 = \{1, 2, 6, 5, 4, 3\}; \rho_{12} = \{1, 2, 5, 6, 3, 4\};$$

```
In[113]:= Clear[S3]

For[i = 3, i ≤ 6, i++,
  For[m = 0, m ≤ L - 1, m++, For[n = 0, n ≤ L - 1, n++, μ = Position[Sites, {i, m, n}][[1, 1]];
    S3[μ] = Which[EvenQ[m] && EvenQ[n], s[i], OddQ[m] && EvenQ[n], s[ρ1[[i]],
      EvenQ[m] && OddQ[n], s[ρ2[[i]], OddQ[m] && OddQ[n], s[ρ12[[i]]]]]]]
```

The remaining bow tie spins are defined such that they complete 120° triangles:

```
In[115]:= For[m = 0, m ≤ L - 1, m++, For[n = 0, n ≤ L - 1, n++, μ = Position[Sites, {1, m, n}][[1, 1]];
  λ = Position[Sites, {3, m, n}][[1, 1]];
  ν = Position[Sites, {6, m, n}][[1, 1]];
  S3[μ] = Simplify[-S3[λ] - S3[ν]]]

In[116]:= For[m = 0, m ≤ L - 1, m++, For[n = 0, n ≤ L - 1, n++, μ = Position[Sites, {2, m, n}][[1, 1]];
  λ = Position[Sites, {3, m, n}][[1, 1]];
  ν = Position[Sites, {4, m, n}][[1, 1]];
  S3[μ] = Simplify[-S3[λ] - S3[ν]]]
```

The total spin configuration only uses the following 8 different spin vectors, 4 from the squares and 4 from the bow tie spins:

```
In[117]:= Y3 = Union[Table[S3[μ], {μ, NN}]];
Z3 = Table[Flatten[{CB[[i]], Y3[[i]]}], {i, 8}] // TableForm
```

Out[117]/TableForm=

|                                                                                     | 0                                                                   | 0                                    | 1                                                |
|-------------------------------------------------------------------------------------|---------------------------------------------------------------------|--------------------------------------|--------------------------------------------------|
| 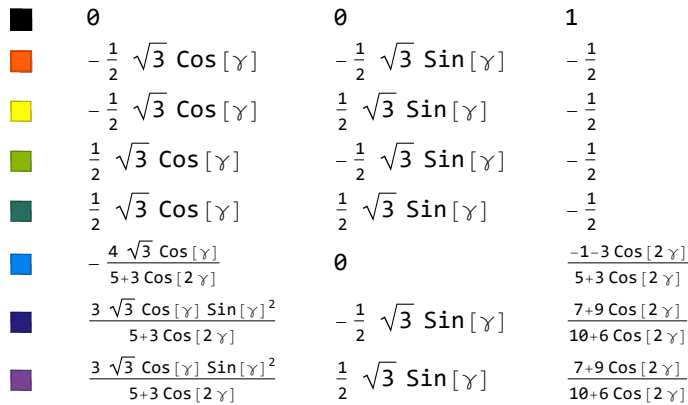 |                                                                     |                                      |                                                  |
| 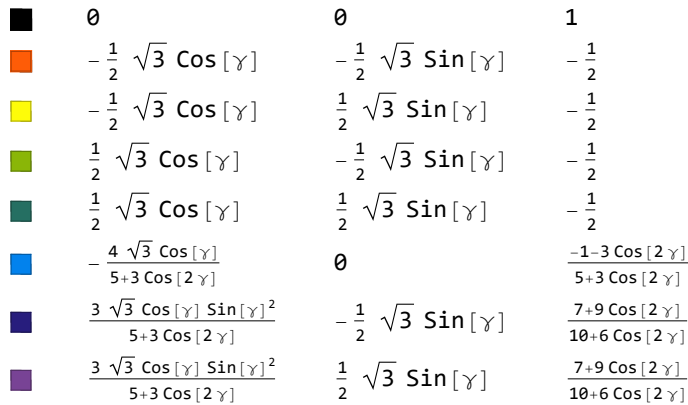 | $-\frac{1}{2} \sqrt{3} \cos[\gamma]$                                | $-\frac{1}{2} \sqrt{3} \sin[\gamma]$ | $-\frac{1}{2}$                                   |
| 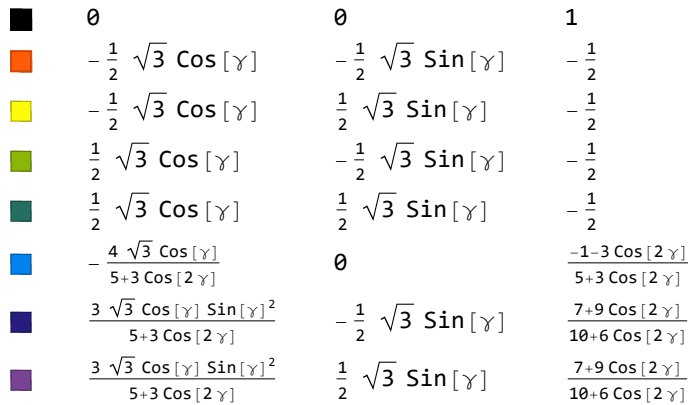 | $-\frac{1}{2} \sqrt{3} \cos[\gamma]$                                | $\frac{1}{2} \sqrt{3} \sin[\gamma]$  | $-\frac{1}{2}$                                   |
| 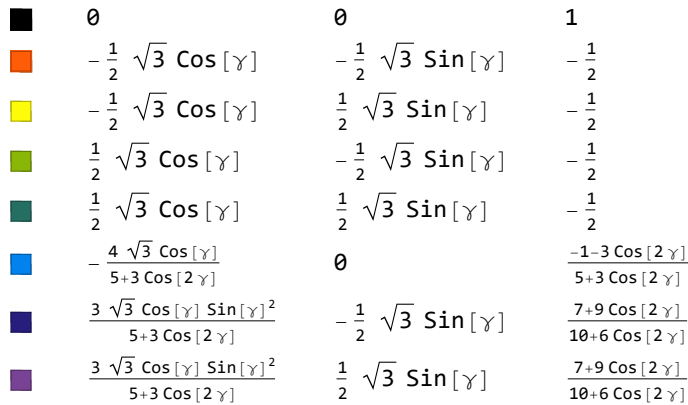 | $\frac{1}{2} \sqrt{3} \cos[\gamma]$                                 | $-\frac{1}{2} \sqrt{3} \sin[\gamma]$ | $-\frac{1}{2}$                                   |
| 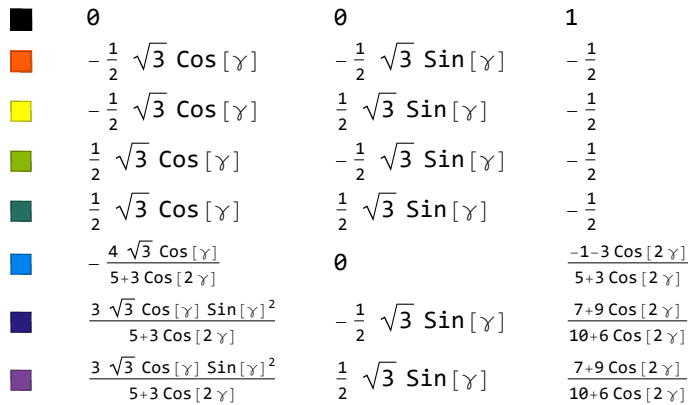 | $\frac{1}{2} \sqrt{3} \cos[\gamma]$                                 | $\frac{1}{2} \sqrt{3} \sin[\gamma]$  | $-\frac{1}{2}$                                   |
| 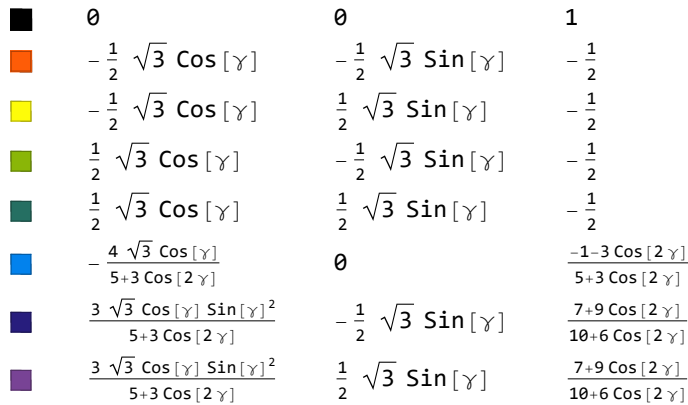 | $-\frac{4 \sqrt{3} \cos[\gamma]}{5+3 \cos[2 \gamma]}$               | 0                                    | $\frac{-1-3 \cos[2 \gamma]}{5+3 \cos[2 \gamma]}$ |
| 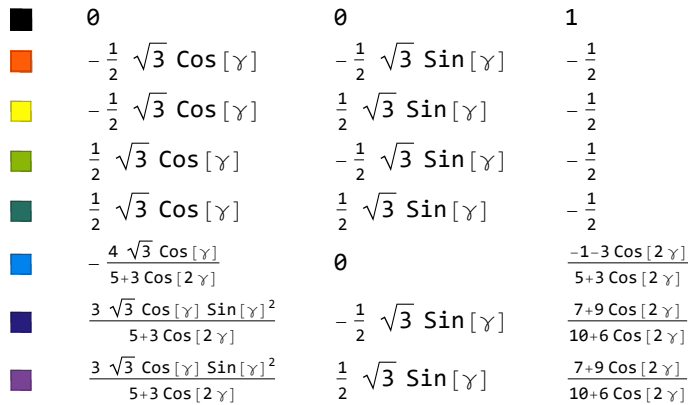 | $\frac{3 \sqrt{3} \cos[\gamma] \sin[\gamma]^2}{5+3 \cos[2 \gamma]}$ | $-\frac{1}{2} \sqrt{3} \sin[\gamma]$ | $\frac{7+9 \cos[2 \gamma]}{10+6 \cos[2 \gamma]}$ |
| 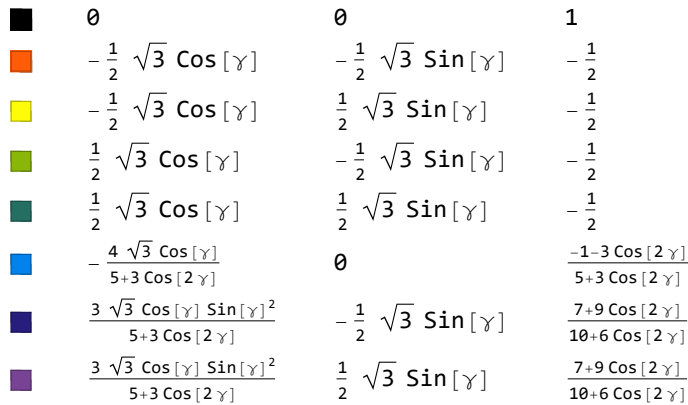 | $\frac{3 \sqrt{3} \cos[\gamma] \sin[\gamma]^2}{5+3 \cos[2 \gamma]}$ | $\frac{1}{2} \sqrt{3} \sin[\gamma]$  | $\frac{7+9 \cos[2 \gamma]}{10+6 \cos[2 \gamma]}$ |

A test follows whether the known minimal energy function

$E = \frac{1}{3} \times (-3 + Jc + Jp)$  of the coplanar  $120^\circ$  ground states is also obtained by the above defined spin configuration:

```
In[118]:= E3 = Simplify[1 / (2 NN) Sum[JA[[μ, ν]] × Simplify[S3[μ].S3[ν]], {μ, NN}, {ν, NN}]]
Out[118]=  $\frac{1}{3} \times (-3 + Jc + Jp)$ 
```

Next we produce a graphical sketch of the spin configuration by using 8 different colors:

```
In[119]:= col3[μ_] := CB[Position[Y3, S3[μ]]][1, 1]]

In[120]:= Graphics[
  {Table[{Gray, Line[{e[3] + m e1 + n e2, e[4] + m e1 + n e2, e[5] + m e1 + n e2, e[6] + m e1 + n e2,
    e[3] + m e1 + n e2}], Line[{e[1] + m e1 + n e2, e[2] + m e1 + n e2,
    e[1] + (m + 1) e1 + n e2, e[2] + m e1 + (n + 1) e2, e[1] + m e1 + n e2}]}],
  {m, 1, L2}, {n, 1, L2}], Table[μ = Position[Sites, {i, m, n}][1, 1];
  {col3[μ], PointSize[0.03], Point[e[i] + m e1 + n e2]}, {i, 6}, {m, 1, L2}, {n, 1, L2}]]]
```

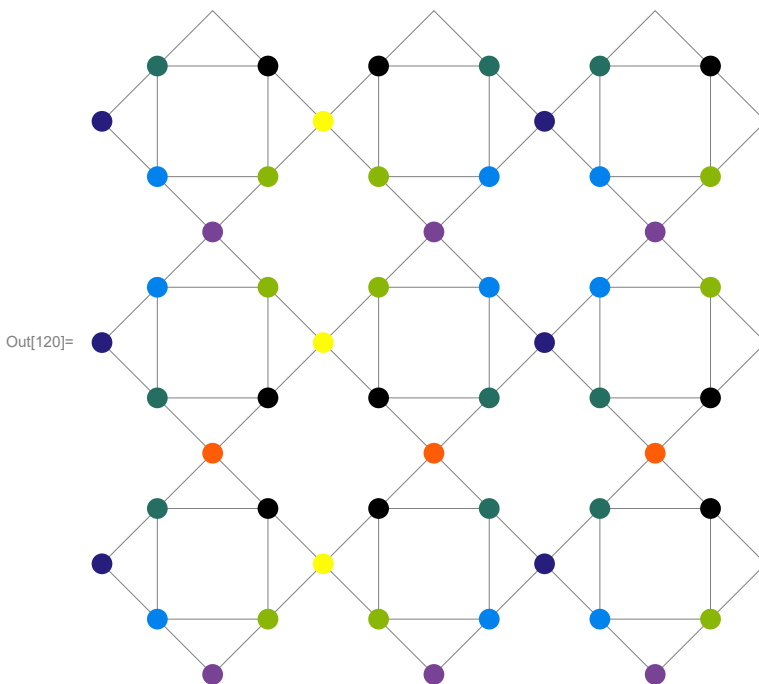

Next we consider the limit cases, first  $\gamma \rightarrow 0$ :

```
In[121]:= Y30 = Union[Simplify[Y3 /. γ → 0]]
Out[121]= {{0, 0, 1}, {-√3/2, 0, -1/2}, {√3/2, 0, -1/2}}

In[122]:= col30[μ_] := CB[Position[Y30, Simplify[S3[μ] /. γ → 0]]][1, 1]]
```



```

In[123]:= Graphics[
  {Table[{Gray, Line[{e[3] + m e1 + n e2, e[4] + m e1 + n e2, e[5] + m e1 + n e2, e[6] + m e1 + n e2,
    e[3] + m e1 + n e2}], Line[{e[1] + m e1 + n e2, e[2] + m e1 + n e2,
    e[1] + (m + 1) e1 + n e2, e[2] + m e1 + (n + 1) e2, e[1] + m e1 + n e2}]}],
  {m, 1, L2}, {n, 1, L2}], Table[μ = Position[Sites, {i, m, n}][[1, 1]];
  {col30[μ], PointSize[0.03], Point[e[i] + m e1 + n e2]}, {i, 6}, {m, 1, L2}, {n, 1, L2}]]]

```

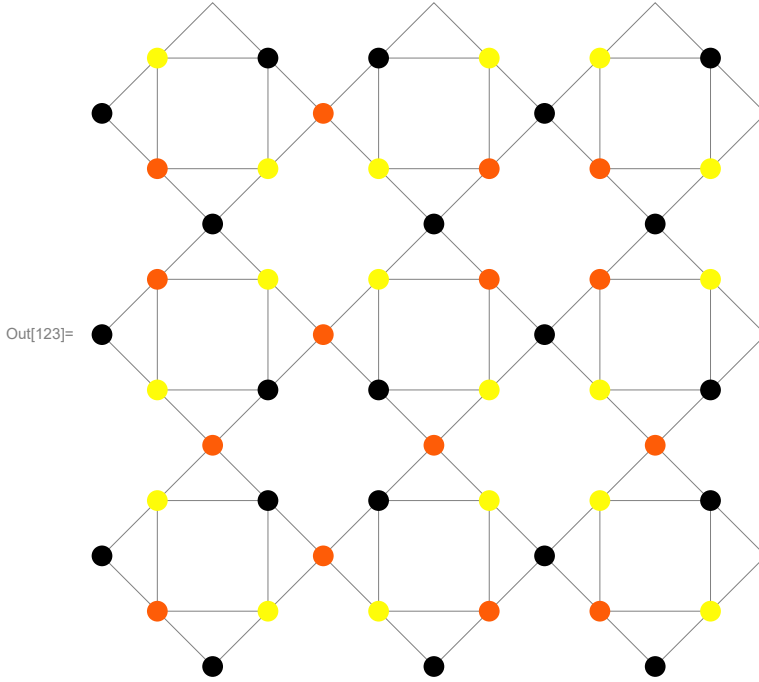

This is obviously the coplanar configuration (c) considered in the main text, Figure 8.

Next consider  $\gamma \rightarrow \pi/2$ :

```

In[124]:= Y31 = Union[Simplify[Y3 /. γ → π / 2]]

```

```

Out[124]= {{0, 0, 1}, {0, -√3/2, -1/2}, {0, √3/2, -1/2}}

```

```

In[125]:= col31[μ_] := CB[Position[Y31, Simplify[S3[μ] /. γ → π / 2]][[1, 1]]

```

```

In[126]:= Graphics[
  {Table[{Gray, Line[{e[3] + m e1 + n e2, e[4] + m e1 + n e2, e[5] + m e1 + n e2, e[6] + m e1 + n e2,
    e[3] + m e1 + n e2}], Line[{e[1] + m e1 + n e2, e[2] + m e1 + n e2,
    e[1] + (m + 1) e1 + n e2, e[2] + m e1 + (n + 1) e2, e[1] + m e1 + n e2}]}],
  {m, 1, L2}, {n, 1, L2}], Table[μ = Position[Sites, {i, m, n}][[1, 1]];
  {col31[μ], PointSize[0.03], Point[e[i] + m e1 + n e2]}, {i, 6}, {m, 1, L2}, {n, 1, L2}]]]

```

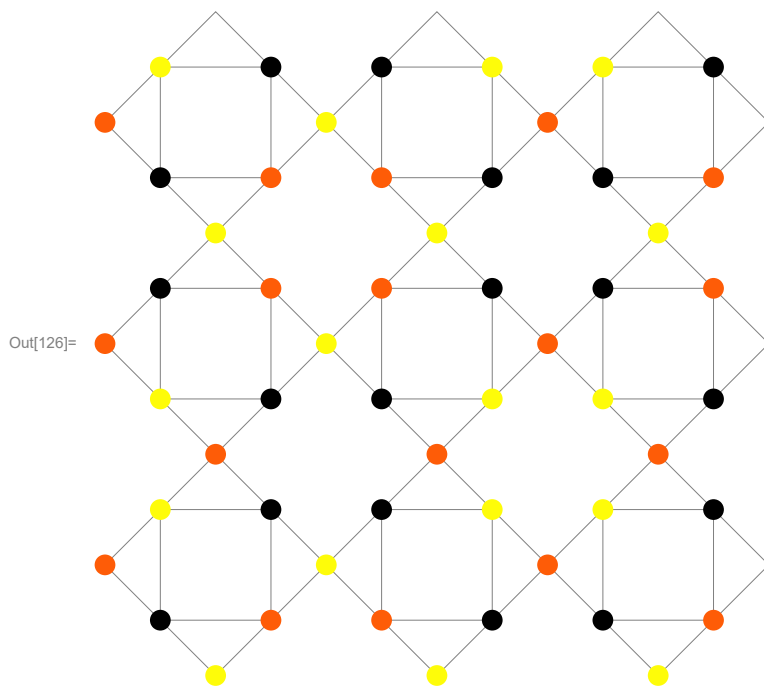

This is again the coplanar configuration (c) resulting from the previous one by a left translation and the permutation of colors  $\{\blacksquare \leftrightarrow \text{yellow square}\}$ . This confirms the remaining part of the above sketch:

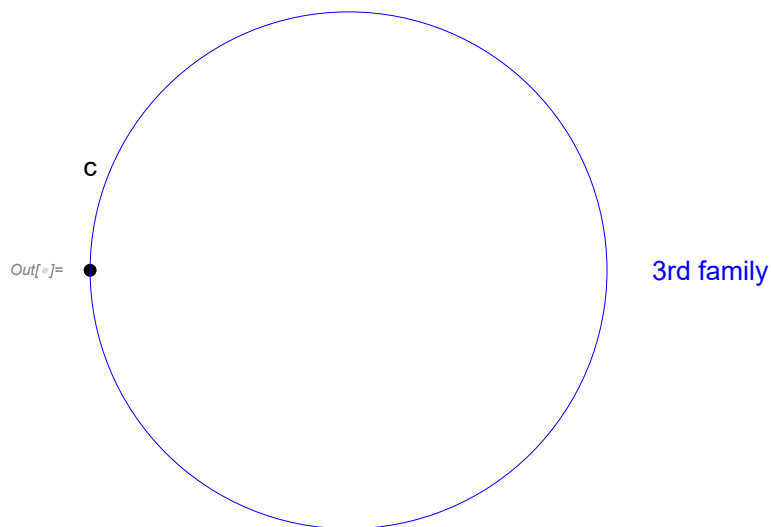

```

In[127]:=

```

## Phase VII (deformed 120° ground states)

We will describe a 1-parameter family of generally non-coplanar spin configurations that generalize the deformed 120° ground states described in the manuscript and have the same energy.

First consider the following 5 spin vectors depending on  $J_c$  and a parameter  $\alpha$ , encoded by the colors {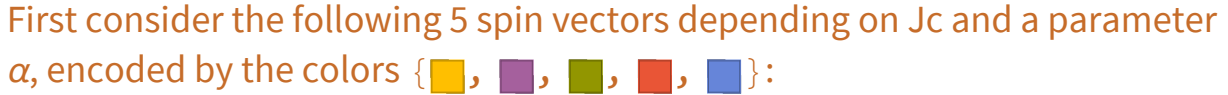, 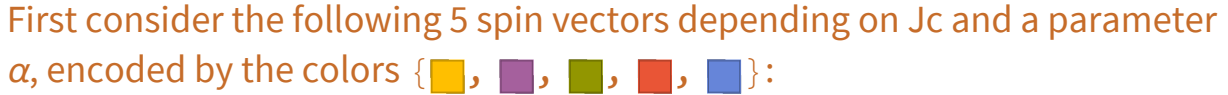, 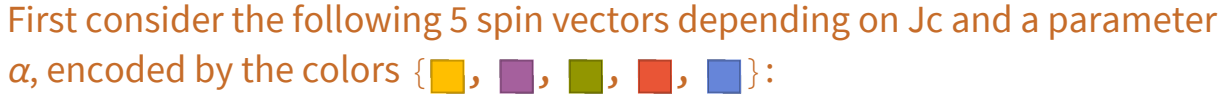, 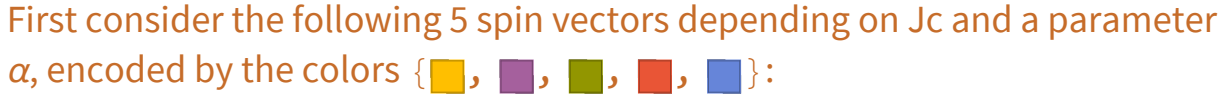, 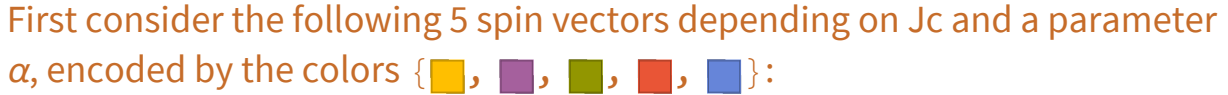}:

```
In[128]:= CD = {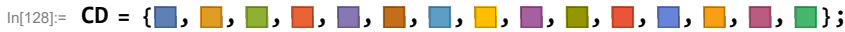, 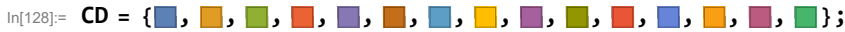, 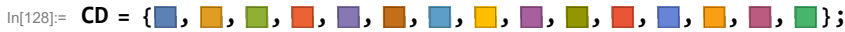, 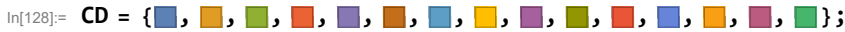, 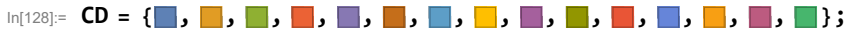, 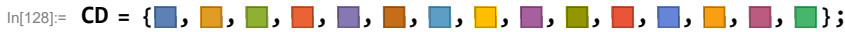, 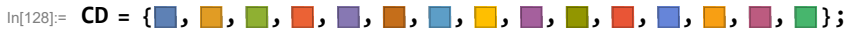, 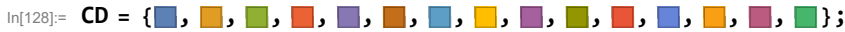, 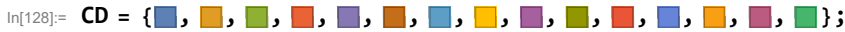, 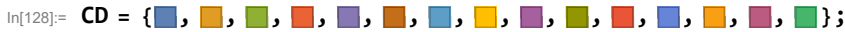, 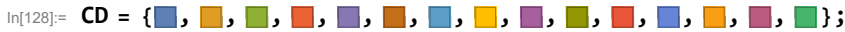, 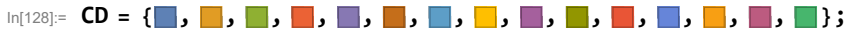, 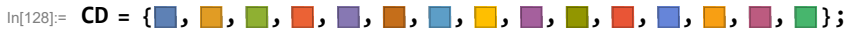, 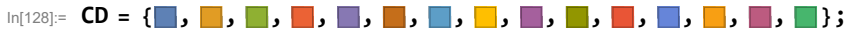, 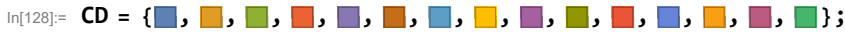};
```

```
In[129]:= SZ = { {-1, 0, 0}, { $\frac{1}{2+J_c}$ ,  $-\frac{\sqrt{3+4J_c+J_c^2}}{2+J_c}$ , 0}, { $\frac{1}{2+J_c}$ ,  $\frac{\sqrt{3+4J_c+J_c^2}}{2+J_c}$ , 0},  

{ $\frac{1}{2+J_c}$ ,  $-\frac{\sqrt{3+4J_c+J_c^2} \cos[\alpha]}{2+J_c}$ ,  $\frac{\sqrt{3+4J_c+J_c^2} \sin[\alpha]}{2+J_c}$ },  

{ $\frac{1}{2+J_c}$ ,  $\frac{\sqrt{3+4J_c+J_c^2} \cos[\alpha]}{2+J_c}$ ,  $-\frac{\sqrt{3+4J_c+J_c^2} \sin[\alpha]}{2+J_c}$ }};
```

```
In[130]:= SF = Table[Flatten[{CD[[i+7]], SZ[[i]]}], {i, 5}]; SF // TableForm
```

```
Out[130]//TableForm=
```

|                                                                                     |                   |                                                   |                                                   |
|-------------------------------------------------------------------------------------|-------------------|---------------------------------------------------|---------------------------------------------------|
| 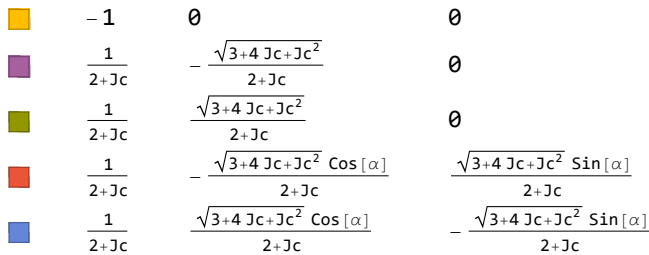 | -1                | 0                                                 | 0                                                 |
| 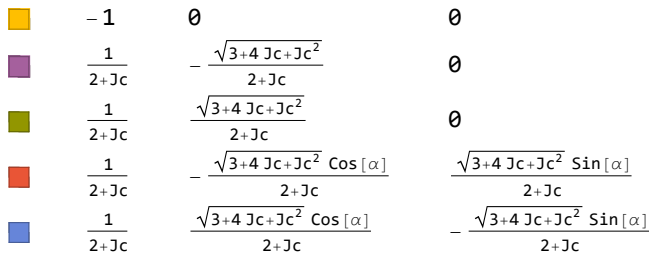 | $\frac{1}{2+J_c}$ | $-\frac{\sqrt{3+4J_c+J_c^2}}{2+J_c}$              | 0                                                 |
| 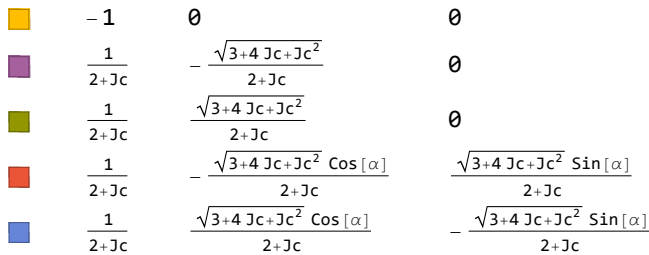 | $\frac{1}{2+J_c}$ | $\frac{\sqrt{3+4J_c+J_c^2}}{2+J_c}$               | 0                                                 |
| 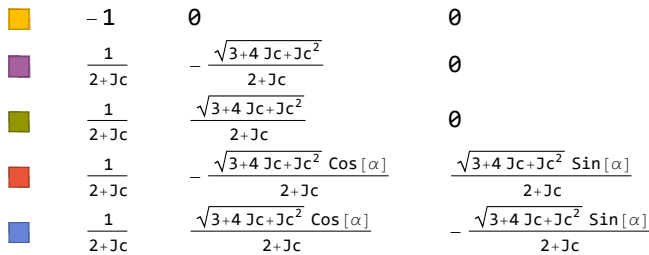 | $\frac{1}{2+J_c}$ | $-\frac{\sqrt{3+4J_c+J_c^2} \cos[\alpha]}{2+J_c}$ | $\frac{\sqrt{3+4J_c+J_c^2} \sin[\alpha]}{2+J_c}$  |
| 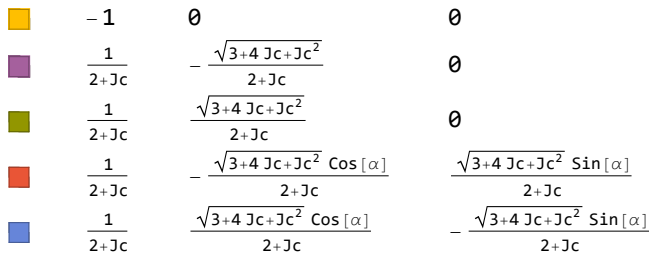 | $\frac{1}{2+J_c}$ | $\frac{\sqrt{3+4J_c+J_c^2} \cos[\alpha]}{2+J_c}$  | $-\frac{\sqrt{3+4J_c+J_c^2} \sin[\alpha]}{2+J_c}$ |

We define the following spin configuration  $S[\mu]$  with a magnetic unit cell of size  $2 \times 2$ :

```
In[131]:= Clear[S]
```

```
In[132]:= For[μ = 1, μ ≤ NN, μ++, {i, m, n} = Sites[μ];  

S[μ] = Which[i == 1 || i == 2, SZ[[1]], (i == 3 || i == 5) && EvenQ[m] && EvenQ[n], SZ[[3]],  

(i == 4 || i == 6) && EvenQ[m] && EvenQ[n], SZ[[2]], (i == 3 || i == 5) && OddQ[m] && OddQ[n],  

SZ[[2]], (i == 4 || i == 6) && OddQ[m] && OddQ[n], SZ[[3]], (i == 3 || i == 5) && OddQ[m] &&  

EvenQ[n], SZ[[4]], (i == 3 || i == 5) && EvenQ[m] && OddQ[n], SZ[[5]], (i == 4 || i == 6) &&  

OddQ[m] && EvenQ[n], SZ[[5]], (i == 4 || i == 6) && EvenQ[m] && OddQ[n], SZ[[4]]];
```

It can be visualized as follows:

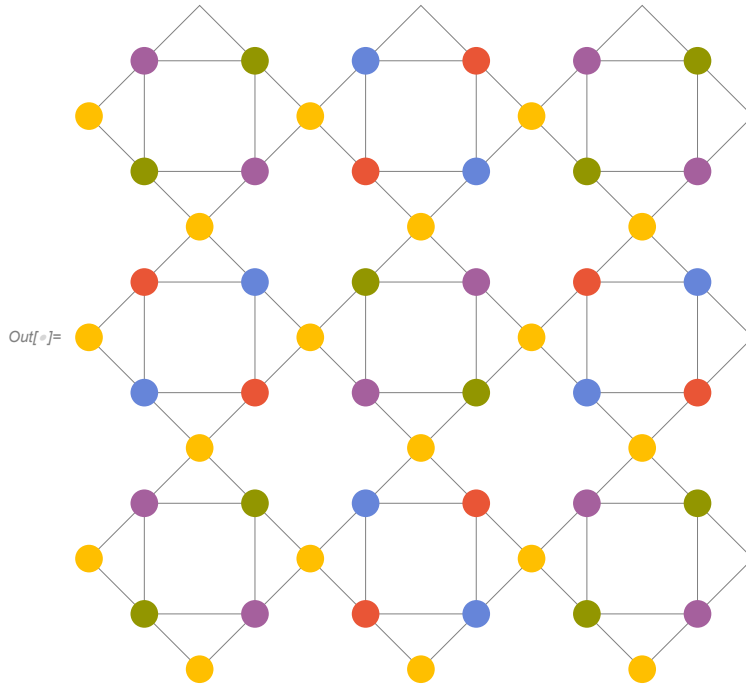

Its energy  $E7$  coincides with the energy  $E_{120^\circ-d}$  calculated in the manuscript for the deformed  $120^\circ$  ground state. Hence this spin configuration represents a ground state in the domain of phase VII.

$$\text{In}[133]:= \mathbf{E7} = \mathbf{FullSimplify}\left[\frac{1}{2 \text{NN}} \text{Sum}[\text{Simplify}[\mathbf{JA}[\mu, \nu] \times \mathbf{S}[\mu] \cdot \mathbf{S}[\nu]], \{\mu, \text{NN}\}, \{\nu, \text{NN}\}]\right]$$

$$\text{Out}[133]= \frac{1}{3} \times \left(-2 - \text{Jc} - \frac{2}{2 + \text{Jc}} + \text{Jp}\right)$$

$$\text{In}[134]:= \mathbf{Simplify}\left[\mathbf{E7} == -\frac{6 + \text{Jc}^2 - \text{Jc}(-4 + \text{Jp}) - 2 \text{Jp}}{3 \times (2 + \text{Jc})}\right]$$

$$\text{Out}[134]= \text{True}$$

In general the dimension of the ground state is 3, the matrix rank of SZ. We show an example for  $\alpha=\pi/2$ :

```
In[135]:= Graphics3D[
  {Table[{CD[[i + 7]], Thick, Arrow[{0, 0, 0}, SZ[[i]] /. Jc -> 1 / 5 /.  $\alpha \rightarrow \pi / 2$ ]}, {i, 5}],
  Table[Text[Style[i, CD[[i + 7]], 18], 1.1 SZ[[i]] /. Jc -> 1 / 5 /.  $\alpha \rightarrow \pi / 2$ ], {i, 5}],
  Opacity[0.2], Sphere[], Boxed -> False]
```

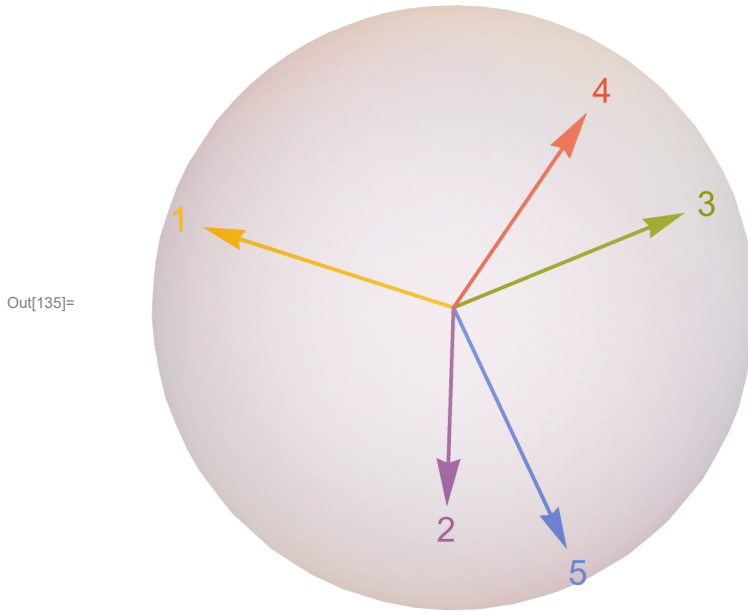

```
In[136]:= MatrixRank[SZ]
```

Out[136]= 3

However, for the special values of  $\alpha=0$  and  $\alpha=\pi$  its dimension is reduced to 2. These two configurations can be identified with the coplanar deformed  $120^\circ$  ground state described in the main text which has only 3 different spin vectors.

```
In[137]:= MatrixRank[SZ /.  $\alpha \rightarrow 0$ ]
```

Out[137]= 2

```
In[138]:= MatrixRank[SZ /.  $\alpha \rightarrow \pi$ ]
```

Out[138]= 2

```
In[139]:= Graphics3D[
  {Table[{CD[[i + 7]], Thick, Arrow[{0, 0, 0}, SZ[[i]] /. Jc -> 1 / 5 /.  $\alpha$  -> 0]}], {i, 5}},
  Opacity[0.2], Sphere[], Boxed -> False]
```

Out[139]=

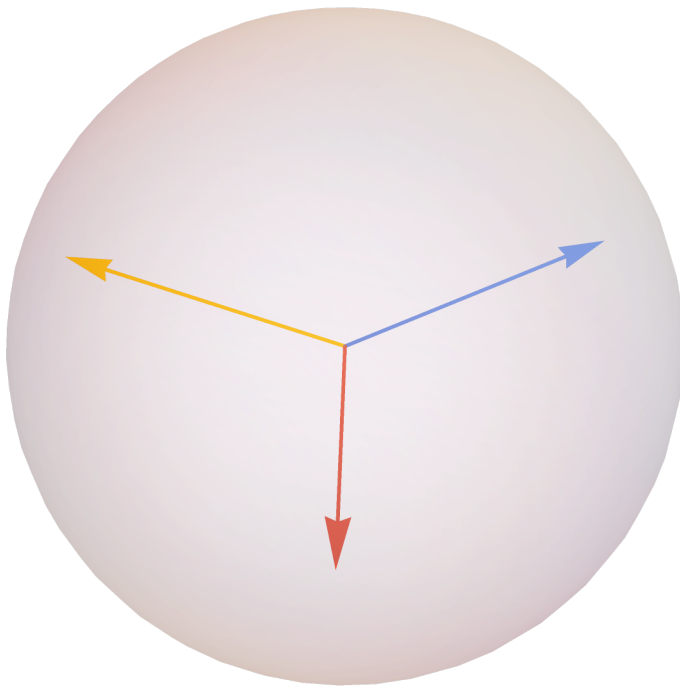

```
In[140]:= Graphics3D[
  {Table[{CD[[i + 7]], Thick, Arrow[{0, 0, 0}, SZ[[i]] /. Jc -> 1 / 5 /.  $\alpha$  ->  $\pi$ ]}], {i, 5}},
  Opacity[0.2], Sphere[], Boxed -> False]
```

Out[140]=

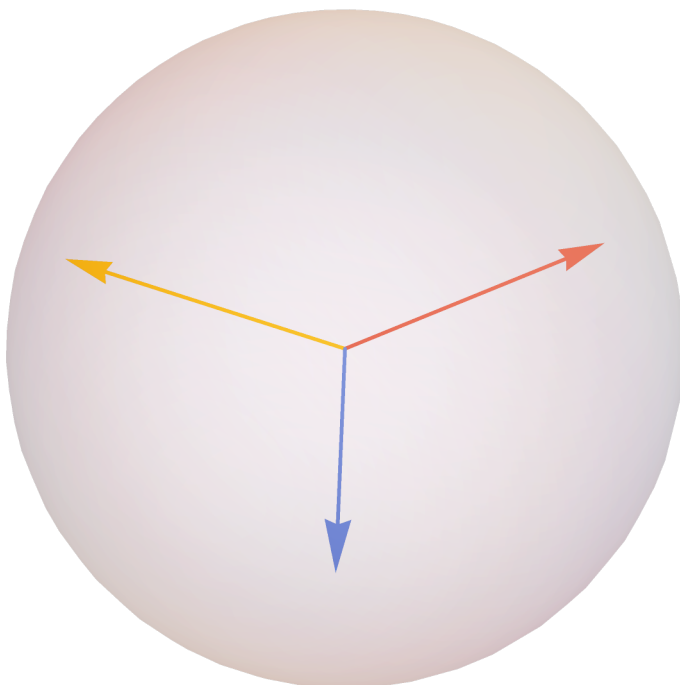

Supplement: Supplementary file 2 [file NonCoplanar_120.pdf]
