# Supplementary material for: Non-Coplanar Magnetic Orders in Classical Square-Kagome Antiferromagnets
Source: arXiv:2302.04171 ancillary file (2023-11-30)

# Semi-analytical description of the spiral phases V , IV, and IX

## Square kagome, $J_1=J_2=J_3=1$

We consider a finite model of the square kagome lattice consisting of  $12 \times 12$  unit cells with 6 spins and represent each spin site by the multi-indices  $\{i, m, n\}$  such that  $i=1,2,3,4,5,6$  and  $m, n=0, \dots, 11 \bmod 12$ . “Sites” is the list of all spin sites.

It has the length  $NN=6 \times 12 \times 12=864$ .

The number  $\text{pos}[i, m, n]$  is the position of the spin site  $\{i, m, n\}$  within “Sites”.

```
In[1]:= L = 12;
In[2]:= Sites = Flatten[Table[{i, m, n}, {i, 6}, {m, 0, L - 1}, {n, 0, L - 1}], 2];
In[3]:= NN = Length[Sites]
Out[3]= 864
In[4]:= For[i = 1, i <= 6, i++, For[m = 0, m <= 11, m++,
    For[n = 0, n <= 11, n++, pos[i, m, n] = Position[Sites, {i, m, n}][[1, 1]]]]]
```

Next we define the J-matrix of the square kagome model with arbitrary coupling constants

$J_1, J_2, J_3, J_p, J_c$  (note that we avoid subscripts in the variables and have set  $J_p \equiv J_+$  and  $J_c \equiv J_x$ ):

```
In[5]:= J = Table[0, {NN}, {NN}];
```

```

In[6]:= For[μ = 1, μ <= NN, μ++, {i1, n1, m1} = Sites[μ]];
For[ν = 1, ν <= NN, ν++, {i2, n2, m2} = Sites[ν]];
If[n1 == n2 && m1 == m2, If[Sort[{i1, i2}] == {3, 4} || Sort[{i1, i2}] == {4, 5} ||
Sort[{i1, i2}] == {5, 6} || Sort[{i1, i2}] == {3, 6}, J[[μ, ν]] = J[[ν, μ]] = J1]];
If[n1 == n2 && m1 == m2, If[Sort[{i1, i2}] == {1, 3} || Sort[{i1, i2}] == {2, 4},
J[[μ, ν]] = J[[ν, μ]] = J2]];
If[n1 == n2 && m1 == m2, If[Sort[{i1, i2}] == {1, 6} || Sort[{i1, i2}] == {2, 3},
J[[μ, ν]] = J[[ν, μ]] = J3]];
If[Mod[n1 - 1 - n2, L] == 0 && m1 == m2,
If[{i1, i2} == {1, 5}, J[[μ, ν]] = J[[ν, μ]] = J2]];
If[Mod[n1 - 1 - n2, L] == 0 && m1 == m2,
If[{i1, i2} == {1, 4}, J[[μ, ν]] = J[[ν, μ]] = J3]];
If[Mod[n1 - 1 - n2, L] == 0 && m1 == m2,
If[{i1, i2} == {2, 2}, J[[μ, ν]] = J[[ν, μ]] = Jp]];
If[Mod[n1 + 1 - n2, L] == 0 && m1 == m2,
If[{i1, i2} == {2, 2}, J[[μ, ν]] = J[[ν, μ]] = Jp]];
If[Mod[m1 - 1 - m2, L] == 0 && n1 == n2,
If[{i1, i2} == {2, 6}, J[[μ, ν]] = J[[ν, μ]] = J2]];
If[Mod[m1 - 1 - m2, L] == 0 && n1 == n2,
If[{i1, i2} == {2, 5}, J[[μ, ν]] = J[[ν, μ]] = J3]];
If[Mod[m1 - 1 - m2, L] == 0 && n1 == n2,
If[{i1, i2} == {1, 1}, J[[μ, ν]] = J[[ν, μ]] = Jp]];
If[Mod[m1 + 1 - m2, L] == 0 && n1 == n2,
If[{i1, i2} == {1, 1}, J[[μ, ν]] = J[[ν, μ]] = Jp]];
If[Mod[m1 - 1 - m2, L] == 0 && Mod[n1 - 1 - n2, L] == 0,
If[{i1, i2} == {3, 5}, J[[μ, ν]] = J[[ν, μ]] = Jc]];
If[Mod[m1 + 1 - m2, L] == 0 && Mod[n1 - 1 - n2, L] == 0,
If[{i1, i2} == {6, 4}, J[[μ, ν]] = J[[ν, μ]] = Jc]];
If[Mod[m1 - 1 - m2, L] == 0 && Mod[n1 + 1 - n2, L] == 0,
If[{i1, i2} == {4, 6}, J[[μ, ν]] = J[[ν, μ]] = Jc]];
If[Mod[m1 + 1 - m2, L] == 0 && Mod[n1 + 1 - n2, L] == 0,
If[{i1, i2} == {5, 3}, J[[μ, ν]] = J[[ν, μ]] = Jc]]];

```

## Phase V

We consider the specialization JA to the values

$$\{J_1 \rightarrow 1, J_2 \rightarrow 1, J_3 \rightarrow 1, J_p \rightarrow \frac{1}{5}, J_c \rightarrow -1\}$$

corresponding to a point in the  $(J_p, J_c)$ -plane where we have observed ground states of phase V.

```
In[7]:= val = {J1 -> 1, J2 -> 1, J3 -> 1, Jp -> 1/5, Jc -> -1}
```

```
Out[7]= {J1 -> 1, J2 -> 1, J3 -> 1, Jp -> 1/5, Jc -> -1}
```

```
In[8]:= JA = Simplify[J /. val];
```

Next, we import the result of a Monte Carlo calculation of the ground state for the square Kagome lattice and the coupling values “val”. We represent the numerical spin vectors  $r[[\mu]]$  of the ground state in the order defined above, which corresponds to the order of the multi-indices  $\{i, m, n\}$  in the list “Sites”.

```
In[9]:= r = {{0.96511, 0.031637, 0.25992}, {-0.5507, -0.82679, 0.11462},
  {-0.43973, 0.87116, -0.21843}, {0.99675, -0.064729, 0.048018},
  {-0.56896, -0.81354, 0.12015}, {-0.4016, 0.9149, -0.040922},
  {0.94549, -0.18761, -0.26617}, {-0.5323, -0.66103, 0.52886},
  {-0.44166, 0.7882, -0.42858}, {0.98948, -0.11165, -0.092003},
  {-0.51884, -0.67406, 0.52578}, {-0.44111, 0.6966, -0.56583},
  {-0.42998, 0.66711, -0.60834}, {0.96761, 0.04779, 0.24789},
  {-0.5595, -0.8177, 0.1354}, {-0.44877, 0.86202, -0.23566},
  {0.99733, -0.052751, 0.050492}, {-0.55982, -0.81779, 0.13345},
  {-0.41763, 0.90642, -0.063133}, {0.92806, -0.18953, -0.32059},
  {-0.52416, -0.63707, 0.56515}, {-0.45616, 0.77462, -0.43805},
  {0.98917, -0.096099, -0.11096}, {-0.52524, -0.65199, 0.54684},
  {-0.5312, -0.64541, 0.54888}, {-0.4459, 0.6843, -0.57698},
  {0.96979, 0.030402, 0.24202}, {-0.55314, -0.82367, 0.12493},
  {-0.44362, 0.87103, -0.21097}, {0.99786, -0.065351, 0.0033689},
  {-0.551, -0.81667, 0.1716}, {-0.39185, 0.91991, -0.014627},
  {0.91832, -0.2076, -0.33702}, {-0.5253, -0.63223, 0.56952},
  {-0.43985, 0.78699, -0.43265}, {0.98548, -0.13112, -0.10787},
  {0.9896, -0.11503, -0.086391}, {-0.53633, -0.66129, 0.52445},
  {-0.44039, 0.68078, -0.58532}, {0.96348, 0.042942, 0.26433},
```

```

{-0.56285, -0.81743, 0.12256}, {-0.42658, 0.88767, -0.17345},
{0.99619, -0.086393, -0.012146}, {-0.55639, -0.81859, 0.1426},
{-0.38847, 0.92142, -0.0084181}, {0.93241, -0.19814, -0.30225},
{-0.52981, -0.6311, 0.56658}, {-0.43193, 0.78914, -0.43668},
{-0.43981, 0.77406, -0.45541}, {0.99514, -0.08766, -0.044859},
{-0.53365, -0.67115, 0.51457}, {-0.43574, 0.67658, -0.59361},
{0.95852, 0.055723, 0.27952}, {-0.56032, -0.82245, 0.098066},
{-0.39866, 0.89628, -0.19432}, {0.99518, -0.097649, -0.0089299},
{-0.55963, -0.80467, 0.19831}, {-0.39394, 0.91833, -0.038441},
{0.91046, -0.22976, -0.3439}, {-0.52297, -0.61199, 0.59327},
{-0.52601, -0.59473, 0.60795}, {-0.42234, 0.75947, -0.49481},
{0.99479, -0.099372, -0.022713}, {-0.54967, -0.65404, 0.5197},
{-0.41621, 0.68264, -0.60064}, {0.95592, 0.033798, 0.29169},
{-0.56446, -0.82343, 0.057901}, {-0.39604, 0.90165, -0.17371},
{0.99247, -0.12006, -0.024275}, {-0.56607, -0.80233, 0.1893},
{-0.38377, 0.92333, -0.013432}, {0.90434, -0.22607, -0.36202},
{0.90979, -0.22259, -0.35034}, {-0.52014, -0.59973, 0.6081},
{-0.43766, 0.76453, -0.47323}, {0.99211, -0.11999, -0.036259},
{-0.56723, -0.63876, 0.51983}, {-0.4149, 0.70066, -0.58046},
{0.96566, -0.010028, 0.25963}, {-0.58464, -0.80478, 0.10256},
{-0.40186, 0.90193, -0.15817}, {0.99323, -0.10289, -0.053849},
{-0.57509, -0.7881, 0.21945}, {-0.38054, 0.92449, -0.022543},
{-0.37515, 0.92614, -0.039052}, {0.92624, -0.21887, -0.30687},
{-0.54086, -0.62691, 0.56076}, {-0.4266, 0.79282, -0.43525},
{0.98924, -0.1412, -0.038352}, {-0.55969, -0.66099, 0.49984},
{-0.44192, 0.73894, -0.5086}, {0.97691, -0.013039, 0.21326},
{-0.58448, -0.80168, 0.12524}, {-0.39826, 0.90238, -0.16464},
{0.99165, -0.10844, -0.06975}, {-0.5726, -0.7919, 0.21218},
{-0.57262, -0.79663, 0.19365}, {-0.38336, 0.92167, -0.059712},
{0.92605, -0.21669, -0.30901}, {-0.5371, -0.62328, 0.56837},
{-0.41114, 0.80793, -0.42216}, {0.99491, -0.092937, -0.039029},
{-0.53311, -0.70164, 0.47275}, {-0.44795, 0.7343, -0.51004},
{0.97776, 0.0052497, 0.20965}, {-0.55563, -0.82911, 0.062049},
{-0.41542, 0.89978, -0.13348}, {0.99379, -0.098018, -0.052593},
{0.99491, -0.10077, -0.00041865}, {-0.57018, -0.8072, 0.1527},
{-0.39681, 0.91655, -0.0497}, {0.92682, -0.2193, -0.30483},
{-0.54812, -0.63004, 0.5501}, {-0.4283, 0.80105, -0.41819},
{0.99464, -0.097788, -0.033615}, {-0.52604, -0.7094, 0.46908},
{-0.44451, 0.72113, -0.53139}, {0.9672, 0.02626, 0.25264},
{-0.53773, -0.83935, 0.079569}, {-0.42764, 0.88682, -0.17512},
{-0.4169, 0.88094, -0.22391}, {0.99745, -0.071148, -0.0053479},
{-0.55812, -0.81515, 0.15502}, {-0.39583, 0.9172, -0.045493},
{0.93075, -0.21273, -0.29739}, {-0.54377, -0.63039, 0.554},
{-0.44002, 0.80097, -0.406}, {0.98854, -0.12631, -0.08273},
{-0.53344, -0.6613, 0.52736}, {-0.45059, 0.69927, -0.55496},
{0.97808, 0.0083597, 0.20806}, {-0.57147, -0.81015, 0.13069},
{-0.57392, -0.80751, 0.13618}, {-0.43149, 0.87792, -0.20754},
{0.99738, -0.068841, 0.022079}, {-0.55559, -0.82009, 0.13702},
{-0.39428, 0.91862, -0.026081}, {0.93688, -0.19289, -0.29163},
{-0.53353, -0.65015, 0.54097}, {-0.42323, 0.81478, -0.39625},

```

```

{0.98685, -0.13162, -0.093829}, {-0.51989, -0.66247, 0.5393},
{-0.44808, 0.70634, -0.54801}, {0.97851, 0.01178, 0.20588},
{-0.43227, 0.70914, -0.55701}, {0.9766, 0.010874, 0.21478},
{-0.55848, -0.81463, 0.15645}, {-0.43163, 0.87351, -0.22512},
{0.9979, -0.045264, 0.046402}, {-0.55793, -0.81778, 0.14124},
{-0.39359, 0.91913, -0.016718}, {0.92511, -0.19259, -0.32723},
{-0.53788, -0.65054, 0.53617}, {-0.43259, 0.80983, -0.39629},
{0.98224, -0.14709, -0.11646}, {-0.52233, -0.64294, 0.56018},
{-0.5175, -0.65281, 0.5532}, {-0.43245, 0.68251, -0.5892},
{0.96068, 0.05405, 0.27236}, {-0.54171, -0.83448, 0.10093},
{-0.43631, 0.87669, -0.2026}, {0.99825, -0.058836, 0.0056186},
{-0.55438, -0.82359, 0.11987}, {-0.40842, 0.91264, -0.016805},
{0.92824, -0.20075, -0.31316}, {-0.52747, -0.64489, 0.55308},
{-0.44216, 0.78986, -0.42499}, {0.98673, -0.11922, -0.11024},
{0.98717, -0.13152, -0.090493}, {-0.54414, -0.62546, 0.5592},
{-0.42133, 0.66121, -0.62072}, {0.95574, 0.05647, 0.28875},
{-0.5461, -0.83074, 0.10793}, {-0.43126, 0.87277, -0.22866},
{0.99685, -0.078288, 0.012615}, {-0.56009, -0.81641, 0.14058},
{-0.40315, 0.91513, 0.0036225}, {0.91056, -0.21423, -0.35352},
{-0.49994, -0.61115, 0.61364}, {-0.45965, 0.7646, -0.45178},
{-0.4449, 0.77145, -0.4549}, {0.99131, -0.10459, -0.079777},
{-0.54999, -0.63581, 0.54153}, {-0.42571, 0.66222, -0.61664},
{0.95644, 0.060371, 0.28561}, {-0.56357, -0.81924, 0.10598},
{-0.40502, 0.89263, -0.19793}, {0.99544, -0.095398, -0.00014956},
{-0.5796, -0.80353, 0.13567}, {-0.35984, 0.93145, 0.054031},
{0.89656, -0.23732, -0.37398}, {-0.51774, -0.60078, 0.6091},
{-0.50903, -0.60109, 0.6161}, {-0.44337, 0.76533, -0.46657},
{0.99342, -0.10363, -0.048751}, {-0.5325, -0.66657, 0.52166},
{-0.43596, 0.67583, -0.59431}, {0.96309, 0.036525, 0.26669},
{-0.56393, -0.82353, 0.061525}, {-0.39648, 0.8959, -0.20043},
{0.99342, -0.11448, 0.0020312}, {-0.57477, -0.80269, 0.15916},
{-0.36916, 0.92936, -0.0019}, {0.89784, -0.2418, -0.36798},
{0.91185, -0.21166, -0.35176}, {-0.53277, -0.60581, 0.59089},
{-0.42781, 0.77838, -0.45945}, {0.99587, -0.087218, -0.02506},
{-0.532, -0.6879, 0.49372}, {-0.4279, 0.72057, -0.54561},
{0.96234, 0.014865, 0.27145}, {-0.58279, -0.80986, 0.066987},
{-0.41868, 0.90102, -0.11344}, {0.99255, -0.093234, -0.078455},
{-0.56464, -0.79397, 0.22537}, {-0.38579, 0.92115, -0.051393},
{-0.4041, 0.91206, -0.06965}, {0.93442, -0.20168, -0.29355},
{-0.53879, -0.61028, 0.58075}, {-0.42284, 0.76639, -0.48358},
{0.99702, -0.076625, -0.0091079}, {-0.56579, -0.67547, 0.47289},
{-0.42396, 0.72711, -0.53997}, {0.95826, 0.027693, 0.28454},
{-0.55881, -0.82852, 0.03588}, {-0.4166, 0.90478, -0.088427},
{0.98917, -0.10531, -0.10227}, {-0.54832, -0.79324, 0.2648},
{-0.57183, -0.79094, 0.21777}, {-0.3923, 0.91788, -0.060028},
{0.92507, -0.21862, -0.31057}, {-0.54282, -0.62307, 0.56314},
{-0.41728, 0.79525, -0.43983}, {0.99098, -0.12681, -0.043424},
{-0.54816, -0.65679, 0.51783}, {-0.41593, 0.70216, -0.57791},
{0.96497, 0.020007, 0.26158}, {-0.56082, -0.82556, 0.062738},
{-0.40952, 0.89975, -0.15081}, {0.99169, -0.1144, -0.058838},

```

```

{0.99388, -0.10962, -0.013695}, {-0.57491, -0.79928, 0.17499},
{-0.42182, 0.90126, -0.098998}, {0.93661, -0.20845, -0.28164},
{-0.55031, -0.63777, 0.5389}, {-0.42406, 0.80934, -0.40638},
{0.99227, -0.10885, -0.059518}, {-0.54137, -0.68585, 0.48634},
{-0.45267, 0.72199, -0.52328}, {0.98319, 0.0050617, 0.18251},
{-0.58112, -0.79925, 0.15333}, {-0.40489, 0.89213, -0.20039},
{-0.41742, 0.88869, -0.18971}, {0.99602, -0.086773, -0.020454},
{-0.5598, -0.80802, 0.18366}, {-0.40925, 0.91019, -0.063842},
{0.9435, -0.20522, -0.26016}, {-0.54718, -0.64665, 0.53144},
{-0.41563, 0.81925, -0.39507}, {0.99284, -0.1055, -0.055988},
{-0.52722, -0.71702, 0.45598}, {-0.47375, 0.74925, -0.4628},
{0.98834, -0.017672, 0.15124}, {-0.57512, -0.80486, 0.14645},
{-0.551, -0.82506, 0.12519}, {-0.42564, 0.87581, -0.22759},
{0.9983, -0.054363, 0.021077}, {-0.5548, -0.81812, 0.15127},
{-0.40391, 0.91344, -0.049832}, {0.94024, -0.20082, -0.27499},
{-0.54623, -0.64196, 0.53808}, {-0.43475, 0.80473, -0.40424},
{0.99306, -0.092314, -0.072892}, {-0.52547, -0.69088, 0.49655},
{-0.4428, 0.72475, -0.52789}, {0.98051, 0.018248, 0.19563},
{0.9709, 0.021207, 0.23856}, {-0.58029, -0.79912, 0.15708},
{-0.42674, 0.86998, -0.24702}, {0.99643, -0.059317, 0.060129},
{-0.56305, -0.81425, 0.14133}, {-0.39496, 0.91667, -0.060979},
{0.93542, -0.19374, -0.29572}, {-0.52495, -0.64871, 0.55101},
{-0.45055, 0.7884, -0.41884}, {0.98859, -0.11004, -0.10286},
{-0.52963, -0.64707, 0.54844}, {-0.43668, 0.67521, -0.59448},
{-0.54347, -0.7808, 0.3082}, {-0.38897, 0.7592, -0.52184},
{0.91584, 0.021117, 0.40099}, {-0.51186, -0.84122, -0.17422},
{-0.43196, 0.89474, 0.11339}, {0.95649, -0.10309, -0.27295},
{-0.56304, -0.75356, 0.33932}, {-0.3728, 0.92015, -0.11979},
{0.88726, -0.28987, -0.35881}, {-0.45394, -0.47801, 0.75196},
{-0.473, 0.56152, -0.67895}, {0.97583, 0.10587, 0.19116}, {0.97398, 0.10701, 0.1998},
{-0.55993, -0.74378, 0.36506}, {-0.38228, 0.74056, -0.55266},
{0.92036, 0.027554, 0.39011}, {-0.51256, -0.84148, -0.17085},
{-0.41743, 0.89967, 0.12783}, {0.9478, -0.12216, -0.29455},
{-0.53117, -0.75278, 0.38881}, {-0.34874, 0.92856, -0.12715},
{0.87047, -0.30278, -0.38809}, {-0.45043, -0.42838, 0.78333},
{-0.4785, 0.53424, -0.69687}, {-0.4731, 0.54346, -0.69342},
{0.97276, 0.08925, 0.21396}, {-0.53887, -0.76944, 0.34291},
{-0.38256, 0.75585, -0.53136}, {0.93538, 0.022566, 0.35291},
{-0.52896, -0.83653, -0.14288}, {-0.41569, 0.89518, 0.16078},
{0.92921, -0.12569, -0.34753}, {-0.54879, -0.7427, 0.3837},
{-0.3403, 0.93314, -0.11597}, {0.85628, -0.32915, -0.39805},
{-0.44925, -0.43426, 0.78077}, {-0.46731, -0.42644, 0.77445},
{-0.47067, 0.53259, -0.70343}, {0.96122, 0.11698, 0.24972},
{-0.53792, -0.78998, 0.29423}, {-0.39356, 0.76632, -0.50781},
{0.93251, -0.019703, 0.3606}, {-0.54728, -0.82045, -0.16537},
{-0.39237, 0.9027, 0.17657}, {0.93091, -0.11677, -0.34608},
{-0.54666, -0.73645, 0.3985}, {-0.35867, 0.92143, -0.1494},
{0.87548, -0.31519, -0.36631}, {0.88703, -0.30954, -0.34257},
{-0.47482, -0.42736, 0.76936}, {-0.45893, 0.51073, -0.72701},
{0.95664, 0.13063, 0.26033}, {-0.52488, -0.80646, 0.27224},

```

```

{-0.37989, 0.7837, -0.49142}, {0.92606, -0.039343, 0.37533},
{-0.56145, -0.80716, -0.18239}, {-0.37689, 0.90457, 0.19928},
{0.90417, -0.14827, -0.40062}, {-0.5104, -0.7127, 0.48119},
{-0.37005, 0.91202, -0.17688}, {-0.38213, 0.90107, -0.20505},
{0.89528, -0.30107, -0.32836}, {-0.48923, -0.42523, 0.76147},
{-0.44596, 0.49859, -0.74332}, {0.95335, 0.13332, 0.27082},
{-0.54897, -0.79859, 0.24676}, {-0.35865, 0.79914, -0.48244},
{0.92855, -0.046249, 0.36831}, {-0.55496, -0.80539, -0.20825},
{-0.36573, 0.90345, 0.22367}, {0.8845, -0.14722, -0.44271},
{-0.48953, -0.70409, 0.5144}, {-0.51108, -0.70191, 0.49611},
{-0.38924, 0.89706, -0.20924}, {0.89285, -0.30934, -0.3273},
{-0.48865, -0.42334, 0.76289}, {-0.43678, 0.53072, -0.72633},
{0.96313, 0.074967, 0.25836}, {-0.56419, -0.77955, 0.272},
{-0.3536, 0.79785, -0.48827}, {0.94634, -0.047212, 0.3197},
{-0.56289, -0.81373, -0.14493}, {-0.36308, 0.91021, 0.19924},
{0.88106, -0.16248, -0.44422}, {0.90575, -0.16186, -0.39168},
{-0.5327, -0.72141, 0.44249}, {-0.37291, 0.907, -0.19568},
{0.89877, -0.29773, -0.32181}, {-0.50225, -0.46895, 0.72652},
{-0.44007, 0.57652, -0.68844}, {0.9755, 0.074988, 0.20681},
{-0.54987, -0.8001, 0.23977}, {-0.39558, 0.81291, -0.42744},
{0.96432, -0.053933, 0.2592}, {-0.58127, -0.8079, -0.097068},
{-0.37451, 0.91379, 0.15728}, {-0.38087, 0.91231, 0.15043},
{0.91982, -0.15463, -0.36057}, {-0.52845, -0.72041, 0.44916},
{-0.36714, 0.90835, -0.20029}, {0.89619, -0.30205, -0.32498},
{-0.50321, -0.47571, 0.72144}, {-0.45223, 0.56615, -0.68918},
{0.96123, 0.10182, 0.25624}, {-0.52297, -0.8313, 0.18826},
{-0.42194, 0.82809, -0.3691}, {0.97069, -0.054755, 0.23403},
{-0.57996, -0.80688, -0.11221}, {-0.5563, -0.81955, -0.13737},
{-0.39047, 0.90632, 0.16163}, {0.93772, -0.13405, -0.32049},
{-0.54718, -0.73303, 0.40407}, {-0.35863, 0.91875, -0.16519},
{0.88351, -0.3105, -0.3507}, {-0.49363, -0.47919, 0.72575},
{-0.46182, 0.55431, -0.69243}, {0.96045, 0.13101, 0.24572},
{-0.52417, -0.82287, 0.21941}, {-0.4029, 0.80395, -0.43742},
{0.94876, -0.029276, 0.31463}, {0.94056, -0.0089066, 0.33951},
{-0.53622, -0.83592, -0.11702}, {-0.4158, 0.90138, 0.12095},
{0.94517, -0.12587, -0.30134}, {-0.57239, -0.73211, 0.36931},
{-0.35598, 0.92508, -0.13233}, {0.87008, -0.32221, -0.37301},
{-0.4716, -0.47292, 0.74427}, {-0.46444, 0.56518, -0.68181},
{0.97835, 0.078683, 0.19141}, {-0.55321, -0.76806, 0.32256},
{-0.39698, 0.7678, -0.50288}, {-0.39232, 0.76669, -0.5082},
{0.93911, -0.011744, 0.34341}, {-0.51226, -0.84663, -0.14424},
{-0.42567, 0.89509, 0.13273}, {0.94948, -0.11737, -0.29106},
{-0.56629, -0.74556, 0.35136}, {-0.36441, 0.92413, -0.11483},
{0.87532, -0.30913, -0.37181}, {-0.47246, -0.47684, 0.74121},
{-0.47588, 0.5837, -0.65789}, {0.98545, 0.074764, 0.15262},
{-0.55533, -0.75628, 0.34589}, {0.97047, 0.085782, 0.22546},
{-0.56791, -0.75539, 0.32691}, {-0.36877, 0.74951, -0.54977},
{0.91875, -0.0022875, 0.39483}, {-0.51714, -0.84119, -0.158},
{-0.41692, 0.89846, 0.13766}, {0.94456, -0.1332, -0.30011},
{-0.52743, -0.73538, 0.42548}, {-0.34908, 0.92464, -0.15224},

```

```

{0.87872, -0.30989, -0.36307}, {-0.46761, -0.40493, 0.78573},
{-0.46745, 0.52809, -0.70895}, {-0.45305, 0.53687, -0.7117},
{0.9755, 0.073281, 0.20744}, {-0.55426, -0.77451, 0.30483},
{-0.38508, 0.77465, -0.50163}, {0.93031, -0.010343, 0.36662},
{-0.55487, -0.82104, -0.13423}, {-0.39368, 0.90353, 0.16926},
{0.92282, -0.14677, -0.35618}, {-0.55231, -0.72176, 0.41715},
{-0.33169, 0.93366, -0.13515}, {0.86087, -0.33852, -0.37988},
{-0.47284, -0.40169, 0.78426}, {-0.4846, -0.40741, 0.77407},
{-0.44172, 0.52178, -0.72981}, {0.9641, 0.11493, 0.23939},
{-0.5443, -0.79479, 0.2684}, {-0.3886, 0.78498, -0.48249},
{0.93648, -0.022684, 0.34998}, {-0.5576, -0.81349, -0.16528},
{-0.37995, 0.90456, 0.1934}, {0.91652, -0.15334, -0.36944},
{-0.55019, -0.7219, 0.4197}, {-0.35499, 0.91785, -0.17758},
{0.87878, -0.32374, -0.35063}, {0.88245, -0.32845, -0.33676},
{-0.48777, -0.42932, 0.76011}, {-0.43125, 0.50763, -0.74588},
{0.94647, 0.14487, 0.28846}, {-0.53815, -0.80685, 0.24369},
{-0.36414, 0.80368, -0.47063}, {0.92868, -0.051457, 0.36729},
{-0.57668, -0.79756, -0.17702}, {-0.36441, 0.90842, 0.2049},
{0.889, -0.17385, -0.42361}, {-0.52312, -0.69344, 0.49547},
{-0.36321, 0.90483, -0.22217}, {-0.37586, 0.89786, -0.22929},
{0.89398, -0.32151, -0.31215}, {-0.50877, -0.40435, 0.76003},
{-0.41562, 0.50826, -0.75428}, {0.94594, 0.13482, 0.29498},
{-0.56221, -0.7957, 0.22533}, {-0.36051, 0.81463, -0.45432},
{0.9221, -0.058361, 0.38252}, {-0.5916, -0.78178, -0.19705},
{-0.33265, 0.91525, 0.22731}, {0.87495, -0.18278, -0.44838},
{-0.50817, -0.68734, 0.51896}, {-0.50235, -0.69335, 0.51664},
{-0.38321, 0.89258, -0.23759}, {0.89347, -0.32694, -0.30792},
{-0.50785, -0.41625, 0.75421}, {-0.41555, 0.54143, -0.73087},
{0.95693, 0.081157, 0.27876}, {-0.58958, -0.7728, 0.2349},
{-0.36474, 0.82058, -0.44002}, {0.94295, -0.065844, 0.32635},
{-0.59105, -0.79361, -0.14441}, {-0.34343, 0.91464, 0.2133},
{0.87247, -0.17909, -0.45468}, {0.89999, -0.18567, -0.39439},
{-0.53655, -0.70235, 0.46777}, {-0.35522, 0.90945, -0.21614},
{0.89778, -0.31527, -0.30758}, {-0.52797, -0.45346, 0.71807},
{-0.42041, 0.58136, -0.69662}, {0.96672, 0.051558, 0.25058},
{-0.55646, -0.79971, 0.22542}, {-0.39439, 0.84041, -0.37172},
{0.96403, -0.072681, 0.25565}, {-0.59879, -0.79562, -0.091855},
{-0.35795, 0.9177, 0.17233}, {-0.35221, 0.92142, 0.1641},
{0.90987, -0.17989, -0.37388}, {-0.54971, -0.69048, 0.47017},
{-0.367, 0.90524, -0.21412}, {0.90089, -0.31885, -0.2945},
{-0.51921, -0.45096, 0.72599}, {-0.43647, 0.57521, -0.69183},
{0.95017, 0.10879, 0.29214}, {-0.55006, -0.81481, 0.18309},
{-0.41007, 0.85415, -0.3198}, {0.96559, -0.076085, 0.24868},
{-0.59346, -0.79876, -0.098916}, {-0.57547, -0.80474, -0.1457},
{-0.36829, 0.91548, 0.16208}, {0.92871, -0.1488, -0.33963},
{-0.55029, -0.70892, 0.44115}, {-0.3472, 0.92128, -0.17522},
{0.89553, -0.30103, -0.32773}, {-0.51452, -0.45241, 0.72842},
{-0.429, 0.56761, -0.70269}, {0.95077, 0.11525, 0.28766},
{-0.54974, -0.81013, 0.20366}, {-0.39557, 0.82538, -0.40283},
{0.94864, -0.046483, 0.31293}, {0.94455, -0.023934, 0.32749},

```

```

{-0.56548, -0.81564, -0.12237}, {-0.39453, 0.90899, 0.13448},
{0.93799, -0.15033, -0.31237}, {-0.56655, -0.72458, 0.39244},
{-0.32709, 0.93214, -0.1553}, {0.87836, -0.32219, -0.3531},
{-0.48461, -0.4408, 0.75554}, {-0.44963, 0.57973, -0.67952},
{0.97383, 0.083591, 0.21135}, {-0.56497, -0.76735, 0.30329},
{-0.3746, 0.8022, -0.46493}, {-0.38549, 0.79353, -0.47086},
{0.93842, -0.015111, 0.34517}, {-0.54926, -0.82284, -0.14575},
{-0.39374, 0.9076, 0.14572}, {0.94329, -0.14352, -0.29933},
{-0.5629, -0.73144, 0.38487}, {-0.34349, 0.92882, -0.13898},
{0.88605, -0.30318, -0.35072}, {-0.49466, -0.4589, 0.73805},
{-0.46564, 0.57862, -0.66961}, {0.984, 0.061576, 0.16719},
{-0.56762, -0.75741, 0.3227}, {-0.56309, -0.77451, 0.2882},
{-0.37434, 0.77392, -0.5108}, {0.92483, -0.0023111, 0.38037},
{-0.54478, -0.81999, -0.17557}, {-0.40897, 0.90087, 0.14551},
{0.94695, -0.15449, -0.28183}, {-0.55556, -0.74274, 0.37375},
{-0.34771, 0.925, -0.15323}, {0.8961, -0.29541, -0.33127},
{-0.47651, -0.46072, 0.74878}, {-0.45471, 0.56012, -0.69246},
{0.97241, 0.082896, 0.21807}, {-0.56451, -0.7454, 0.35454},
{-0.37523, 0.74025, -0.55789}, {0.91875, 0.033769, 0.39338},
{-0.51559, -0.83847, -0.17646}, {-0.44468, 0.88865, 0.11212},
{0.95108, -0.11682, -0.28601}, {-0.5324, -0.75162, 0.38939},
{-0.36781, 0.9215, -0.12472}, {0.86666, -0.31357, -0.38804},
{-0.45068, -0.44142, 0.77591}, {-0.48562, 0.52503, -0.69894},
{0.97463, 0.10483, 0.19777}, {0.97585, 0.092137, 0.19804},
{-0.54674, -0.76247, 0.346}, {-0.38369, 0.757, -0.5289},
{0.93528, 0.015984, 0.35355}, {-0.52309, -0.84012, -0.14346},
{-0.42215, 0.8947, 0.14592}, {0.93057, -0.11326, -0.34816},
{-0.54278, -0.7482, 0.38156}, {-0.3426, 0.93258, -0.11371},
{0.8591, -0.32448, -0.3958}, {-0.44118, -0.43696, 0.78385},
{-0.49091, 0.53182, -0.69005}, {-0.47148, 0.54509, -0.69324},
{0.96284, 0.10706, 0.24794}, {-0.53824, -0.7862, 0.30361},
{-0.3914, 0.76544, -0.5108}, {0.92952, -0.0055225, 0.36874},
{-0.53976, -0.82723, -0.15602}, {-0.40531, 0.89545, 0.18409},
{0.9258, -0.11832, -0.35903}, {-0.53786, -0.74081, 0.40238},
{-0.36461, 0.91827, -0.1544}, {0.8784, -0.30859, -0.36494},
{-0.47209, -0.43523, 0.76662}, {-0.46709, -0.43175, 0.77163},
{-0.4574, 0.50616, -0.73116}, {0.95353, 0.1441, 0.26461},
{-0.52884, -0.80329, 0.27394}, {-0.3963, 0.77116, -0.49826},
{0.93017, -0.023562, 0.36638}, {-0.55458, -0.81638, -0.16117},
{-0.38869, 0.89785, 0.20684}, {0.90179, -0.12804, -0.41277},
{-0.5122, -0.71166, 0.48082}, {-0.36106, 0.91431, -0.1835},
{0.88054, -0.32212, -0.3477}, {0.89449, -0.28894, -0.34119},
{-0.48291, -0.41378, 0.77174}, {-0.45055, 0.50291, -0.73762},
{0.95233, 0.13893, 0.27159}, {-0.54169, -0.80027, 0.25719},
{-0.36852, 0.78994, -0.4901}, {0.92624, -0.036195, 0.3752},
{-0.54928, -0.81097, -0.20156}, {-0.36802, 0.9009, 0.23009},
{0.88722, -0.14706, -0.43729}, {-0.50493, -0.70012, 0.50485},
{-0.37064, 0.91029, -0.18438}, {-0.3695, 0.90683, -0.20279},
{0.8877, -0.31166, -0.33892}, {-0.48972, -0.42597, 0.76074},
{-0.44215, 0.54187, -0.71476}, {0.96621, 0.077675, 0.24579},

```

```

{-0.56176, -0.78303, 0.267}, {-0.3483, 0.80251, -0.48442},
{0.94661, -0.05205, 0.31816}, {-0.5593, -0.81286, -0.16261},
{-0.37597, 0.90767, 0.1865}, {0.88921, -0.16483, -0.42678},
{-0.50336, -0.71121, 0.49072}, {-0.52997, -0.72228, 0.44435},
{-0.36891, 0.91075, -0.1856}, {0.90275, -0.29752, -0.31068},
{-0.50014, -0.46144, 0.73275}, {-0.43004, 0.58628, -0.68654},
{0.9737, 0.062789, 0.219}, {-0.55, -0.8016, 0.23438}, {-0.392, 0.81823, -0.42051},
{0.96795, -0.053441, 0.24539}, {-0.57894, -0.80975, -0.095535},
{-0.36818, 0.91605, 0.15905}, {0.90595, -0.15907, -0.39237},
{0.9173, -0.14867, -0.3694}, {-0.53311, -0.71002, 0.46008},
{-0.36591, 0.91098, -0.19034}, {0.89602, -0.30939, -0.31848},
{-0.50896, -0.46863, 0.72205}, {-0.44676, 0.56512, -0.69357},
{0.95885, 0.10709, 0.26292}, {-0.51277, -0.83831, 0.18522},
{-0.41653, 0.83161, -0.36733}, {0.97062, -0.043083, 0.23674},
{-0.57395, -0.81122, -0.11185}, {-0.37801, 0.91151, 0.16203},
{-0.38005, 0.90944, 0.16878}, {0.93839, -0.13015, -0.32014},
{-0.55312, -0.72613, 0.40842}, {-0.35502, 0.91964, -0.16801},
{0.88793, -0.30556, -0.34383}, {-0.49028, -0.47005, 0.73395},
{-0.4589, 0.55282, -0.69556}, {0.9587, 0.13018, 0.25287},
{-0.51675, -0.8298, 0.21071}, {-0.40369, 0.8045, -0.43568},
{0.94668, -0.02639, 0.3211}, {-0.55437, -0.81971, -0.14405},
{-0.54498, -0.83051, -0.11512}, {-0.41597, 0.90186, 0.11668},
{0.94536, -0.13439, -0.29706}, {-0.55836, -0.73813, 0.37868},
{-0.36273, 0.92129, -0.14015}, {0.86802, -0.31883, -0.38064},
{-0.47325, -0.4671, 0.74689}, {-0.46968, 0.5566, -0.68527},
{0.97795, 0.082565, 0.19181}, {-0.54121, -0.77269, 0.33172},
{-0.38421, 0.77815, -0.49685}, {0.94183, -0.013475, 0.33582},
{0.93757, -0.0098296, 0.34765}, {-0.51948, -0.84211, -0.1449},
{-0.41996, 0.89866, 0.12667}, {0.95178, -0.12265, -0.2812},
{-0.5664, -0.74893, 0.34395}, {-0.35753, 0.92538, -0.12584},
{0.87756, -0.31207, -0.36401}, {-0.48018, -0.48462, 0.73114},
{-0.4768, 0.58868, -0.65278}, {0.98458, 0.076608, 0.15728},
{-0.55287, -0.75969, 0.34234}, {-0.39659, 0.7679, -0.50304},
{-0.38665, 0.75801, -0.52528}, {0.91877, 0.018032, 0.39439},
{-0.514, -0.8381, -0.18273}, {-0.4295, 0.89417, 0.12648},
{0.95503, -0.11206, -0.27451}, {-0.56028, -0.75103, 0.34933},
{-0.37739, 0.91698, -0.12934}, {0.8885, -0.28843, -0.3569},
{-0.46647, -0.47465, 0.7464}, {-0.47505, 0.56056, -0.67831},
{0.97516, 0.095627, 0.19982}, {-0.53918, -0.7798, 0.3181},
{-0.38978, 0.74201, -0.54543}, {0.91786, 0.048078, 0.39399},
{-0.4929, -0.85282, -0.17248}, {-0.4476, 0.88438, 0.13238},
{0.96329, -0.10683, -0.2463}, {-0.5437, -0.77778, 0.31537},
{-0.36465, 0.92683, -0.089519}, {0.88686, -0.26938, -0.3754},
{-0.4393, -0.47688, 0.76132}, {-0.49733, 0.56562, -0.65783},
{0.98025, 0.10282, 0.16895}, {-0.53428, -0.78012, 0.32551},
{-0.53967, -0.7548, 0.37288}, {-0.38277, 0.7214, -0.57712},
{0.91369, 0.046143, 0.40378}, {-0.49219, -0.85801, -0.14685},
{-0.44216, 0.88807, 0.12583}, {0.95738, -0.088988, -0.27477},
{-0.52142, -0.76689, 0.37416}, {-0.37965, 0.92014, -0.095897},
{0.86264, -0.2853, -0.41767}, {-0.42423, -0.44007, 0.79144},

```

```

{-0.51017, 0.53543, -0.67308}, {0.97904, 0.10797, 0.17268},
{0.98282, 0.090792, 0.16071}, {-0.53557, -0.77302, 0.34001},
{-0.40912, 0.72961, -0.54799}, {0.9183, 0.040993, 0.39375},
{-0.51329, -0.84704, -0.13802}, {-0.42931, 0.89011, 0.15296},
{0.93965, -0.089955, -0.33011}, {-0.51359, -0.76769, 0.38325},
{-0.34602, 0.93538, -0.072978}, {0.84876, -0.31498, -0.42473},
{-0.42473, -0.43469, 0.79413}, {-0.49328, 0.55003, -0.6739},
{-0.49611, 0.52336, -0.6928}, {0.97439, 0.1137, 0.194},
{-0.53188, -0.78664, 0.31352}, {-0.41515, 0.74326, -0.5246},
{0.93138, 0.01727, 0.36364}, {-0.5087, -0.84473, -0.1663},
{-0.4081, 0.89545, 0.1778}, {0.93415, -0.109, -0.33982},
{-0.52953, -0.7619, 0.37296}, {-0.37121, 0.91957, -0.12883},
{0.86618, -0.31207, -0.39031}, {-0.45108, -0.43382, 0.77995},
{-0.45221, -0.44654, 0.77208}, {-0.48255, 0.501, -0.71843},
{0.9617, 0.14774, 0.2309}, {-0.52542, -0.79847, 0.2939},
{-0.39055, 0.76349, -0.51435}, {0.9223, 0.0080541, 0.38639},
{-0.54102, -0.82229, -0.17646}, {-0.40842, 0.89326, 0.18783},
{0.91312, -0.12032, -0.38954}, {-0.50989, -0.73852, 0.44115},
{-0.37445, 0.91257, -0.16433}, {0.86833, -0.30791, -0.38885},
{0.88191, -0.30546, -0.35906}, {-0.47121, -0.42399, 0.77343},
{-0.4648, 0.50324, -0.7285}, {0.95873, 0.14679, 0.2435},
{-0.54254, -0.79108, 0.28256}, {-0.3902, 0.77776, -0.49278},
{0.91235, -0.011809, 0.40923}, {-0.53863, -0.81836, -0.20043},
{-0.39565, 0.8905, 0.22465}, {0.9041, -0.12817, -0.40765},
{-0.49381, -0.72975, 0.47289}, {-0.3825, 0.90824, -0.16967},
{-0.39089, 0.90336, -0.17648}, {0.88288, -0.30844, -0.3541},
{-0.47043, -0.43472, 0.76793}, {-0.45633, 0.53514, -0.7109},
{0.9707, 0.090522, 0.2226}, {-0.55316, -0.77889, 0.29554},
{-0.38214, 0.77727, -0.49981}, {0.93456, -0.016938, 0.3554},
{-0.5476, -0.82394, -0.14581}, {-0.39334, 0.89859, 0.19446},
{0.89382, -0.1455, -0.42417}, {-0.50521, -0.72041, 0.47516},
{-0.53378, -0.72677, 0.4323}, {-0.36963, 0.91429, -0.16568},
{0.89714, -0.27967, -0.34194}, {-0.48337, -0.46372, 0.74251},
{-0.44764, 0.57067, -0.68844}, {0.97663, 0.07556, 0.20122},
{-0.53329, -0.79913, 0.27749}, {-0.41911, 0.80987, -0.41045},
{0.95477, -0.0382, 0.29488}, {-0.55737, -0.82537, -0.090032},
{-0.39704, 0.90123, 0.17364}, {0.91483, -0.1335, -0.38114},
{0.92637, -0.13709, -0.35078}, {-0.52737, -0.73623, 0.42407},
{-0.37718, 0.91212, -0.16053}, {0.89439, -0.29484, -0.33635},
{-0.48124, -0.48618, 0.72941}, {-0.47202, 0.56947, -0.67299},
{0.9661, 0.12317, 0.2269}, {-0.51784, -0.82203, 0.23687},
{-0.43787, 0.8187, -0.37148}, {0.95987, -0.029277, 0.2789},
{-0.55551, -0.82415, -0.11036}, {-0.40141, 0.90191, 0.15946},
{-0.41774, 0.89777, 0.13968}, {0.94251, -0.12135, -0.31138},
{-0.54542, -0.74238, 0.3891}, {-0.37846, 0.91662, -0.12876},
{0.89269, -0.27582, -0.35642}, {-0.4596, -0.47063, 0.75317},
{-0.4646, 0.56689, -0.68028}, {0.9606, 0.13675, 0.24198},
{-0.52404, -0.81366, 0.25166}, {-0.41949, 0.79353, -0.44084},
{0.94043, 0.0098713, 0.33983}, {-0.53113, -0.83595, -0.13815},
{-0.52882, -0.84115, -0.11322}, {-0.43873, 0.89086, 0.11782},

```

```
{0.95252, -0.11381, -0.28239}, {-0.55187, -0.75583, 0.35237},
{-0.34278, 0.9349, -0.091974}, {0.87578, -0.29523, -0.3819},
{-0.45098, -0.46526, 0.76167}, {-0.48081, 0.5789, -0.65856},
{0.98139, 0.091324, 0.1689}, {-0.53493, -0.77098, 0.3456},
{-0.41348, 0.75615, -0.50722}, {0.93336, 0.018288, 0.35847},
{0.93345, 0.015157, 0.35838}, {-0.50861, -0.85046, -0.1343},
{-0.44418, 0.88719, 0.12488}, {0.9585, -0.090139, -0.27047},
{-0.55832, -0.76132, 0.32964}, {-0.35309, 0.93191, -0.082937},
{0.87847, -0.2827, -0.3852}, {-0.45494, -0.4761, 0.75257},
{-0.48802, 0.58727, -0.64572}, {0.98818, 0.069627, 0.13657},
{-0.537, -0.76154, 0.3629}, {-0.40487, 0.75388, -0.51744}};
```

```
In[10]:= Length[r]
```

```
Out[10]= 864
```

The graphical representation of the ground state vectors in a common origin plot shows that the vectors are arranged in the form of three separate strands.

```
In[11]:= Graphics3D[
  {Table[Point[r[[μ]]], {μ, Length[r]}], {Opacity[0.4], Sphere[]}}, Boxed → False]
```

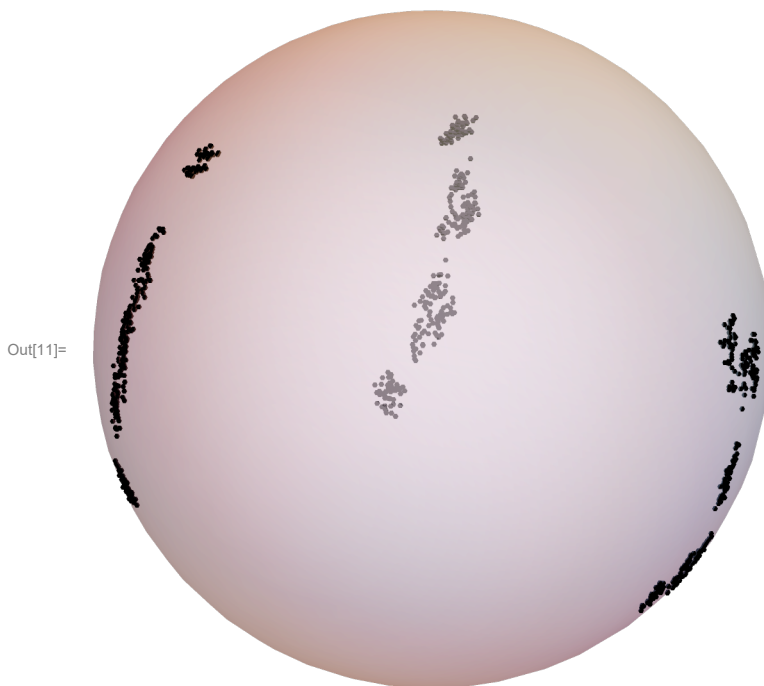

For later purposes we calculate the ground state energy (per spin site) “ee” of the numerical ground state r:

```
In[12]:= ee = 1 / (2 NN) Sum[JA[[μ, ν]] × r[[μ]] . r[[ν]], {μ, NN}, {ν, NN}]
```

```
Out[12]= -1.36709
```

The next task is to identify closely spaced spin vectors. This requires a large

number of analyses, of which we will present only the results here.

The first observation is that the two spins numbered “3” and “5” in the same unit cell are always very close to each other, with a scalar product  $\geq 0.992289$ . This follows from the following calculations and indicates symmetry breaking for the numerical ground state, since the spins of the equivalent pair (4,6) are not close.

```
In[13]:= For[m = 0, m <= 11, m++, For[n = 0, n <= 11, n++,
      G[m, n] = Table[r[[pos[i, m, n]]].r[[pos[j, m, n]]], {i, 6}, {j, 6}]]]
```

```
In[14]:= GG =
      Table[Min[Flatten[Table[G[m, n][[i, j]], {m, 0, 11}, {n, 0, 11}], 2]], {i, 6}, {j, 6}];
      GG // TableForm
```

Out[14]//TableForm=

|           |           |           |           |           |           |
|-----------|-----------|-----------|-----------|-----------|-----------|
| 1.        | -0.56762  | -0.497048 | 0.917025  | -0.499124 | -0.512536 |
| -0.56762  | 1.        | -0.494561 | -0.515095 | -0.496512 | 0.920096  |
| -0.497048 | -0.494561 | 1.        | -0.551344 | 0.992289  | -0.550762 |
| 0.917025  | -0.515095 | -0.551344 | 1.        | -0.550391 | -0.460829 |
| -0.499124 | -0.496512 | 0.992289  | -0.550391 | 1.        | -0.553022 |
| -0.512536 | 0.920096  | -0.550762 | -0.460829 | -0.553022 | 1.        |

```
In[15]:= Sort[Flatten[GG]] [[-7]]
```

Out[15]= 0.992289

Next, we note that any two spins with sites  $\{i, m, n\}$  and  $\{i, m+1, n+1\}$  are always close, with a scalar product  $\geq 0.990749$ , where the addition is understood mod 12. This follows from the following calculations and again indicates the afore-mentioned symmetry breaking, since spins in unit cells are identified along the diagonals with positive slope and not along the diagonals with negative slope.

```
In[16]:= For[i = 1, i <= 6, i++, For[m = 0, m <= 11, m++, For[n = 0, n <= 11, n++,
      H[i, m, n] = r[[pos[i, m, n]]].r[[pos[i, Mod[m + 1, 12], Mod[n + 1, 12]]]]]]]
```

```
In[17]:= HH = Flatten[Table[H[i, m, n], {m, 0, 11}, {n, 0, 11}, {i, 1, 6}, {i, 6}], 3];
      Min[HH]
```

Out[17]= 0.990749

The third observation is that any two spins at sites  $\{2, m, n\}$  and  $\{1, m+1, n\}$  are always very close, with a scalar product  $\geq 0.994236$  and the addition understood mod 12. This follows from the following calculations:

```
In[18]:= For[m = 0, m <= 11, m++,
      For[n = 0, n <= 11, n++, K[m, n] = r[[pos[2, m, n]]].r[[pos[1, Mod[m + 1, 12], n]]]]]
```



```
In[27]:= Total[SitL]
NN
```

```
Out[27]= 864
```

```
Out[28]= 864
```

The numerical approximation  $s[\lambda]$  of the  $\lambda$ -th spin vector will be calculated as a (normalized) mean value of the numerical ground state vectors:

```
In[29]:= For[λ = 1, λ <= MM, λ++,
  s[λ] = Sum[r[[Sit[λ][[i]]]], {i, Length[Sit[λ]]} / Length[Sit[λ]];
  s[λ] = s[λ] / Sqrt[s[λ].s[λ]]]
```

It is possible to define a 48×48 representative J-Matrix JR describing the coupling between different spins and gives the same (or even slightly lower) energy “ee1” as the original J-matrix. For later purposes we let Jp and Jc undefined.

```
In[30]:= JR = Table[0, {MM}, {MM}];
```

```
In[31]:= For[μ = 1, μ <= NN, μ++, κ = StoR[μ];
  For[ν = 1, ν <= NN, ν++, λ = StoR[ν];
    If[Not[TrueQ[J[[μ, ν]] == 0]],
      JR[[λ, κ]] = JR[[λ, κ]] + J[[μ, ν]] /. {J1 -> 1, J2 -> 1, J3 -> 1}]]]
```

```
In[32]:= JR = Simplify[JR];
```

```
In[33]:= ee1 = 1/2 NN Sum[(JR[[κ, λ]] /. val) × s[λ].s[κ], {λ, MM}, {κ, MM}]
```

```
Out[33]= -1.36718
```

```
In[34]:= ee
```

```
Out[34]= -1.36709
```

To find the vertical symmetry axis we compute a sort of “inertial tensor”  $\Theta$  of the representative spin configuration and re-define the spin components w.r.t. the eigenbasis of  $\Theta$ , resulting in spin vectors  $t[\lambda]$ ,  $\lambda=1,...,48$ :

```
In[35]:= Θ = Table[Sum[Length[Sit[μ]] × s[μ][[i]] × s[μ][[j]], {μ, MM}], {i, 3}, {j, 3}];
Θ // TableForm
```

```
Out[35]//TableForm=
387.327      -7.25173      -20.4795
-7.25173      346.533      -106.751
-20.4795      -106.751      130.14
```

```
In[36]:= es = Eigensystem[0]
Out[36]= {{390.892, 388.322, 84.7859}, {-0.466216, -0.805278, 0.366293},
          {0.881774, -0.456469, 0.118792}, {0.071541, 0.37837, 0.922886}}
In[37]:= For[μ = 1, μ <= MM, μ++, t[μ] = es[[2]].s[μ]]
```

Next we observe a reflection symmetry  $S$  of the spin configuration w.r.t. the equatorial plane.  $SP$  is the list of pairs of numbers of spin vectors which are approximate reflections of each other. Let  $\{t[a], t[b]\}$  be such a pair. Then the scalar product between  $t[a]$  and  $S\ t[b]$  will always be  $\geq 0.999862$ :

```
In[38]:= SP = {};
In[39]:= For[v = 1, v <= MM, v++, tab = Table[
          t[μ][[1]] × t[v][[1]] + t[μ][[2]] × t[v][[2]] - t[μ][[3]] × t[v][[3]], {μ, MM}];
          max = Max[tab];
          pos = Position[tab, max][[1, 1]];
          AppendTo[SP, Sort[{v, pos}]]];
In[40]:= SP = Union[SP]
Out[40]= {{1, 7}, {2, 8}, {3, 9}, {4, 10}, {5, 11}, {6, 12}, {13, 19}, {14, 20},
          {15, 21}, {16, 22}, {17, 23}, {18, 24}, {25, 31}, {26, 32}, {27, 33}, {28, 34},
          {29, 35}, {30, 36}, {37, 43}, {38, 44}, {39, 45}, {40, 46}, {41, 47}, {42, 48}}
In[41]:= Length[SP]
Out[41]= 24
In[42]:= SP1 = Table[SP[[i, 1]], {i, Length[SP]}]
Out[42]= {1, 2, 3, 4, 5, 6, 13, 14, 15, 16, 17, 18, 25, 26, 27, 28, 29, 30, 37, 38, 39, 40, 41, 42}
In[43]:= Min[Table[μ = SP[[i, 1]];
          v = SP[[i, 2]];
          t[μ][[1]] × t[v][[1]] + t[μ][[2]] × t[v][[2]] - t[μ][[3]] × t[v][[3]],
          {i, Length[SP]}]]
Out[43]= 0.999862
```

Summarizing, we can describe the ground state configuration by the positions of 24 spin vectors  $v[i]$  with numbers  $i$  given by the list  $SP1$  above. This gives 48 parameters

$z[i], \phi[i], i \in SP1$ , which are sufficient to describe the ground state. We will use the freedom of a further rotation about the  $z$ -axis to choose  $\phi[1]=0$  and thus to further reduce the number of parameters to 47.

```
In[44]:= Clear[v]
```

```

In[45]:= For[i = 1, i <= Length[SP], i++, j = SP[[i, 1]];
          k = SP[[i, 2]];
          v[j] = {Sqrt[1 - z[j]^2] Cos[phi[j]], Sqrt[1 - z[j]^2] Sin[phi[j]], z[j]} /. phi[1] -> 0;
          v[k] = {Sqrt[1 - z[j]^2] Cos[phi[j]], Sqrt[1 - z[j]^2] Sin[phi[j]], -z[j]} /. phi[1] -> 0}

```

For the numerical ground state these parameters assume the following values:

```

In[46]:= phi[1] = Arg[t[SP1[[1]]][[1]] + i t[SP1[[1]]][[2]]]

```

```

Out[46]= 1.98342

```

```

In[47]:= sub = Join[Table[z[SP1[[i]]] -> t[SP1[[i]]][[3]], {i, Length[SP1]}],
               Table[phi[SP1[[i]]] -> Arg[t[SP1[[i]]][[1]] + i t[SP1[[i]]][[2]]] - phi[1],
               {i, 2, Length[SP1]}]]

```

```

Out[47]= {z[1] -> 0.30359, z[2] -> -0.286354, z[3] -> 0.187337,
          z[4] -> -0.0327822, z[5] -> -0.134308, z[6] -> 0.249182, z[13] -> -0.0739623,
          z[14] -> 0.315896, z[15] -> -0.470119, z[16] -> 0.491016, z[17] -> -0.380675,
          z[18] -> 0.174287, z[25] -> 0.332977, z[26] -> -0.478999, z[27] -> 0.496226,
          z[28] -> -0.36549, z[29] -> 0.151714, z[30] -> 0.101205, z[37] -> -0.197267,
          z[38] -> -0.0511767, z[39] -> 0.292988, z[40] -> -0.457743, z[41] -> 0.501752,
          z[42] -> -0.395768, phi[2] -> -4.18755, phi[3] -> -2.0932, phi[4] -> -0.00379932,
          phi[5] -> -4.19463, phi[6] -> -2.10253, phi[13] -> -2.06869, phi[14] -> 0.0827858,
          phi[15] -> -4.13011, phi[16] -> -2.1273, phi[17] -> -0.0902281, phi[18] -> -4.24462,
          phi[25] -> 0.0675476, phi[26] -> -4.1563, phi[27] -> -2.15773, phi[28] -> -0.106128,
          phi[29] -> -4.25943, phi[30] -> -2.0827, phi[37] -> -4.22691, phi[38] -> -2.05932,
          phi[39] -> 0.100024, phi[40] -> -4.11019, phi[41] -> -2.10303, phi[42] -> -0.0680268}

```

```

In[48]:= try = Table[Apply[List, sub[[i]]], {i, Length[sub]}]

```

```

Out[48]= {{z[1], 0.30359}, {z[2], -0.286354}, {z[3], 0.187337}, {z[4], -0.0327822},
          {z[5], -0.134308}, {z[6], 0.249182}, {z[13], -0.0739623}, {z[14], 0.315896},
          {z[15], -0.470119}, {z[16], 0.491016}, {z[17], -0.380675}, {z[18], 0.174287},
          {z[25], 0.332977}, {z[26], -0.478999}, {z[27], 0.496226}, {z[28], -0.36549},
          {z[29], 0.151714}, {z[30], 0.101205}, {z[37], -0.197267}, {z[38], -0.0511767},
          {z[39], 0.292988}, {z[40], -0.457743}, {z[41], 0.501752}, {z[42], -0.395768},
          {phi[2], -4.18755}, {phi[3], -2.0932}, {phi[4], -0.00379932}, {phi[5], -4.19463},
          {phi[6], -2.10253}, {phi[13], -2.06869}, {phi[14], 0.0827858}, {phi[15], -4.13011},
          {phi[16], -2.1273}, {phi[17], -0.0902281}, {phi[18], -4.24462}, {phi[25], 0.0675476},
          {phi[26], -4.1563}, {phi[27], -2.15773}, {phi[28], -0.106128}, {phi[29], -4.25943},
          {phi[30], -2.0827}, {phi[37], -4.22691}, {phi[38], -2.05932}, {phi[39], 0.100024},
          {phi[40], -4.11019}, {phi[41], -2.10303}, {phi[42], -0.0680268}}

```

The energy (per site) EV of the spin configuration described by the 47 parameters is evaluated as follows:

```

In[49]:= EV = Simplify[1/2 NN Sum[Jr[[k, l]] * v[l].v[k], {l, MM}, {k, MM}]]

```

$$\begin{aligned}
\text{Out[49]} = & \frac{1}{36} \times \left( 6 \text{Jc} + 2 \text{Jp} z[1] \times z[2] + 2 \text{Jp} \cos[\phi[2]] \sqrt{1-z[1]^2} \sqrt{1-z[2]^2} + \right. \\
& 2 \text{Jp} z[2] \times z[3] + 2 \text{Jp} \cos[\phi[2] - \phi[3]] \sqrt{1-z[2]^2} \sqrt{1-z[3]^2} + \\
& 2 \text{Jp} z[3] \times z[4] + 2 \text{Jp} \cos[\phi[3] - \phi[4]] \sqrt{1-z[3]^2} \sqrt{1-z[4]^2} + 2 \text{Jp} z[4] \times z[5] + \\
& 2 \text{Jp} \cos[\phi[4] - \phi[5]] \sqrt{1-z[4]^2} \sqrt{1-z[5]^2} - 2 \text{Jp} z[1] \times z[6] + 2 \text{Jp} z[5] \times z[6] + \\
& 2 \text{Jp} \cos[\phi[6]] \sqrt{1-z[1]^2} \sqrt{1-z[6]^2} + 2 \text{Jp} \cos[\phi[5] - \phi[6]] \sqrt{1-z[5]^2} \sqrt{1-z[6]^2} + \\
& 2 z[1] \times z[13] + 2 z[2] \times z[13] + 2 \cos[\phi[13]] \sqrt{1-z[1]^2} \sqrt{1-z[13]^2} + \\
& 2 \cos[\phi[2] - \phi[13]] \sqrt{1-z[2]^2} \sqrt{1-z[13]^2} + 2 z[2] \times z[14] + 2 z[3] \times z[14] + \\
& 2 \cos[\phi[2] - \phi[14]] \sqrt{1-z[2]^2} \sqrt{1-z[14]^2} + 2 \cos[\phi[3] - \phi[14]] \sqrt{1-z[3]^2} \sqrt{1-z[14]^2} + \\
& 2 z[3] \times z[15] + 2 z[4] \times z[15] + 2 \cos[\phi[3] - \phi[15]] \sqrt{1-z[3]^2} \sqrt{1-z[15]^2} + \\
& 2 \cos[\phi[4] - \phi[15]] \sqrt{1-z[4]^2} \sqrt{1-z[15]^2} + 2 z[4] \times z[16] + 2 z[5] \times z[16] + \\
& 2 \cos[\phi[4] - \phi[16]] \sqrt{1-z[4]^2} \sqrt{1-z[16]^2} + 2 \cos[\phi[5] - \phi[16]] \sqrt{1-z[5]^2} \sqrt{1-z[16]^2} + \\
& 2 z[5] \times z[17] + 2 z[6] \times z[17] + 2 \cos[\phi[5] - \phi[17]] \sqrt{1-z[5]^2} \sqrt{1-z[17]^2} + \\
& 2 \cos[\phi[6] - \phi[17]] \sqrt{1-z[6]^2} \sqrt{1-z[17]^2} - 2 z[1] \times z[18] + 2 z[6] \times z[18] + \\
& 2 \cos[\phi[18]] \sqrt{1-z[1]^2} \sqrt{1-z[18]^2} + 2 \cos[\phi[6] - \phi[18]] \sqrt{1-z[6]^2} \sqrt{1-z[18]^2} + \\
& 2 z[2] \times z[25] + 2 z[13] \times z[25] + 2 \cos[\phi[2] - \phi[25]] \sqrt{1-z[2]^2} \sqrt{1-z[25]^2} + \\
& 2 \cos[\phi[13] - \phi[25]] \sqrt{1-z[13]^2} \sqrt{1-z[25]^2} + 2 z[3] \times z[26] + \\
& 2 z[14] \times z[26] + 2 \cos[\phi[3] - \phi[26]] \sqrt{1-z[3]^2} \sqrt{1-z[26]^2} + \\
& 2 \cos[\phi[14] - \phi[26]] \sqrt{1-z[14]^2} \sqrt{1-z[26]^2} + 2 z[4] \times z[27] + \\
& 2 z[15] \times z[27] + 2 \cos[\phi[4] - \phi[27]] \sqrt{1-z[4]^2} \sqrt{1-z[27]^2} + \\
& 2 \cos[\phi[15] - \phi[27]] \sqrt{1-z[15]^2} \sqrt{1-z[27]^2} + 2 z[5] \times z[28] + \\
& 2 z[16] \times z[28] + 2 \cos[\phi[5] - \phi[28]] \sqrt{1-z[5]^2} \sqrt{1-z[28]^2} + \\
& 2 \cos[\phi[16] - \phi[28]] \sqrt{1-z[16]^2} \sqrt{1-z[28]^2} + 2 z[6] \times z[29] + \\
& 2 z[17] \times z[29] + 2 \cos[\phi[6] - \phi[29]] \sqrt{1-z[6]^2} \sqrt{1-z[29]^2} + \\
& 2 \cos[\phi[17] - \phi[29]] \sqrt{1-z[17]^2} \sqrt{1-z[29]^2} - 2 z[1] \times z[30] + 2 z[18] \times z[30] + \\
& 2 \cos[\phi[30]] \sqrt{1-z[1]^2} \sqrt{1-z[30]^2} + 2 \cos[\phi[18] - \phi[30]] \sqrt{1-z[18]^2} \sqrt{1-z[30]^2} + \\
& 2 z[1] \times z[37] + 2 z[13] \times z[37] - \text{Jc} z[29] \times z[37] + \\
& 2 \cos[\phi[37]] \sqrt{1-z[1]^2} \sqrt{1-z[37]^2} + 2 \cos[\phi[13] - \phi[37]] \sqrt{1-z[13]^2} \sqrt{1-z[37]^2} + \\
& \text{Jc} \cos[\phi[29] - \phi[37]] \sqrt{1-z[29]^2} \sqrt{1-z[37]^2} + 2 z[2] \times z[38] + \\
& 2 z[14] \times z[38] - \text{Jc} z[30] \times z[38] + 2 \cos[\phi[2] - \phi[38]] \sqrt{1-z[2]^2} \sqrt{1-z[38]^2} + \\
& 2 \cos[\phi[14] - \phi[38]] \sqrt{1-z[14]^2} \sqrt{1-z[38]^2} + \\
& \text{Jc} \cos[\phi[30] - \phi[38]] \sqrt{1-z[30]^2} \sqrt{1-z[38]^2} + 2 z[3] \times z[39] + \\
& 2 z[15] \times z[39] + \text{Jc} z[25] \times z[39] + 2 \cos[\phi[3] - \phi[39]] \sqrt{1-z[3]^2} \sqrt{1-z[39]^2} + \\
& 2 \cos[\phi[15] - \phi[39]] \sqrt{1-z[15]^2} \sqrt{1-z[39]^2} + \\
& \text{Jc} \cos[\phi[25] - \phi[39]] \sqrt{1-z[25]^2} \sqrt{1-z[39]^2} + 2 z[4] \times z[40] + \\
& 2 z[16] \times z[40] + \text{Jc} z[26] \times z[40] + 2 \cos[\phi[4] - \phi[40]] \sqrt{1-z[4]^2} \sqrt{1-z[40]^2} + \\
& 2 \cos[\phi[16] - \phi[40]] \sqrt{1-z[16]^2} \sqrt{1-z[40]^2} + \\
& \text{Jc} \cos[\phi[26] - \phi[40]] \sqrt{1-z[26]^2} \sqrt{1-z[40]^2} + 2 z[5] \times z[41] + \\
& 2 z[17] \times z[41] + \text{Jc} z[27] \times z[41] + 2 \cos[\phi[5] - \phi[41]] \sqrt{1-z[5]^2} \sqrt{1-z[41]^2} + \\
& 2 \cos[\phi[17] - \phi[41]] \sqrt{1-z[17]^2} \sqrt{1-z[41]^2} + \\
& \text{Jc} \cos[\phi[27] - \phi[41]] \sqrt{1-z[27]^2} \sqrt{1-z[41]^2} + 2 z[6] \times z[42] +
\end{aligned}$$

$$2 z[18] \times z[42] + Jc z[28] \times z[42] + 2 \cos[\phi[6] - \phi[42]] \sqrt{1 - z[6]^2} \sqrt{1 - z[42]^2} + \\ 2 \cos[\phi[18] - \phi[42]] \sqrt{1 - z[18]^2} \sqrt{1 - z[42]^2} + \\ Jc \cos[\phi[28] - \phi[42]] \sqrt{1 - z[28]^2} \sqrt{1 - z[42]^2}$$

We check the energy for the numerical ground state:

```
In[50]:= EV /. val /. sub
```

```
Out[50]= -1.36718
```

```
In[51]:= ee1
```

```
Out[51]= -1.36718
```

It is possible to lower the energy a bit more to ee2=-1.36719 with the command FindMinimum[...]:

```
In[52]:= {ee2, rule} = FindMinimum[EV /. val, try]
```

```
Out[52]= {-1.36719, {z[1] -> 0.311596, z[2] -> -0.287905, z[3] -> 0.18945,
  z[4] -> -0.0327949, z[5] -> -0.13502, z[6] -> 0.259062, z[13] -> -0.0799723,
  z[14] -> 0.315322, z[15] -> -0.469915, z[16] -> 0.496651, z[17] -> -0.386531,
  z[18] -> 0.174895, z[25] -> 0.338187, z[26] -> -0.481991, z[27] -> 0.494381,
  z[28] -> -0.370693, z[29] -> 0.149992, z[30] -> 0.107347, z[37] -> -0.201371,
  z[38] -> -0.0533123, z[39] -> 0.295355, z[40] -> -0.462186, z[41] -> 0.503477,
  z[42] -> -0.405956, phi[2] -> -4.18535, phi[3] -> -2.09044, phi[4] -> 0.00137808,
  phi[5] -> -4.19058, phi[6] -> -2.09702, phi[13] -> -2.06687, phi[14] -> 0.0876626,
  phi[15] -> -4.12466, phi[16] -> -2.12485, phi[17] -> -0.0889819, phi[18] -> -4.2443,
  phi[25] -> 0.0684796, phi[26] -> -4.15094, phi[27] -> -2.15095, phi[28] -> -0.107248,
  phi[29] -> -4.25726, phi[30] -> -2.08043, phi[37] -> -4.22911, phi[38] -> -2.05436,
  phi[39] -> 0.103251, phi[40] -> -4.10121, phi[41] -> -2.09735, phi[42] -> -0.0668957}}
```

```
In[53]:= Length[rule]
```

```
Out[53]= 47
```

A graphical representation of the semi-analytically reconstructed ground state for Jc=-1, Jp=0.2 follows. We still recognize the three strands:

```
In[54]:= EQUA = Plot3D[0, {x, y} ∈ Region[Disk[]], Mesh -> None, PlotStyle -> Opacity[0.2]];
```

```
In[55]:= GA = Graphics3D[Join[
  Table[{PointSize[0.01], Point[v[λ] /. rule]}, {λ, MM}], {Opacity[0.4], Sphere[]}]];
```

```
In[56]:= LONE = Graphics3D[{Red, Line[{{0, 0, 1}, {0, 0, -1}}], Point[{0, 0, 0}]}];
```

```
In[57]:= Show[GA, EQUA, LONE, Boxed -> False]
```

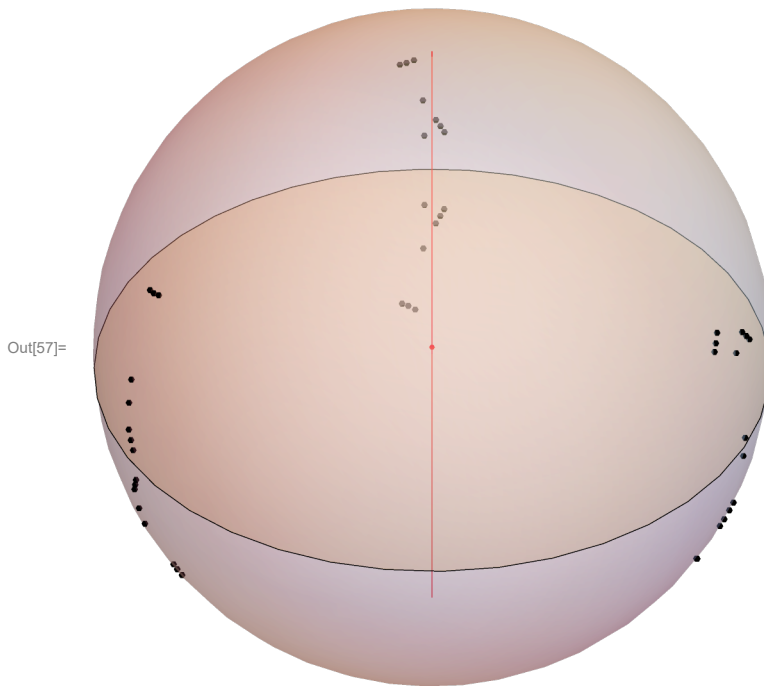

The advantage of having derived an explicit form of the energy  $EV$  is that we do not need to repeat the above numerical calculations for different values of  $J_p$  and  $J_c$ , but can minimize  $EV$  directly. As an example, we calculate the energy of the ground state phase  $V$  for the interval  $J_p \in (0.008, 0.2)$ ,  $J_c = -1$  (for values  $J_p < 0.008$  the `FindMinimum[...]`-command does not give reasonable results anymore):

```
In[58]:= ini0 = Table[Apply[List, rule[[i]]], {i, Length[rule]}];
```

```
In[59]:= Length[ini0]
```

```
Out[59]= 47
```

```
In[60]:= JE = {{0.2, ee2}}
```

```
Out[60]= {{0.2, -1.36719}}
```

```
In[61]:= ini = ini0;
```

```
In[62]:= For[x = 0.199, x >= 0.008, x = x - 0.001,
  {ee, rule} = FindMinimum[EV /. {Jp -> x, Jc -> -1}, ini];
  ini = Table[Apply[List, rule[[i]]], {i, Length[rule]}];
  AppendTo[JE, {x, ee}]]
```

```
In[63]:= ListPlot[JE, AxesLabel → {"J+", "Emin"}, LabelStyle → Directive[14, Gray],
  Epilog → {Text[Style["Jx = -1", 24, Gray], {0.1, -1.36}], PlotRange → All]
```

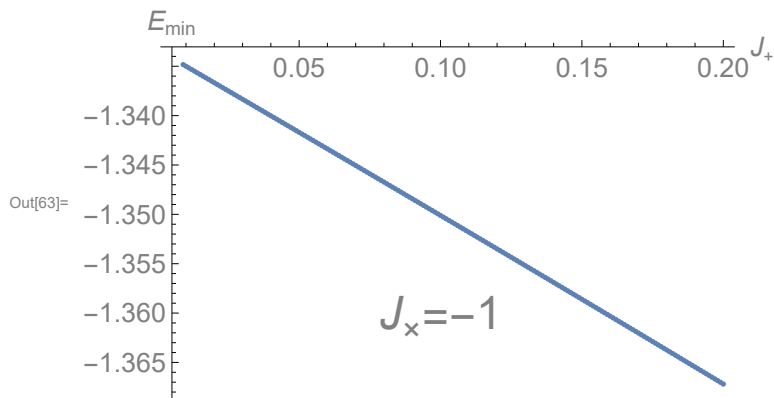

A graphical representation of the semi-analytically reconstructed ground state for  $J_c = -1$ ,  $J_p = 0.008$ , which approximates a  $120^\circ$  ground state of the adjacent phase VI, follows:

```
In[64]:= GA = Graphics3D[Join[
  Table[{PointSize[0.01], Point[v[λ] /. rule]}, {λ, MM}], {Opacity[0.4], Sphere[]}]];
```

```
In[65]:= Show[GA, EQUA, LONE, Boxed → False]
```

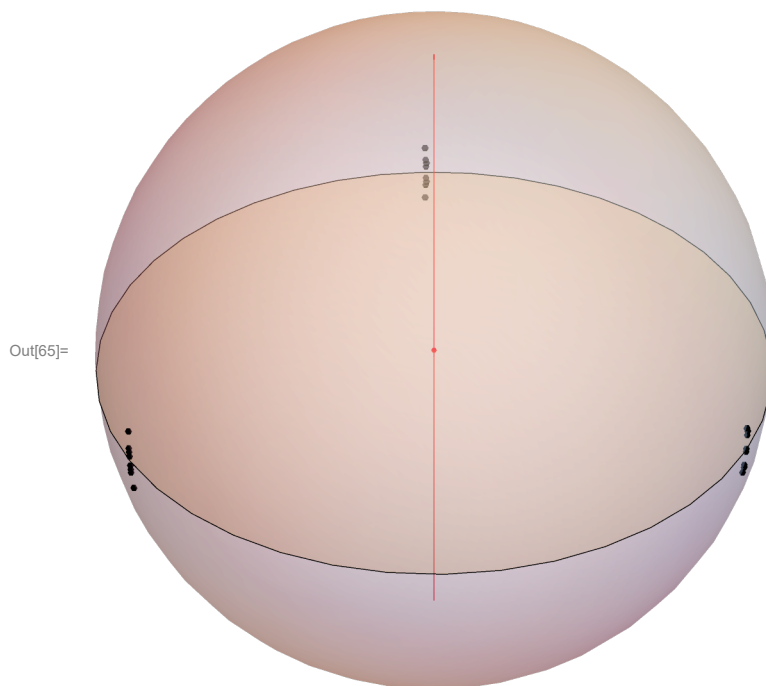

## Phase IV

We will not present the identification of the nearby spins of phase IV in as much detail as in the case of phase V, focusing instead on the symmetry analysis. In particular, we will omit the detailed coordinates of the numerical ground state for the standard values  $\{J_1 \rightarrow 1, J_2 \rightarrow 1, J_3 \rightarrow 1, J_p \rightarrow \frac{1}{5}, J_c \rightarrow -\frac{1}{5}\}$  and present only the common origin plot of this ground state from “above”:

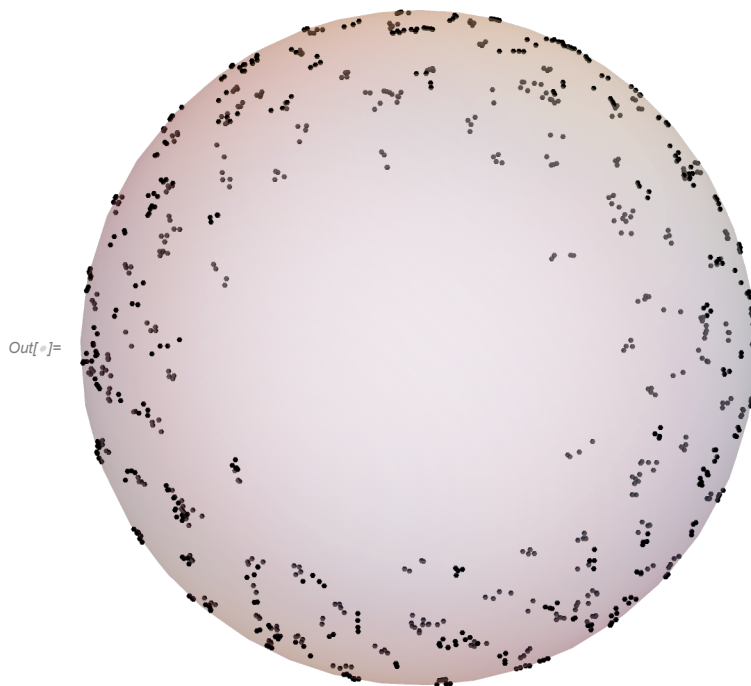

We set:

```
In[66]:= valIV = {J1 -> 1, J2 -> 1, J3 -> 1, Jp -> 1/5, Jc -> -1/5}
```

```
Out[66]= {J1 -> 1, J2 -> 1, J3 -> 1, Jp -> 1/5, Jc -> -1/5}
```

```
In[67]:= JB = Simplify[J /. {J1 -> 1, J2 -> 1, J3 -> 1}];
```

We start with the partition “IDENT” of the set  $\{1, \dots, 864\}$  of numbers of spin sites (according to the list “Sites” defined above) corresponding to an identification of numerically close spin vectors:

|     |     |     |     |
|-----|-----|-----|-----|
| 301 | 379 | 588 | 654 |
| 340 | 418 | 615 | 693 |
| 346 | 412 | 621 | 687 |
| 307 | 373 | 582 | 660 |
| 314 | 392 | 641 | 719 |

|     |     |     |     |
|-----|-----|-----|-----|
| 353 | 431 | 602 | 680 |
| 359 | 425 | 608 | 674 |
| 320 | 386 | 647 | 713 |
| 327 | 405 | 628 | 706 |
| 300 | 366 | 589 | 667 |
| 294 | 372 | 595 | 661 |
| 333 | 399 | 634 | 700 |
| 442 | 469 | 508 | 547 |
| 741 | 780 | 807 | 846 |
| 735 | 774 | 813 | 852 |
| 436 | 475 | 514 | 541 |
| 458 | 497 | 536 | 575 |
| 724 | 763 | 802 | 829 |
| 447 | 486 | 525 | 564 |
| 453 | 492 | 519 | 558 |
| 730 | 757 | 796 | 835 |
| 464 | 503 | 530 | 569 |
| 752 | 791 | 818 | 857 |
| 746 | 785 | 824 | 863 |
| 440 | 493 | 506 | 571 |
| 466 | 479 | 532 | 545 |
| 770 | 783 | 848 | 861 |
| 743 | 756 | 809 | 822 |
| 737 | 750 | 815 | 828 |
| 776 | 789 | 842 | 855 |
| 460 | 473 | 538 | 551 |
| 434 | 499 | 512 | 565 |
| 726 | 739 | 804 | 805 |
| 765 | 778 | 831 | 844 |
| 471 | 484 | 549 | 562 |
| 444 | 445 | 510 | 523 |
| 438 | 451 | 516 | 517 |
| 477 | 490 | 543 | 556 |
| 759 | 772 | 837 | 850 |
| 732 | 733 | 798 | 811 |
| 482 | 495 | 560 | 573 |
| 455 | 468 | 521 | 534 |
| 728 | 781 | 794 | 859 |
| 754 | 767 | 820 | 833 |
| 748 | 761 | 826 | 839 |
| 722 | 787 | 800 | 853 |
| 449 | 462 | 527 | 540 |
| 488 | 501 | 554 | 567 |
| 731 | 745 | 797 | 823 |
| 758 | 784 | 836 | 862 |
| 465 | 491 | 531 | 557 |
| 452 | 504 | 518 | 570 |
| 446 | 498 | 524 | 576 |
| 459 | 485 | 537 | 563 |
| 764 | 790 | 830 | 856 |
| 725 | 751 | 803 | 817 |
| 435 | 487 | 513 | 553 |
| 448 | 474 | 526 | 552 |
| 723 | 775 | 801 | 841 |
| 736 | 762 | 814 | 840 |

```

742 768 808 834
729 769 795 847
454 480 520 546
441 481 507 559
734 786 812 864
747 773 825 851
476 502 542 568
437 463 515 529
443 457 509 535
470 496 548 574
753 779 819 845
740 792 806 858
744 810 "" ""
771 849 "" ""
478 544 "" ""
439 505 "" ""
433 511 "" ""
472 550 "" ""
777 843 "" ""
738 816 "" ""
500 566 "" ""
461 539 "" ""
788 854 "" ""
749 827 "" ""
755 821 "" ""
782 860 "" ""
467 533 "" ""
494 572 "" ""
721 799 "" ""
760 838 "" ""
489 555 "" ""
450 528 "" ""
456 522 "" ""
483 561 "" ""
766 832 "" ""
727 793 "" ""
18 96 163 229
57 123 202 268
52 130 184 262
13 91 145 223
19 85 151 217
58 124 190 256
51 129 196 274
24 90 157 235
41 119 173 251
2 80 212 278
8 74 206 284
47 113 179 245
62 140 207 285
35 101 180 246
29 107 174 252
68 134 213 279
63 141 195 273
36 102 168 234;
In[68]:= IDENT = 32 100 167 240;

```

|     |     |     |     |
|-----|-----|-----|-----|
| 50  | 100 | 102 | 240 |
| 69  | 135 | 201 | 267 |
| 7   | 73  | 152 | 218 |
| 46  | 112 | 191 | 257 |
| 40  | 118 | 185 | 263 |
| 1   | 79  | 146 | 224 |
| 5   | 83  | 176 | 242 |
| 44  | 110 | 215 | 281 |
| 65  | 143 | 171 | 249 |
| 26  | 104 | 210 | 288 |
| 32  | 98  | 216 | 282 |
| 71  | 137 | 177 | 243 |
| 38  | 116 | 209 | 287 |
| 11  | 77  | 170 | 248 |
| 54  | 132 | 160 | 238 |
| 15  | 93  | 199 | 265 |
| 21  | 87  | 193 | 271 |
| 60  | 126 | 166 | 232 |
| 49  | 127 | 154 | 220 |
| 22  | 88  | 181 | 259 |
| 16  | 94  | 187 | 253 |
| 55  | 121 | 148 | 226 |
| 10  | 76  | 182 | 260 |
| 37  | 115 | 155 | 221 |
| 43  | 109 | 149 | 227 |
| 4   | 82  | 188 | 254 |
| 72  | 138 | 165 | 231 |
| 33  | 99  | 204 | 270 |
| 27  | 105 | 198 | 276 |
| 66  | 144 | 159 | 237 |
| 70  | 136 | 189 | 255 |
| 31  | 97  | 150 | 228 |
| 12  | 78  | 158 | 236 |
| 39  | 117 | 197 | 275 |
| 45  | 111 | 203 | 269 |
| 6   | 84  | 164 | 230 |
| 25  | 103 | 156 | 222 |
| 64  | 142 | 183 | 261 |
| 67  | 133 | 147 | 225 |
| 28  | 106 | 186 | 264 |
| 34  | 100 | 192 | 258 |
| 61  | 139 | 153 | 219 |
| 48  | 114 | 167 | 233 |
| 9   | 75  | 194 | 272 |
| 3   | 81  | 200 | 266 |
| 42  | 120 | 161 | 239 |
| 23  | 89  | 169 | 247 |
| 50  | 128 | 208 | 286 |
| 56  | 122 | 214 | 280 |
| 17  | 95  | 175 | 241 |
| 59  | 125 | 178 | 244 |
| 20  | 86  | 205 | 283 |
| 14  | 92  | 211 | 277 |
| 53  | 131 | 172 | 250 |
| 297 | 363 | 625 | 703 |
| --  | --  | --  | --  |

|     |     |     |     |
|-----|-----|-----|-----|
| 336 | 402 | 598 | 664 |
| 308 | 374 | 648 | 714 |
| 347 | 413 | 609 | 675 |
| 352 | 430 | 614 | 692 |
| 313 | 391 | 587 | 653 |
| 319 | 385 | 581 | 659 |
| 358 | 424 | 620 | 686 |
| 341 | 419 | 603 | 681 |
| 302 | 380 | 642 | 720 |
| 330 | 408 | 592 | 670 |
| 291 | 369 | 631 | 697 |
| 310 | 376 | 624 | 690 |
| 337 | 415 | 585 | 651 |
| 321 | 387 | 635 | 701 |
| 360 | 426 | 596 | 662 |
| 299 | 365 | 601 | 679 |
| 326 | 404 | 640 | 718 |
| 332 | 398 | 646 | 712 |
| 293 | 371 | 607 | 673 |
| 354 | 432 | 590 | 668 |
| 315 | 393 | 629 | 707 |
| 343 | 409 | 579 | 657 |
| 304 | 382 | 618 | 696 |
| 350 | 428 | 638 | 716 |
| 323 | 389 | 611 | 677 |
| 295 | 361 | 583 | 649 |
| 334 | 400 | 622 | 688 |
| 339 | 417 | 627 | 705 |
| 312 | 378 | 600 | 666 |
| 306 | 384 | 594 | 672 |
| 345 | 411 | 633 | 699 |
| 328 | 406 | 616 | 694 |
| 289 | 367 | 577 | 655 |
| 317 | 395 | 605 | 683 |
| 356 | 422 | 644 | 710 |
| 290 | 368 | 643 | 709 |
| 329 | 407 | 604 | 682 |
| 357 | 423 | 632 | 698 |
| 318 | 396 | 593 | 671 |
| 324 | 390 | 599 | 665 |
| 351 | 429 | 626 | 704 |
| 335 | 401 | 610 | 676 |
| 296 | 362 | 637 | 715 |
| 303 | 381 | 630 | 708 |
| 342 | 420 | 591 | 669 |
| 292 | 370 | 619 | 685 |
| 331 | 397 | 580 | 658 |
| 325 | 403 | 586 | 652 |
| 298 | 364 | 613 | 691 |
| 348 | 414 | 597 | 663 |
| 309 | 375 | 636 | 702 |
| 316 | 394 | 617 | 695 |
| 355 | 421 | 578 | 656 |
| 305 | 383 | 606 | 684 |
| 344 | 410 | 645 | 711 |

|     |     |     |     |
|-----|-----|-----|-----|
| 338 | 416 | 639 | 717 |
| 311 | 377 | 612 | 678 |
| 349 | 427 | 584 | 650 |
| 322 | 388 | 623 | 689 |

```
In[69]:= M = Length[IDENT]
```

```
Out[69]= 228
```

```
In[70]:= Sort[Flatten[IDENT]] == Range[NN]
```

```
Out[70]= True
```

The scalar product between spin vectors of the numerically determined ground state within the same set  $\text{IDENT}[[\mu]]$  always exceeds 0.993.

In the following we denote the  $M=228$  spin vectors by  $s[\mu]$ ,  $\mu=1, \dots, 228$ .

The next step is the symmetry analysis. The symmetry group  $G$  of the ground state of order 24 is generated by two reflections,

$$S1[1] = \begin{pmatrix} -1 & 0 & 0 \\ 0 & -1 & 0 \\ 0 & 0 & -1 \end{pmatrix}, \quad S2[1] = \begin{pmatrix} -1 & 0 & 0 \\ 0 & 1 & 0 \\ 0 & 0 & 1 \end{pmatrix},$$

and one rotation around the 3-axis with  $60^\circ$ ,

$$R[1] = \begin{pmatrix} \frac{1}{2} & -\frac{\sqrt{3}}{2} & 0 \\ \frac{\sqrt{3}}{2} & \frac{1}{2} & 0 \\ 0 & 0 & 1 \end{pmatrix}.$$

Let  $R[k]$ ,  $k=0, \dots, 5$ , denote the powers  $R[k] := (R[1])^k$ , analogously for  $S1[i]$  and  $S2[j]$ :

```
In[71]:= R[0] = {{1, 0, 0}, {0, 1, 0}, {0, 0, 1}};
```

$$R[1] = \left\{ \left\{ \frac{1}{2}, -\frac{\sqrt{3}}{2}, 0 \right\}, \left\{ \frac{\sqrt{3}}{2}, \frac{1}{2}, 0 \right\}, \{0, 0, 1\} \right\};$$

$$R[2] = \left\{ \left\{ -\frac{1}{2}, -\frac{\sqrt{3}}{2}, 0 \right\}, \left\{ \frac{\sqrt{3}}{2}, -\frac{1}{2}, 0 \right\}, \{0, 0, 1\} \right\};$$

$$R[3] = \left\{ \{-1, 0, 0\}, \{0, -1, 0\}, \{0, 0, 1\} \right\};$$

$$R[4] = \left\{ \left\{ -\frac{1}{2}, \frac{\sqrt{3}}{2}, 0 \right\}, \left\{ -\frac{\sqrt{3}}{2}, -\frac{1}{2}, 0 \right\}, \{0, 0, 1\} \right\};$$

$$R[5] = \left\{ \left\{ \frac{1}{2}, \frac{\sqrt{3}}{2}, 0 \right\}, \left\{ -\frac{\sqrt{3}}{2}, \frac{1}{2}, 0 \right\}, \{0, 0, 1\} \right\};$$

$$S1[0] = S2[0] = R[0];$$

$$S1[1] = \left\{ \{-1, 0, 0\}, \{0, -1, 0\}, \{0, 0, -1\} \right\};$$

$$S2[1] = \left\{ \{-1, 0, 0\}, \{0, 1, 0\}, \{0, 0, 1\} \right\};$$

These symmetries induce a further partition of the set of 228 spin vectors

into “orbits” of  $G$ . An “orbit” is the set of spin vectors obtained by applying all symmetries  $\text{symm} \in G$  to a given spin vector. We obtain 13 orbits  $\text{ORB}[i]$  of different size and choose one representative spin vector  $\text{rep}[i]$ ,  $i=1,\dots,13$  within each orbit.

For example:

```
In[80]:= Clear[ $\phi$ ];
```

```
In[81]:= ORB[1] = {{0, 0, 0, 32}, {0, 0, 1, 36}, {0, 0, 2, 42}, {0, 0, 3, 26},
  {0, 0, 4, 38}, {0, 0, 5, 48}, {0, 1, 0, 28}, {0, 1, 1, 40}, {0, 1, 2, 46},
  {0, 1, 3, 30}, {0, 1, 4, 34}, {0, 1, 5, 44}, {1, 0, 0, 25}, {1, 0, 1, 37},
  {1, 0, 2, 47}, {1, 0, 3, 31}, {1, 0, 4, 35}, {1, 0, 5, 41}, {1, 1, 0, 29},
  {1, 1, 1, 33}, {1, 1, 2, 43}, {1, 1, 3, 27}, {1, 1, 4, 39}, {1, 1, 5, 45}};
```

```
In[82]:= rep[1] = {Cos[ $\phi$ [1]]  $\sqrt{1 - z[1]^2}$ , Sin[ $\phi$ [1]]  $\sqrt{1 - z[1]^2}$ , z[1]};
```

```
In[83]:= Length[ORB[1]]
```

```
Out[83]= 24
```

This notation means the following: The element  $\{i,j,k,\mu\}$  of  $\text{ORB}[1]$  represents the spin vector  $s[\mu]=S1[j] S2[j] R[k] \text{rep}[1]$ . The first element of  $\text{ORB}[1]$  is  $\{0,0,0,32\}$  and hence  $\text{rep}[1]=s[32]$  is the representative spin vector of  $\text{ORB}[1]$ . The numerical findings do not indicate any simplified value for  $\text{rep}[1]$  and thus we represent  $\text{rep}[1]$  completely general as a function of two parameters  $z[1]$  and  $\phi[1]$ , its 3rd coordinate and its azimuthal angle. All symmetries applied to  $\text{rep}[1]$  generate new spin vectors and hence the length of the orbit  $\text{ORB}[1]$  equals the order of  $G$ , which is 24.

Recall that  $\text{rep}[1]=s[32]$  is the common spin vector of 4 spin sites with numbers  $\{434,499,512,565\}$ :

```
In[84]:= IDENT[[32]]
```

```
Out[84]= {434, 499, 512, 565}
```

Hence we will define:

```
In[85]:= S[434] = S[499] = S[512] = S[565] = rep[1];
```

More generally, taking into account the symmetries, this definition can be extended to all spin sites belonging to spin vectors occurring in the orbit ORB[1]:

```
In[86]:= For[a = 1, a ≤ Length[ORB[1]], a++, {i, j, k, μ} = ORB[1][[a]];
part = IDENT[[μ]];
symm = S1[i].S2[j].R[k];
For[b = 1, b ≤ Length[part], b++, S[part[[b]]] = symm.rep[1]]]
```

Let us check one spin site corresponding to the last element of ORB[1]:

```
In[87]:= ORB[1][[-1, 4]]
```

```
Out[87]= 45
```

```
In[88]:= IDENT[[45]]
```

```
Out[88]= {748, 761, 826, 839}
```

```
In[89]:= S[748]
```

```
Out[89]= { 1/2 Cos[φ[1]] √(1 - z[1]^2) + 1/2 √3 Sin[φ[1]] √(1 - z[1]^2),
1/2 √3 Cos[φ[1]] √(1 - z[1]^2) - 1/2 Sin[φ[1]] √(1 - z[1]^2), -z[1]}
```

The above procedure will be repeated for the other orbits. We first consider ORB[2] and ORB[3]:

```
In[90]:= ORB[2] = {{0, 0, 0, 56}, {0, 0, 1, 60}, {0, 0, 2, 66}, {0, 0, 3, 50},
{0, 0, 4, 62}, {0, 0, 5, 72}, {0, 1, 0, 52}, {0, 1, 1, 64}, {0, 1, 2, 70},
{0, 1, 3, 54}, {0, 1, 4, 58}, {0, 1, 5, 68}, {1, 0, 0, 49}, {1, 0, 1, 61},
{1, 0, 2, 71}, {1, 0, 3, 55}, {1, 0, 4, 59}, {1, 0, 5, 65}, {1, 1, 0, 53},
{1, 1, 1, 57}, {1, 1, 2, 67}, {1, 1, 3, 51}, {1, 1, 4, 63}, {1, 1, 5, 69}};
```

```
In[91]:= rep[2] = {Cos[φ[2]] √(1 - z[2]^2), Sin[φ[2]] √(1 - z[2]^2), z[2]};
```

```
In[92]:= For[a = 1, a ≤ Length[ORB[2]], a++, {i, j, k, μ} = ORB[2][[a]];
part = IDENT[[μ]];
symm = S1[i].S2[j].R[k];
For[b = 1, b ≤ Length[part], b++, S[part[[b]]] = symm.rep[2]]]
```

```
In[93]:=
```

```
In[94]:= ORB[3] = {{0, 0, 0, 80}, {0, 0, 1, 84}, {0, 0, 2, 90}, {0, 0, 3, 74},
{0, 0, 4, 86}, {0, 0, 5, 96}, {0, 1, 0, 76}, {0, 1, 1, 88}, {0, 1, 2, 94},
{0, 1, 3, 78}, {0, 1, 4, 82}, {0, 1, 5, 92}, {1, 0, 0, 73}, {1, 0, 1, 85},
{1, 0, 2, 95}, {1, 0, 3, 79}, {1, 0, 4, 83}, {1, 0, 5, 89}, {1, 1, 0, 77},
{1, 1, 1, 81}, {1, 1, 2, 91}, {1, 1, 3, 75}, {1, 1, 4, 87}, {1, 1, 5, 93}};
```

```
In[95]:= rep[3] = {Cos[φ[3]] √(1 - z[3]^2), Sin[φ[3]] √(1 - z[3]^2), z[3]};
```

```
In[96]:= For[a = 1, a ≤ Length[ORB[3]], a++, {i, j, k, μ} = ORB[3][[a]];
part = IDENT[μ];
symm = S1[i].S2[j].R[k];
For[b = 1, b ≤ Length[part], b++, S[part[[b]]] = symm.rep[3]]]
```

The 4th orbit is different in kind. It contains all spin vectors with  $z=0$ . Hence the reflection

$$S1[1] = \begin{pmatrix} -1 & 0 & 0 \\ 0 & -1 & 0 \\ 0 & 0 & -1 \end{pmatrix} \text{ and the rotation } R[3] = \begin{pmatrix} -1 & 0 & 0 \\ 0 & -1 & 0 \\ 0 & 0 & 1 \end{pmatrix} \text{ have the same}$$

effect and we obtain only 12 different spin vectors in this orbit.

We use a different coding for ORB[4]:  $\{j, k, \mu\} \in \text{ORB}[4]$  means that  $s[\mu] = S2[j] R[k] \text{rep}[4]$ .

```
In[97]:= ORB[4] = {{0, 0, 16}, {0, 1, 19}, {0, 2, 17}, {0, 3, 13}, {0, 4, 20}, {0, 5, 22},
{1, 0, 14}, {1, 1, 21}, {1, 2, 24}, {1, 3, 15}, {1, 4, 18}, {1, 5, 23}};
```

```
In[98]:= Length[ORB[4]]
```

```
Out[98]= 12
```

```
In[99]:= rep[4] = {Cos[φ[4]], Sin[φ[4]], 0};
```

```
In[100]:= For[a = 1, a ≤ Length[ORB[4]], a++, {j, k, μ} = ORB[4][[a]];
part = IDENT[μ];
symm = S2[j].R[k];
For[b = 1, b ≤ Length[part], b++, S[part[[b]]] = symm.rep[4]]]
```

The next 3 orbits are of the same kind as before:

```
In[101]:= ORB[5] = {{0, 0, 0, 104}, {0, 0, 1, 110}, {0, 0, 2, 118}, {0, 0, 3, 98},
{0, 0, 4, 112}, {0, 0, 5, 120}, {0, 1, 0, 100}, {0, 1, 1, 106}, {0, 1, 2, 116},
{0, 1, 3, 102}, {0, 1, 4, 108}, {0, 1, 5, 114}, {1, 0, 0, 97}, {1, 0, 1, 111},
{1, 0, 2, 119}, {1, 0, 3, 103}, {1, 0, 4, 109}, {1, 0, 5, 117}, {1, 1, 0, 101},
{1, 1, 1, 107}, {1, 1, 2, 113}, {1, 1, 3, 99}, {1, 1, 4, 105}, {1, 1, 5, 115}};
```

```
In[102]:= rep[5] = {Cos[φ[5]] √(1 - z[5]2), Sin[φ[5]] √(1 - z[5]2), z[5]};
```

```
In[103]:= For[a = 1, a ≤ Length[ORB[5]], a++, {i, j, k, μ} = ORB[5][[a]];
part = IDENT[μ];
symm = S1[i].S2[j].R[k];
For[b = 1, b ≤ Length[part], b++, S[part[[b]]] = symm.rep[5]]]
```

```
In[104]:=
```

```
In[105]:= ORB[6] = {{0, 0, 0, 128}, {0, 0, 1, 134}, {0, 0, 2, 142}, {0, 0, 3, 122},
{0, 0, 4, 136}, {0, 0, 5, 144}, {0, 1, 0, 124}, {0, 1, 1, 130}, {0, 1, 2, 140},
{0, 1, 3, 126}, {0, 1, 4, 132}, {0, 1, 5, 138}, {1, 0, 0, 121}, {1, 0, 1, 135},
{1, 0, 2, 143}, {1, 0, 3, 127}, {1, 0, 4, 133}, {1, 0, 5, 141}, {1, 1, 0, 125},
{1, 1, 1, 131}, {1, 1, 2, 137}, {1, 1, 3, 123}, {1, 1, 4, 129}, {1, 1, 5, 139}};
```

```
In[106]:= rep[6] = {Cos[φ[6]] √{1 - z[6]2}, Sin[φ[6]] √{1 - z[6]2}, z[6]};
```

```
In[107]:= For[a = 1, a ≤ Length[ORB[6]], a++, {i, j, k, μ} = ORB[6][[a]];
part = IDENT[μ];
symm = S1[i].S2[j].R[k];
For[b = 1, b ≤ Length[part], b++, S[part[[b]]] = symm.rep[6]]]
```

```
In[108]:=
```

```
In[109]:= ORB[7] = {{0, 0, 0, 152}, {0, 0, 1, 158}, {0, 0, 2, 166}, {0, 0, 3, 146},
{0, 0, 4, 160}, {0, 0, 5, 168}, {0, 1, 0, 148}, {0, 1, 1, 154}, {0, 1, 2, 164},
{0, 1, 3, 150}, {0, 1, 4, 156}, {0, 1, 5, 162}, {1, 0, 0, 145}, {1, 0, 1, 159},
{1, 0, 2, 167}, {1, 0, 3, 151}, {1, 0, 4, 157}, {1, 0, 5, 165}, {1, 1, 0, 149},
{1, 1, 1, 155}, {1, 1, 2, 161}, {1, 1, 3, 147}, {1, 1, 4, 153}, {1, 1, 5, 163}};
```

```
In[110]:= rep[7] = {Cos[φ[7]] √{1 - z[7]2}, Sin[φ[7]] √{1 - z[7]2}, z[7]};
```

```
In[111]:= For[a = 1, a ≤ Length[ORB[7]], a++, {i, j, k, μ} = ORB[7][[a]];
part = IDENT[μ];
symm = S1[i].S2[j].R[k];
For[b = 1, b ≤ Length[part], b++, S[part[[b]]] = symm.rep[7]]]
```

For the remaining orbits the numerical findings indicate that the representative spins can be chosen as  $\text{rep}[a] = \{ \sqrt{1 - z[a]^2}, 0, z[a] \}$  for  $a=8,9,10$  and  $\text{rep}[a] = \{ 0, \sqrt{1 - z[a]^2}, z[a] \}$  for  $a=11,12,13$ .

Hence the reflection

$S2[1] = \begin{pmatrix} -1 & 0 & 0 \\ 0 & 1 & 0 \\ 0 & 0 & 1 \end{pmatrix}$  has the same effect as a suitable rotation and we obtain

only 12 different spin vectors for these orbits. We use a different coding for ORB[a]:

$\{i, k, \mu\} \in \text{ORB}[a]$  means that  $s[\mu] = S1[i] R[k] \text{rep}[a]$  for  $a=8, \dots, 13$ .

```
In[112]:= ORB[8] = {{0, 0, 180}, {0, 1, 178}, {0, 2, 174}, {0, 3, 170}, {0, 4, 172}, {0, 5, 176},
{1, 0, 169}, {1, 1, 171}, {1, 2, 175}, {1, 3, 179}, {1, 4, 177}, {1, 5, 173}};
```

```
In[113]:= rep[8] = {√{1 - z[8]2}, 0, z[8]};
```

```
In[114]:= For[a = 1, a ≤ Length[ORB[8]], a++, {i, k, μ} = ORB[8][[a]];
part = IDENT[μ];
symm = S1[i].R[k];
For[b = 1, b ≤ Length[part], b++, S[part[[b]]] = symm.rep[8]]]
```

```
In[115]:=
```

```
In[116]:= ORB[9] = {{0, 0, 192}, {0, 1, 190}, {0, 2, 186}, {0, 3, 182}, {0, 4, 184}, {0, 5, 188},
               {1, 0, 181}, {1, 1, 183}, {1, 2, 187}, {1, 3, 191}, {1, 4, 189}, {1, 5, 185}};
```

```
In[117]:= rep[9] = { $\sqrt{1 - z[9]^2}$ , 0, z[9]};
```

```
In[118]:= For[a = 1, a ≤ Length[ORB[9]], a++, {i, k, μ} = ORB[9][[a]];
           part = IDENT[μ];
           symm = S1[i].R[k];
           For[b = 1, b ≤ Length[part], b++, S[part[[b]]] = symm.rep[9]]]
```

```
In[119]:=
```

```
In[120]:= ORB[10] = {{0, 0, 204}, {0, 1, 202}, {0, 2, 198}, {0, 3, 194}, {0, 4, 196}, {0, 5, 200},
                   {1, 0, 193}, {1, 1, 195}, {1, 2, 199}, {1, 3, 203}, {1, 4, 201}, {1, 5, 197}};
```

```
In[121]:= rep[10] = { $\sqrt{1 - z[10]^2}$ , 0, z[10]};
```

```
In[122]:= For[a = 1, a ≤ Length[ORB[10]], a++, {i, k, μ} = ORB[10][[a]];
           part = IDENT[μ];
           symm = S1[i].R[k];
           For[b = 1, b ≤ Length[part], b++, S[part[[b]]] = symm.rep[10]]]
```

```
In[123]:=
```

```
In[124]:= ORB[11] = {{0, 0, 4}, {0, 1, 208}, {0, 2, 206}, {0, 3, 2}, {0, 4, 210}, {0, 5, 212},
                   {1, 0, 1}, {1, 1, 209}, {1, 2, 211}, {1, 3, 3}, {1, 4, 207}, {1, 5, 205}};
```

```
In[125]:= rep[11] = {0,  $\sqrt{1 - z[11]^2}$ , z[11]};
```

```
In[126]:= For[a = 1, a ≤ Length[ORB[11]], a++, {i, k, μ} = ORB[11][[a]];
           part = IDENT[μ];
           symm = S1[i].R[k];
           For[b = 1, b ≤ Length[part], b++, S[part[[b]]] = symm.rep[11]]]
```

```
In[127]:=
```

```
In[128]:= ORB[12] = {{0, 0, 8}, {0, 1, 216}, {0, 2, 214}, {0, 3, 6}, {0, 4, 218}, {0, 5, 220},
                   {1, 0, 5}, {1, 1, 217}, {1, 2, 219}, {1, 3, 7}, {1, 4, 215}, {1, 5, 213}};
```

```
In[129]:= rep[12] = {0,  $\sqrt{1 - z[12]^2}$ , z[12]};
```

```
In[130]:= For[a = 1, a ≤ Length[ORB[12]], a++, {i, k, μ} = ORB[12][[a]];
           part = IDENT[μ];
           symm = S1[i].R[k];
           For[b = 1, b ≤ Length[part], b++, S[part[[b]]] = symm.rep[12]]]
```

```
In[131]:=
```

```
In[132]:= ORB[13] = {{0, 0, 12}, {0, 1, 224}, {0, 2, 222}, {0, 3, 10}, {0, 4, 226}, {0, 5, 228},
                   {1, 0, 9}, {1, 1, 225}, {1, 2, 227}, {1, 3, 11}, {1, 4, 223}, {1, 5, 221}};
```

```

In[133]:= rep[13] = {0,  $\sqrt{1 - z[13]^2}$ , z[13]};

In[134]:= For[a = 1, a ≤ Length[ORB[13]], a++, {i, k, μ} = ORB[13][[a]];
           part = IDENT[μ];
           symm = S1[i].R[k];
           For[b = 1, b ≤ Length[part], b++, S[part[[b]]] = symm.rep[13]]

```

This concludes the enumeration of all orbits. We will check that the set of all spin vectors is thereby exhausted:

```

In[135]:= Sort[Union[Flatten[Table[ORB[i][[a, 4]], {i, {1, 2, 3, 5, 6, 7}}, {a, 24}]],
                Flatten[Table[ORB[i][[a, 3]], {i, {4, 8, 9, 10, 11, 12, 13}}, {a, 12}]]] == Range[228]

Out[135]= True

```

Now we can calculate the energy (per site) EIV as a function of Jp, Jc and the 19 parameters

{z[1],z[2],z[3],z[5],...,z[13],φ[1],...,φ[7]}:

$$\begin{aligned}
 \text{In[136]:= EIV} &= \text{Simplify}\left[\frac{1}{2 \text{NN}} \text{Sum}[\text{JB}[\mu, \nu] \times \mathbf{S}[\mu] \cdot \mathbf{S}[\nu], \{\mu, \text{NN}\}, \{\nu, \text{NN}\}]\right] \\
 \text{Out[136]=} &\frac{1}{36} \times \left( 2 \text{Jc} - \text{Jc} \cos[2 \phi[3]] + \text{Jc} \cos[2 \phi[4]] - 2 \text{Jp} \cos[2 \phi[5]] - \text{Jp} \cos[2 \phi[6]] + \right. \\
 &\sqrt{3} \text{Jc} \sin[2 \phi[1]] - \sqrt{3} \text{Jp} \sin[2 \phi[6]] + 2 \text{Jc} z[1]^2 - \sqrt{3} \text{Jc} \sin[2 \phi[1]] z[1]^2 + \\
 &\text{Jc} \cos[2 \phi[1]] (-1 + z[1]^2) + 2 \text{Jc} z[2]^2 + 2 \text{Jc} \cos[2 \phi[2]] (-1 + z[2]^2) + \text{Jc} z[3]^2 + \\
 &\text{Jc} \cos[2 \phi[3]] z[3]^2 + 4 z[1] \times z[5] - 4 z[3] \times z[5] + 2 \text{Jp} z[5]^2 + 2 \text{Jp} \cos[2 \phi[5]] z[5]^2 - \\
 &2 \sin[\phi[1] - \phi[5]] \sqrt{3 - 3 z[1]^2} \sqrt{1 - z[5]^2} + 2 \cos[\phi[1] - \phi[5]] \sqrt{1 - z[1]^2} \sqrt{1 - z[5]^2} - \\
 &4 \cos[\phi[3] - \phi[5]] \sqrt{1 - z[3]^2} \sqrt{1 - z[5]^2} - 4 z[2] \times z[6] - 2 \text{Jp} z[6]^2 + \\
 &\text{Jp} \cos[2 \phi[6]] z[6]^2 + \sqrt{3} \text{Jp} \sin[2 \phi[6]] z[6]^2 - 2 \sin[\phi[4] - \phi[6]] \sqrt{3 - 3 z[6]^2} - \\
 &2 \cos[\phi[4] - \phi[6]] \sqrt{1 - z[6]^2} - 4 \cos[\phi[2] - \phi[6]] \sqrt{1 - z[2]^2} \sqrt{1 - z[6]^2} - \\
 &4 z[1] \times z[7] + 4 z[2] \times z[7] - 4 \text{Jp} z[5] \times z[7] - 4 \text{Jp} z[6] \times z[7] - \\
 &2 \sin[\phi[1] - \phi[7]] \sqrt{3 - 3 z[1]^2} \sqrt{1 - z[7]^2} + 2 \cos[\phi[1] - \phi[7]] \sqrt{1 - z[1]^2} \sqrt{1 - z[7]^2} - \\
 &4 \cos[\phi[2] - \phi[7]] \sqrt{1 - z[2]^2} \sqrt{1 - z[7]^2} - 2 \text{Jp} \sin[\phi[5] + \phi[7]] \sqrt{3 - 3 z[5]^2} \sqrt{1 - z[7]^2} - \\
 &2 \text{Jp} \cos[\phi[5] + \phi[7]] \sqrt{1 - z[5]^2} \sqrt{1 - z[7]^2} - \\
 &4 \text{Jp} \cos[\phi[6] + \phi[7]] \sqrt{1 - z[6]^2} \sqrt{1 - z[7]^2} - 4 z[2] \times z[8] - 4 z[7] \times z[8] - \\
 &2 \sin[\phi[2]] \sqrt{3 - 3 z[2]^2} \sqrt{1 - z[8]^2} + 2 \cos[\phi[2]] \sqrt{1 - z[2]^2} \sqrt{1 - z[8]^2} + \\
 &2 \sin[\phi[7]] \sqrt{3 - 3 z[7]^2} \sqrt{1 - z[8]^2} - 2 \cos[\phi[7]] \sqrt{1 - z[7]^2} \sqrt{1 - z[8]^2} + \\
 &4 z[2] \times z[9] - 4 z[6] \times z[9] - 2 \text{Jc} z[9]^2 - 2 \sin[\phi[2]] \sqrt{3 - 3 z[2]^2} \sqrt{1 - z[9]^2} + \\
 &2 \cos[\phi[2]] \sqrt{1 - z[2]^2} \sqrt{1 - z[9]^2} + 2 \sin[\phi[6]] \sqrt{3 - 3 z[6]^2} \sqrt{1 - z[9]^2} - \\
 &2 \cos[\phi[6]] \sqrt{1 - z[6]^2} \sqrt{1 - z[9]^2} - 4 z[3] \times z[10] + 4 z[5] \times z[10] + \\
 &2 \text{Jc} z[8] \times z[10] - 2 \sin[\phi[3]] \sqrt{3 - 3 z[3]^2} \sqrt{1 - z[10]^2} + \\
 &2 \cos[\phi[3]] \sqrt{1 - z[3]^2} \sqrt{1 - z[10]^2} + 2 \sin[\phi[5]] \sqrt{3 - 3 z[5]^2} \sqrt{1 - z[10]^2} - \\
 &2 \cos[\phi[5]] \sqrt{1 - z[5]^2} \sqrt{1 - z[10]^2} + 2 \text{Jc} \sqrt{1 - z[8]^2} \sqrt{1 - z[10]^2} - \\
 &4 z[1] \times z[11] - 4 z[5] \times z[11] - 2 \cos[\phi[1]] \sqrt{3 - 3 z[1]^2} \sqrt{1 - z[11]^2} - \\
 &2 \sin[\phi[1]] \sqrt{1 - z[1]^2} \sqrt{1 - z[11]^2} - 4 \sin[\phi[5]] \sqrt{1 - z[5]^2} \sqrt{1 - z[11]^2} - \\
 &4 z[6] \times z[12] - 2 \cos[\phi[4]] \sqrt{3 - 3 z[12]^2} + 2 \sin[\phi[4]] \sqrt{1 - z[12]^2} - \\
 &4 \sin[\phi[6]] \sqrt{1 - z[6]^2} \sqrt{1 - z[12]^2} + 4 z[1] \times z[13] - 4 z[7] \times z[13] - 2 \text{Jc} z[12] \times z[13] - \\
 &2 \cos[\phi[1]] \sqrt{3 - 3 z[1]^2} \sqrt{1 - z[13]^2} - 2 \sin[\phi[1]] \sqrt{1 - z[1]^2} \sqrt{1 - z[13]^2} - \\
 &4 \sin[\phi[7]] \sqrt{1 - z[7]^2} \sqrt{1 - z[13]^2} + 2 \text{Jc} \sqrt{1 - z[12]^2} \sqrt{1 - z[13]^2} \Big)
 \end{aligned}$$

The numerical ground state data yield the following approximation for the parameters :

$$\begin{aligned}
 \text{In[137]:= rule} &= \{z[1] \rightarrow 0.37888, \phi[1] \rightarrow 1.4119, z[2] \rightarrow 0.18786, \phi[2] \rightarrow 1.2715, z[3] \rightarrow 0.4806, \\
 &\phi[3] \rightarrow 1.1812, \phi[4] \rightarrow 0.27302, z[5] \rightarrow 0.32466, \phi[5] \rightarrow 0.086545, z[6] \rightarrow 0.56987, \\
 &\phi[6] \rightarrow 0.20111, z[7] \rightarrow 0.52427, \phi[7] \rightarrow 0.48269, z[8] \rightarrow 0.65653, z[9] \rightarrow 0.33587, \\
 &z[10] \rightarrow 0.18627, z[11] \rightarrow 0.76046, z[12] \rightarrow 0.52009, z[13] \rightarrow 0.084699\};
 \end{aligned}$$

The corresponding value of the minimal energy (per site) at  $\{J_p \rightarrow \frac{1}{5}, J_c \rightarrow -\frac{1}{5}\}$  is:

```
In[138]:= valIV
```

```
Out[138]:= {J1 → 1, J2 → 1, J3 → 1, Jp →  $\frac{1}{5}$ , Jc →  $-\frac{1}{5}$ }
```

```
In[139]:= ee1 = EIV /. valIV /. rule
```

```
Out[139]:= -1.10491
```

This energy can be further decreased by using the command FindMinimum[...]:

```
In[140]:= ini = Table[Apply[List, rule[[i]]], {i, Length[rule]}]
```

```
Out[140]:= {{z[1], 0.378881}, {φ[1], 1.41187}, {z[2], 0.187857},
{φ[2], 1.27146}, {z[3], 0.480604}, {φ[3], 1.18124}, {φ[4], 0.27302},
{z[5], 0.324658}, {φ[5], 0.0865451}, {z[6], 0.569872}, {φ[6], 0.201108},
{z[7], 0.524272}, {φ[7], 0.482686}, {z[8], 0.656527}, {z[9], 0.335866},
{z[10], 0.186274}, {z[11], 0.760458}, {z[12], 0.520089}, {z[13], 0.0846993}}
```

```
In[141]:= {ee2, rulenew} =
```

```
FindMinimum[{EIV /. valIV, -1 < z[1] < 1 && -1 < z[2] < 1 && -1 < z[3] < 1 &&
-1 < z[5] < 1 && -1 < z[6] < 1 && -1 < z[7] < 1 && -1 < z[8] < 1 && -1 < z[9] < 1 &&
-1 < z[10] < 1 && -1 < z[11] < 1 && -1 < z[12] < 1 && -1 < z[13] < 1}, ini]
```

```
Out[141]:= {-1.10525,
{z[1] → 0.388118, φ[1] → 1.41618, z[2] → 0.181714, φ[2] → 1.27991, z[3] → 0.475637,
φ[3] → 1.17642, φ[4] → 0.277265, z[5] → 0.342232, φ[5] → 0.0653045, z[6] → 0.577961,
φ[6] → 0.189554, z[7] → 0.525727, φ[7] → 0.473656, z[8] → 0.665262, z[9] → 0.33061,
z[10] → 0.191503, z[11] → 0.75233, z[12] → 0.514554, z[13] → 0.0816232}}
```

The obtained value of ee2=-1.10525 is slightly below the Monte-Carlo minimal energy of  $e_{MC} = -1.10514$ , which confirms the above calculations.

Finally, we present a common origin plot of the reconstructed ground state to be compared with the initial plot of the numerical ground state:

```
In[142]:= G1 = Graphics3D[Table[Point[S[μ] /. rulenew], {μ, NN}]];
```

```
In[143]:= PC = ParametricPlot3D[
Join[Table[{Cos[α]  $\sqrt{1 - z[i]^2}$ , Sin[α]  $\sqrt{1 - z[i]^2}$ , z[i]} /. rulenew,
{i, {1, 2, 3, 5, 6, 7, 8, 9, 10, 11, 12, 13}}],
Table[{Cos[α]  $\sqrt{1 - z[i]^2}$ , Sin[α]  $\sqrt{1 - z[i]^2}$ , -z[i]} /. rulenew,
{i, {1, 2, 3, 5, 6, 7, 8, 9, 10, 11, 12, 13}}]], {α, 0, 2π}, PlotStyle → Thin];
```

```
In[144]:= SP = Graphics3D[{Opacity[0.25], Sphere[]},  
    Boxed → False, PlotRange → {{-1, 1}, {-1, 1}, {-1, 1}}];  
  
In[145]:= Show[SP, PC, G1, ViewPoint → {0, 0, 5}, Boxed → False, Axes → False]
```

Out[145]=

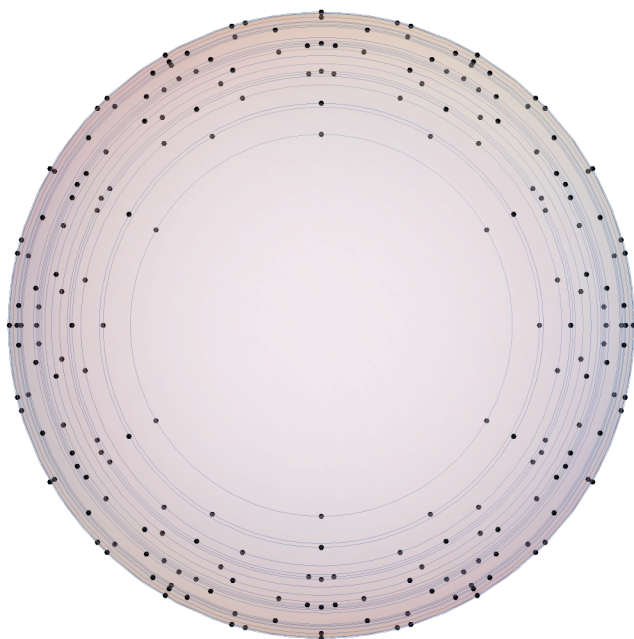

## Phase IX

Since the procedure is analogous to that of the phases IV and V we will only present the results. For the values  $\{J_1 \rightarrow 1, J_2 \rightarrow 1, J_3 \rightarrow 1, J_p \rightarrow -\frac{1}{5}, J_c \rightarrow 1\}$  the common origin plot of the numerically determined ground state looks as follows, viewed from “above”:

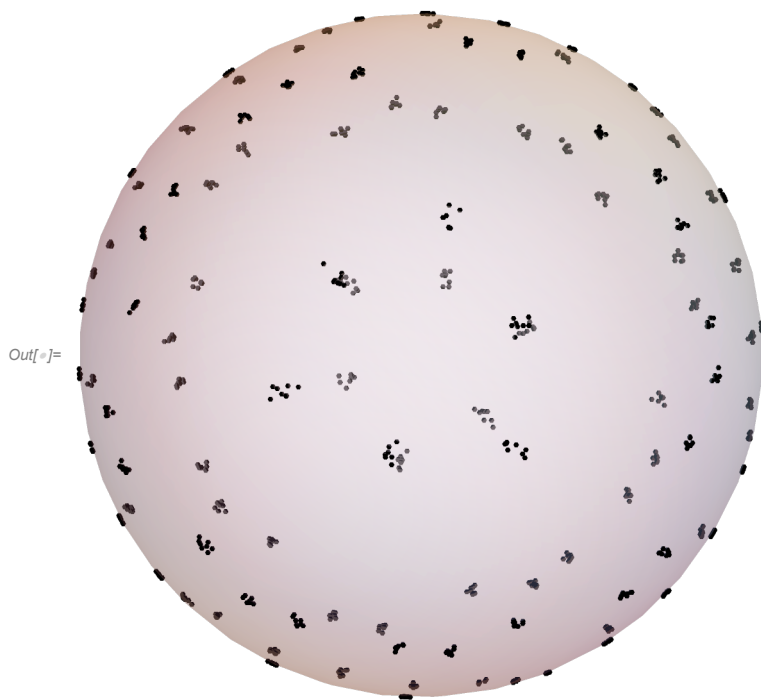

If we identify points that are close to each other, we find that there are only  $M=108$  different spin vectors. The symmetry group of this state is generated by a point reflection (antipodal symmetry) and rotations with an angle of  $120^\circ$  around the vertical symmetry axis. This results in 18 orbits with  $K=18$  representative spin vectors described by 36 parameters  $z[i], \phi[i], i=1, \dots, 18$ . Due to a number of simplifications suggested by the numerical findings the list of parameters can be reduced to the following of length 26:

```
In[146]:= VAR = {z[1], z[2], z[3], z[4], z[5], z[6], z[11], z[12], z[13], z[14],  $\phi$ [1],  $\phi$ [2],  $\phi$ [3],
 $\phi$ [4],  $\phi$ [5],  $\phi$ [7],  $\phi$ [8],  $\phi$ [9],  $\phi$ [10],  $\phi$ [11],  $\phi$ [12],  $\phi$ [13],  $\phi$ [15],  $\phi$ [16],  $\phi$ [17],  $\phi$ [18]}
Out[146]:= {z[1], z[2], z[3], z[4], z[5], z[6], z[11], z[12], z[13], z[14],  $\phi$ [1],  $\phi$ [2],  $\phi$ [3],  $\phi$ [4],
 $\phi$ [5],  $\phi$ [7],  $\phi$ [8],  $\phi$ [9],  $\phi$ [10],  $\phi$ [11],  $\phi$ [12],  $\phi$ [13],  $\phi$ [15],  $\phi$ [16],  $\phi$ [17],  $\phi$ [18]}

In[147]:= Length[VAR]
Out[147]:= 26
```

The total energy (per site) as a function of  $J_p, J_c$  and the 26 parameters assumes the following form:

$$\begin{aligned} \text{In[148]:= EIX} = & \frac{1}{36} \left( J_p - 4 z[1] \times z[2] + 4 J_p z[2]^2 + \sin[\phi[1] - \phi[9]] \sqrt{3 - 3 z[1]^2} \sqrt{1 - z[2]^2} + \right. \\ & \sin[\phi[2] - \phi[10]] \sqrt{3 - 3 z[1]^2} \sqrt{1 - z[2]^2} + \cos[\phi[1] - \phi[9]] \sqrt{1 - z[1]^2} \sqrt{1 - z[2]^2} + \\ & \cos[\phi[2] - \phi[10]] \sqrt{1 - z[1]^2} \sqrt{1 - z[2]^2} - J_p \cos[\phi[2] - \phi[9]] (-1 + z[2]^2) + \\ & \sqrt{3} J_p \sin[\phi[2] - \phi[9]] (-1 + z[2]^2) + \sin[\phi[3] - \phi[18]] \sqrt{3 - 3 z[3]^2} + \\ & \sin[\phi[8] - \phi[18]] \sqrt{3 - 3 z[3]^2} - \cos[\phi[3] - \phi[18]] \sqrt{1 - z[3]^2} + \\ & \cos[\phi[8] - \phi[18]] \sqrt{1 - z[3]^2} - 4 J_c z[1] \times z[4] + 4 z[2] \times z[4] - \\ & 2 J_c \cos[\phi[1] - \phi[4]] \sqrt{1 - z[1]^2} \sqrt{1 - z[4]^2} - 2 J_c \cos[\phi[7] - \phi[10]] \\ & \sqrt{1 - z[1]^2} \sqrt{1 - z[4]^2} + \sin[\phi[2] - \phi[4]] \sqrt{3 - 3 z[2]^2} \sqrt{1 - z[4]^2} + \\ & \sin[\phi[7] - \phi[9]] \sqrt{3 - 3 z[2]^2} \sqrt{1 - z[4]^2} - \cos[\phi[2] - \phi[4]] \sqrt{1 - z[2]^2} \sqrt{1 - z[4]^2} - \\ & \cos[\phi[7] - \phi[9]] \sqrt{1 - z[2]^2} \sqrt{1 - z[4]^2} + 4 z[4] \times z[5] - \\ & \sin[\phi[4] - \phi[5]] \sqrt{3 - 3 z[4]^2} \sqrt{1 - z[5]^2} - \sin[\phi[5] - \phi[7]] \sqrt{3 - 3 z[4]^2} \sqrt{1 - z[5]^2} - \\ & \cos[\phi[4] - \phi[5]] \sqrt{1 - z[4]^2} \sqrt{1 - z[5]^2} - \cos[\phi[5] - \phi[7]] \sqrt{1 - z[4]^2} \sqrt{1 - z[5]^2} - \\ & 4 z[1] \times z[6] + 2 J_p z[5] \times z[6] + \sin[\phi[1] - \phi[5]] \sqrt{3 - 3 z[1]^2} \sqrt{1 - z[6]^2} + \\ & \sin[\phi[5] - \phi[10]] \sqrt{3 - 3 z[1]^2} \sqrt{1 - z[6]^2} + \cos[\phi[1] - \phi[5]] \sqrt{1 - z[1]^2} \sqrt{1 - z[6]^2} + \\ & \cos[\phi[5] - \phi[10]] \sqrt{1 - z[1]^2} \sqrt{1 - z[6]^2} + 2 J_p \sqrt{1 - z[5]^2} \sqrt{1 - z[6]^2} - 4 z[1] \times z[11] + \\ & 4 z[2] \times z[11] + 4 z[3] \times z[11] + \sin[\phi[10] - \phi[17]] \sqrt{3 - 3 z[1]^2} \sqrt{1 - z[11]^2} - \\ & 2 \cos[\phi[1] - \phi[11]] \sqrt{1 - z[1]^2} \sqrt{1 - z[11]^2} + \cos[\phi[10] - \phi[17]] \\ & \sqrt{1 - z[1]^2} \sqrt{1 - z[11]^2} + \sin[\phi[9] - \phi[11]] \sqrt{3 - 3 z[2]^2} \sqrt{1 - z[11]^2} + \\ & \sin[\phi[2] - \phi[17]] \sqrt{3 - 3 z[2]^2} \sqrt{1 - z[11]^2} - \cos[\phi[9] - \phi[11]] \end{aligned}$$

$$\begin{aligned}
& \sqrt{1-z[2]^2} \sqrt{1-z[11]^2} - \text{Cos}[\phi[2] - \phi[17]] \sqrt{1-z[2]^2} \sqrt{1-z[11]^2} + \\
& \text{Sin}[\phi[3] - \phi[11]] \sqrt{3-3z[3]^2} \sqrt{1-z[11]^2} + \text{Sin}[\phi[8] - \phi[17]] \\
& \sqrt{3-3z[3]^2} \sqrt{1-z[11]^2} - \text{Cos}[\phi[3] - \phi[11]] \sqrt{1-z[3]^2} \sqrt{1-z[11]^2} - \\
& \text{Cos}[\phi[8] - \phi[17]] \sqrt{1-z[3]^2} \sqrt{1-z[11]^2} + 4z[1] \times z[12] - 4z[3] \times z[12] + \\
& 4Jc z[3] \times z[12] - 4z[6] \times z[12] + \text{Sin}[\phi[12] - \phi[18]] \sqrt{3-3z[12]^2} - \\
& \text{Sin}[\phi[16] - \phi[18]] \sqrt{3-3z[12]^2} + \text{Cos}[\phi[12] - \phi[18]] \sqrt{1-z[12]^2} - \\
& \text{Cos}[\phi[16] - \phi[18]] \sqrt{1-z[12]^2} + \text{Sin}[\phi[1] - \phi[12]] \sqrt{3-3z[1]^2} \sqrt{1-z[12]^2} + \\
& \text{Sin}[\phi[10] - \phi[16]] \sqrt{3-3z[1]^2} \sqrt{1-z[12]^2} - \text{Cos}[\phi[1] - \phi[12]] \\
& \sqrt{1-z[1]^2} \sqrt{1-z[12]^2} - \text{Cos}[\phi[10] - \phi[16]] \sqrt{1-z[1]^2} \sqrt{1-z[12]^2} + \\
& \text{Sin}[\phi[3] - \phi[12]] \sqrt{3-3z[3]^2} \sqrt{1-z[12]^2} + Jc \text{Sin}[\phi[3] - \phi[12]] \\
& \sqrt{3-3z[3]^2} \sqrt{1-z[12]^2} + Jc \text{Sin}[\phi[8] - \phi[16]] \sqrt{3-3z[3]^2} \sqrt{1-z[12]^2} + \\
& \text{Cos}[\phi[3] - \phi[12]] \sqrt{1-z[3]^2} \sqrt{1-z[12]^2} - Jc \text{Cos}[\phi[3] - \phi[12]] \\
& \sqrt{1-z[3]^2} \sqrt{1-z[12]^2} - 2 \text{Cos}[\phi[8] - \phi[16]] \sqrt{1-z[3]^2} \sqrt{1-z[12]^2} - \\
& Jc \text{Cos}[\phi[8] - \phi[16]] \sqrt{1-z[3]^2} \sqrt{1-z[12]^2} + \text{Sin}[\phi[5] - \phi[12]] \\
& \sqrt{3-3z[6]^2} \sqrt{1-z[12]^2} + \text{Cos}[\phi[5] - \phi[12]] \sqrt{1-z[6]^2} \sqrt{1-z[12]^2} - \\
& 2 \text{Cos}[\phi[5] - \phi[16]] \sqrt{1-z[6]^2} \sqrt{1-z[12]^2} - 4z[2] \times z[13] - 8z[4] \times z[13] - \\
& 4z[5] \times z[13] - 4Jc z[11] \times z[13] + \text{Sin}[\phi[9] - \phi[15]] \sqrt{3-3z[2]^2} \sqrt{1-z[13]^2} - \\
& 2 \text{Cos}[\phi[2] - \phi[13]] \sqrt{1-z[2]^2} \sqrt{1-z[13]^2} + \text{Cos}[\phi[9] - \phi[15]] \\
& \sqrt{1-z[2]^2} \sqrt{1-z[13]^2} + \text{Sin}[\phi[4] - \phi[13]] \sqrt{3-3z[4]^2} \sqrt{1-z[13]^2} + \\
& \text{Sin}[\phi[4] - \phi[15]] \sqrt{3-3z[4]^2} \sqrt{1-z[13]^2} + \text{Cos}[\phi[4] - \phi[13]] \\
& \sqrt{1-z[4]^2} \sqrt{1-z[13]^2} - 2 \text{Cos}[\phi[7] - \phi[13]] \sqrt{1-z[4]^2} \sqrt{1-z[13]^2} + \\
& \text{Cos}[\phi[4] - \phi[15]] \sqrt{1-z[4]^2} \sqrt{1-z[13]^2} - 2 \text{Cos}[\phi[7] - \phi[15]] \\
& \sqrt{1-z[4]^2} \sqrt{1-z[13]^2} + \text{Sin}[\phi[5] - \phi[13]] \sqrt{3-3z[5]^2} \sqrt{1-z[13]^2} + \\
& \text{Cos}[\phi[5] - \phi[13]] \sqrt{1-z[5]^2} \sqrt{1-z[13]^2} - 2 \text{Cos}[\phi[5] - \phi[15]] \sqrt{1-z[5]^2} \\
& \sqrt{1-z[13]^2} - 2Jc \text{Cos}[\phi[11] - \phi[13]] \sqrt{1-z[11]^2} \sqrt{1-z[13]^2} - \\
& 2Jc \text{Cos}[\phi[15] - \phi[17]] \sqrt{1-z[11]^2} \sqrt{1-z[13]^2} - 4z[3] \times z[14] - 2Jp z[5] \times z[14] + \\
& 2Jp z[6] \times z[14] - 4z[11] \times z[14] + \text{Cos}[\phi[8]] \sqrt{3-3z[3]^2} \sqrt{1-z[14]^2} + \\
& 2 \text{Sin}[\phi[3]] \sqrt{1-z[3]^2} \sqrt{1-z[14]^2} - \text{Sin}[\phi[8]] \sqrt{1-z[3]^2} \sqrt{1-z[14]^2} - \\
& Jp \text{Cos}[\phi[5]] \sqrt{3-3z[5]^2} \sqrt{1-z[14]^2} - Jp \text{Sin}[\phi[5]] \sqrt{1-z[5]^2} \sqrt{1-z[14]^2} + \\
& Jp \text{Cos}[\phi[5]] \sqrt{3-3z[6]^2} \sqrt{1-z[14]^2} + Jp \text{Sin}[\phi[5]] \sqrt{1-z[6]^2} \sqrt{1-z[14]^2} + \\
& \text{Cos}[\phi[11]] \sqrt{3-3z[11]^2} \sqrt{1-z[14]^2} - \text{Cos}[\phi[17]] \sqrt{3-3z[11]^2} \sqrt{1-z[14]^2} - \\
& \text{Sin}[\phi[11]] \sqrt{1-z[11]^2} \sqrt{1-z[14]^2} - \text{Sin}[\phi[17]] \sqrt{1-z[11]^2} \sqrt{1-z[14]^2} \Big);
\end{aligned}$$

The plot of the reconstructed ground state clearly shows the  $D_3$  symmetry:

Out[ ]=

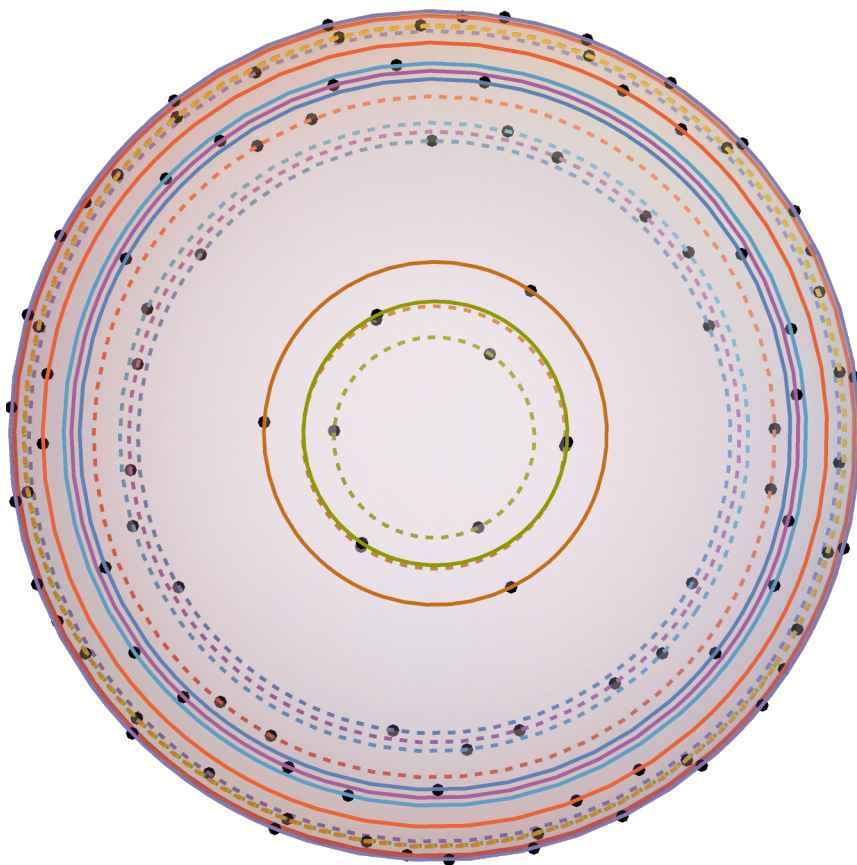

Supplement: Supplementary file 3 [file Spiral_Phases.pdf]
